# Supplementary material for: Learn the Time to Learn: Replay Scheduling in Continual Learning
Source: arXiv:2209.08660 source file (2023-11-20)
Supplement: Supplementary file 1 [file fashionmnist_new_task_order.tex]

\begin{tabular}{lcccccccccc}
\toprule
                 & \multicolumn{2}{c}{\textbf{Test Env. Seed 10}} & \multicolumn{2}{c}{\textbf{Test Env. Seed 11}} & \multicolumn{2}{c}{\textbf{Test Env. Seed 12}} & \multicolumn{2}{c}{\textbf{Test Env. Seed 13}} & \multicolumn{2}{c}{\textbf{Test Env. Seed 14}} \\
\cmidrule(lr){2-3} \cmidrule(lr){4-5} \cmidrule(lr){6-7} \cmidrule(lr){8-9} \cmidrule(lr){10-11}
\textbf{Methods} & $t$                    & $p$                     & $t$                    & $p$                     & $t$                   & $p$                      & $t$                   & $p$                      & $t$                    & $p$                     \\ \midrule
DQN vs Random   & -0.05      & 0.962             & -0.17      & 0.871             & 0.18      & 0.864              & 3.28      & 0.024              & 0.24       & 0.819             \\
DQN vs ETS      & 1.78       & 0.150             & 0.76       & 0.490             & 2.06      & 0.109              & 12.55     & \textbf{0.000}     & 4.19       & \textbf{0.014}    \\
DQN vs Heur-GD  & -3.61      & \textbf{0.023}    & -1.29      & 0.265             & -0.33     & 0.761              & 4.03      & \textbf{0.016}     & -0.85      & 0.445             \\
DQN vs Heur-LD: & -3.61      & \textbf{0.023}    & -1.99      & 0.118             & -1.07     & 0.343              & 1.51      & 0.205              & -0.56      & 0.604             \\
DQN vs Heur-AT  & 13.80      & \textbf{0.000}    & -1.45      & 0.221             & -0.88     & 0.427              & -2.62     & 0.059              & 11.80      & \textbf{0.000}    \\
DQN vs A2C      & -0.61      & 0.574             & 2.26       & 0.084             & 4.35      & \textbf{0.012}     & -1.51     & 0.180              & -0.13      & 0.901             \\
\midrule
A2C vs Random   & 0.09       & 0.934             & -5.96      & \textbf{0.002}    & -2.74     & 0.052              & 3.87      & \textbf{0.016}     & 0.64       & 0.556             \\
A2C vs ETS      & 22.94      & \textbf{0.000}    & -10.13     & \textbf{0.001}    & -inf      & \textbf{0.000}     & 24.85     & \textbf{0.000}     & 81.68      & \textbf{0.000}    \\
A2C vs Heur-GD  & -28.72     & \textbf{0.000}    & -23.78     & \textbf{0.000}    & -inf      & \textbf{0.000}     & 10.04     & \textbf{0.001}     & -13.50     & \textbf{0.000}    \\
A2C vs Heur-LD  & -28.72     & \textbf{0.000}    & -28.38     & \textbf{0.000}    & -inf      & \textbf{0.000}     & 5.65      & \textbf{0.005}     & -8.14      & \textbf{0.001}    \\
A2C vs Heur-AT  & 138.22     & \textbf{0.000}    & -24.81     & \textbf{0.000}    & -inf      & \textbf{0.000}     & -1.54     & 0.199              & 225.61     & \textbf{0.000}    \\
A2C vs DQN      & 0.61       & 0.574             & -2.26      & 0.084             & -4.35     & 0.012              & 1.51      & 0.180              & 0.13       & 0.901             \\
\midrule
                & \multicolumn{2}{c}{Test Env. Seed 15} & \multicolumn{2}{c}{Test Env. Seed 16} & \multicolumn{2}{c}{Test Env. Seed 17} & \multicolumn{2}{c}{Test Env. Seed 18} & \multicolumn{2}{c}{Test Env. Seed 19} \\
\cmidrule(lr){2-3} \cmidrule(lr){4-5} \cmidrule(lr){6-7} \cmidrule(lr){8-9} \cmidrule(lr){10-11}
Methods         & $t$           & $p$                     & $t$           & $p$                     & $t$          & $p$                      & $t$          & $p$                      & $t$           & $p$                     \\
\midrule
DQN vs Random   & -7.48      & \textbf{0.000}    & -1.05      & 0.327             & -1.11     & 0.300              & 3.23      & \textbf{0.028}     & -2.26      & 0.067             \\
DQN vs ETS      & -13.28     & \textbf{0.000}    & -4.06      & \textbf{0.015}    & 4.28      & \textbf{0.013}     & 5.49      & \textbf{0.005}     & -2.31      & 0.082             \\
DQN vs Heur-GD  & 34.42      & \textbf{0.000}    & 12.59      & \textbf{0.000}    & -3.97     & \textbf{0.017}     & 7.21      & \textbf{0.002}     & -0.34      & 0.752             \\
DQN vs Heur-LD: & -10.25     & \textbf{0.001}    & 7.27       & \textbf{0.002}    & -3.64     & \textbf{0.022}     & 9.52      & \textbf{0.001}     & 2.41       & 0.073             \\
DQN vs Heur-AT  & 3.44       & \textbf{0.026}    & 0.12       & 0.912             & 0.16      & 0.883              & 3.72      & \textbf{0.021}     & -1.24      & 0.281             \\
DQN vs A2C      & 27.78      & \textbf{0.000}    & 2.23       & 0.056             & -0.64     & 0.540              & 3.54      & \textbf{0.010}     & -1.79      & 0.143             \\
\midrule
A2C vs Random   & -26.79     & \textbf{0.000}    & -3.58      & \textbf{0.010}    & -0.50     & 0.634              & 2.39      & 0.073              & -1.34      & 0.235             \\
A2C vs ETS      & -109.10    & \textbf{0.000}    & -6.83      & \textbf{0.002}    & 5.87      & \textbf{0.004}     & 2.18      & 0.094              & -2.52      & 0.066             \\
A2C vs Heur-GD  & 11.50      & \textbf{0.000}    & 8.66       & \textbf{0.001}    & -3.56     & \textbf{0.024}     & 4.99      & \textbf{0.008}     & 7.67       & \textbf{0.002}    \\
A2C vs Heur-LD  & -101.45    & \textbf{0.000}    & 3.71       & \textbf{0.021}    & -3.19     & \textbf{0.033}     & 8.76      & \textbf{0.001}     & 21.88      & \textbf{0.000}    \\
A2C vs Heur-AT  & -66.83     & \textbf{0.000}    & -2.94      & \textbf{0.042}    & 1.15      & 0.313              & -0.71     & 0.517              & 3.00       & \textbf{0.040}    \\
A2C vs DQN      & -27.78     & \textbf{0.000}    & -2.23      & 0.056             & 0.64      & 0.540              & -3.54     & 0.010              & 1.79       & 0.143  \\
\bottomrule
\end{tabular}
