# Supplementary material for: Learn the Time to Learn: Replay Scheduling in Continual Learning
Source: arXiv:2209.08660 source file (2023-11-20)
Supplement: Supplementary file 2 [file results_fashionmnist_new_dataset.tex]

\begin{tabular}{lcccccc}
\toprule
                & \multicolumn{3}{c}{\textbf{Test Env. Seed 0}} & \multicolumn{3}{c}{\textbf{Test Env. Seed 1}} \\
\cmidrule(lr){2-4} \cmidrule(lr){5-7}
\textbf{Method} & ACC (\%)         & BWT (\%)          & Rank   & ACC (\%)         & BWT (\%)          & Rank   \\
\midrule
Random          & 94.33 $\pm$ 3.03   & -6.15 $\pm$ 3.78    & 5.4    & 92.26 $\pm$ 3.84   & -5.96 $\pm$ 4.78    & 4.2    \\
ETS             & 97.10 $\pm$ 0.00   & -2.70 $\pm$ 0.00    & 5.8    & 94.10 $\pm$ 0.00   & -3.59 $\pm$ 0.00    & 3.2    \\
Heur-GD         & 97.90 $\pm$ 0.00   & -1.59 $\pm$ 0.00    & 1      & 95.01 $\pm$ 0.00   & -2.69 $\pm$ 0.00    & 1.4    \\
Heur-LD         & 97.59 $\pm$ 0.00   & -1.99 $\pm$ 0.00    & 3      & 90.03 $\pm$ 0.00   & -8.90 $\pm$ 0.00    & 6.8    \\
Heur-AT         & 97.41 $\pm$ 0.00   & -2.21 $\pm$ 0.00    & 4.6    & 94.09 $\pm$ 0.00   & -3.78 $\pm$ 0.00    & 4.2    \\
DQN             & 96.82 $\pm$ 1.50   & -3.06 $\pm$ 1.87    & 3.8    & 93.74 $\pm$ 1.86   & -4.24 $\pm$ 2.33    & 3.2    \\
A2C             & 95.74 $\pm$ 3.33   & -4.39 $\pm$ 4.15    & 4.4    & 92.80 $\pm$ 1.56   & -5.27 $\pm$ 1.95    & 5      \\
\midrule
                & \multicolumn{3}{c}{\textbf{Test Env. Seed 2}} & \multicolumn{3}{c}{\textbf{Test Env. Seed 3}} \\
\cmidrule(lr){2-4} \cmidrule(lr){5-7}
\textbf{Method} & ACC (\%)         & BWT (\%)          & Rank   & ACC (\%)         & BWT (\%)          & Rank   \\
\midrule
Random          & 93.74 $\pm$ 2.97   & -6.36 $\pm$ 3.71    & 5.8    & 94.12 $\pm$ 4.14   & -6.99 $\pm$ 5.16    & 3.9    \\
ETS             & 86.72 $\pm$ 0.00   & -15.17 $\pm$ 0.00   & 7      & 89.44 $\pm$ 0.00   & -12.86 $\pm$ 0.00   & 6.4    \\
Heur-GD         & 97.41 $\pm$ 0.00   & -1.87 $\pm$ 0.00    & 2.8    & 96.69 $\pm$ 0.00   & -3.68 $\pm$ 0.00    & 3      \\
Heur-LD         & 97.30 $\pm$ 0.00   & -1.91 $\pm$ 0.00    & 3.8    & 90.61 $\pm$ 0.00   & -11.26 $\pm$ 0.00   & 4.8    \\
Heur-AT         & 97.65 $\pm$ 0.00   & -1.58 $\pm$ 0.00    & 1      & 99.40 $\pm$ 0.00   & -0.26 $\pm$ 0.00    & 1.1    \\
DQN             & 96.13 $\pm$ 0.97   & -3.47 $\pm$ 1.20    & 5      & 94.66 $\pm$ 5.00   & -6.24 $\pm$ 6.26    & 3.6    \\
A2C             & 97.31 $\pm$ 0.55   & -1.99 $\pm$ 0.71    & 2.6    & 92.12 $\pm$ 3.75   & -9.40 $\pm$ 4.68    & 5.2    \\
\midrule
                & \multicolumn{3}{c}{\textbf{Test Env. Seed 4}} & \multicolumn{3}{c}{\textbf{Test Env. Seed 5}} \\
\cmidrule(lr){2-4} \cmidrule(lr){5-7}
\textbf{Method} & ACC (\%)         & BWT (\%)          & Rank   & ACC (\%)         & BWT (\%)          & Rank   \\
\midrule
Random          & 83.64 $\pm$ 5.22   & -16.86 $\pm$ 6.48   & 5.4    & 89.76 $\pm$ 2.46   & -7.91 $\pm$ 3.06    & 4      \\
ETS             & 87.07 $\pm$ 0.00   & -12.61 $\pm$ 0.00   & 4.2    & 91.53 $\pm$ 0.00   & -5.61 $\pm$ 0.00    & 1.2    \\
Heur-GD         & 91.29 $\pm$ 0.00   & -7.30 $\pm$ 0.00    & 2.4    & 90.33 $\pm$ 0.00   & -7.25 $\pm$ 0.00    & 3.4    \\
Heur-LD         & 86.75 $\pm$ 0.00   & -12.87 $\pm$ 0.00   & 5.2    & 88.01 $\pm$ 0.00   & -10.02 $\pm$ 0.00   & 4.8    \\
Heur-AT         & 83.28 $\pm$ 0.00   & -17.02 $\pm$ 0.00   & 6.4    & 90.53 $\pm$ 0.00   & -6.81 $\pm$ 0.00    & 2.4    \\
DQN             & 88.76 $\pm$ 4.73   & -10.37 $\pm$ 5.95   & 3.2    & 87.31 $\pm$ 1.09   & -10.89 $\pm$ 1.38   & 6.2    \\
A2C             & 91.98 $\pm$ 0.17   & -6.36 $\pm$ 0.18    & 1.2    & 87.93 $\pm$ 0.00   & -10.07 $\pm$ 0.00   & 6      \\
\midrule
                & \multicolumn{3}{c}{\textbf{Test Env. Seed 6}} & \multicolumn{3}{c}{\textbf{Test Env. Seed 7}} \\
\cmidrule(lr){2-4} \cmidrule(lr){5-7}
\textbf{Method} & ACC (\%)         & BWT (\%)          & Rank   & ACC (\%)         & BWT (\%)          & Rank   \\
\midrule
Random          & 95.34 $\pm$ 0.74   & -2.57 $\pm$ 1.01    & 1.4    & 94.40 $\pm$ 0.77   & -3.53 $\pm$ 0.94    & 4      \\
ETS             & 95.48 $\pm$ 0.00   & -2.50 $\pm$ 0.00    & 1.6    & 95.31 $\pm$ 0.00   & -2.21 $\pm$ 0.00    & 2.6    \\
Heur-GD         & 90.01 $\pm$ 0.00   & -9.09 $\pm$ 0.00    & 4.2    & 91.76 $\pm$ 0.00   & -6.84 $\pm$ 0.00    & 5.6    \\
Heur-LD         & 85.44 $\pm$ 0.00   & -14.96 $\pm$ 0.00   & 5.2    & 95.14 $\pm$ 0.00   & -2.64 $\pm$ 0.00    & 3.6    \\
Heur-AT         & 76.02 $\pm$ 0.00   & -26.58 $\pm$ 0.00   & 7      & 96.78 $\pm$ 0.00   & -0.67 $\pm$ 0.00    & 1.2    \\
DQN             & 86.60 $\pm$ 5.92   & -13.56 $\pm$ 7.39   & 4.8    & 89.22 $\pm$ 2.34   & -10.06 $\pm$ 2.88   & 6.8    \\
A2C             & 89.14 $\pm$ 3.66   & -10.35 $\pm$ 4.57   & 3.8    & 93.49 $\pm$ 2.58   & -4.77 $\pm$ 3.18    & 4.2    \\
\midrule
                & \multicolumn{3}{c}{\textbf{Test Env. Seed 8}} & \multicolumn{3}{c}{\textbf{Test Env. Seed 9}} \\
\cmidrule(lr){2-4} \cmidrule(lr){5-7}
\textbf{Method} & ACC (\%)         & BWT (\%)          & Rank   & ACC (\%)         & BWT (\%)          & Rank   \\
\midrule
Random          & 93.15 $\pm$ 4.08   & -7.22 $\pm$ 5.09    & 3      & 94.81 $\pm$ 3.66   & -5.14 $\pm$ 4.51    & 2.8    \\
ETS             & 94.80 $\pm$ 0.00   & -5.18 $\pm$ 0.00    & 2.8    & 96.71 $\pm$ 0.00   & -2.76 $\pm$ 0.00    & 2      \\
Heur-GD         & 95.00 $\pm$ 0.00   & -4.83 $\pm$ 0.00    & 1.6    & 95.27 $\pm$ 0.00   & -4.75 $\pm$ 0.00    & 3.2    \\
Heur-LD         & 87.86 $\pm$ 0.00   & -13.66 $\pm$ 0.00   & 6.8    & 90.02 $\pm$ 0.00   & -11.16 $\pm$ 0.00   & 6.8    \\
Heur-AT         & 93.93 $\pm$ 0.00   & -6.07 $\pm$ 0.00    & 3.8    & 90.29 $\pm$ 0.00   & -10.82 $\pm$ 0.00   & 5.8    \\
DQN             & 91.67 $\pm$ 2.85   & -8.94 $\pm$ 3.61    & 5      & 95.32 $\pm$ 1.76   & -4.60 $\pm$ 2.19    & 2.6    \\
A2C             & 93.57 $\pm$ 0.00   & -6.61 $\pm$ 0.00    & 5      & 91.31 $\pm$ 1.08   & -9.62 $\pm$ 1.37    & 4.8   \\
\bottomrule
\end{tabular}
