# Supplementary material for: Learn the Time to Learn: Replay Scheduling in Continual Learning
Source: arXiv:2209.08660 source file (2023-11-20)
Supplement: Supplementary file 3 [file results_fashionmnist_new_task_order.tex]

\begin{tabular}{lcccccc}
\toprule
                & \multicolumn{3}{c}{\textbf{Test Env. Seed 10}} & \multicolumn{3}{c}{\textbf{Test Env. Seed 11}} \\
\cmidrule(lr){2-4} \cmidrule(lr){5-7}
\textbf{Method} & ACC (\%)          & BWT (\%)          & Rank   & ACC (\%)          & BWT (\%)          & Rank   \\
\midrule
Random          & 96.79 $\pm$ 3.02    & -3.11 $\pm$ 3.76    & 2.2    & 90.84 $\pm$ 1.64    & -8.02 $\pm$ 2.04    & 4.4    \\
ETS             & 96.10 $\pm$ 0.00    & -3.98 $\pm$ 0.00    & 5.6    & 88.84 $\pm$ 0.00    & -10.55 $\pm$ 0.00   & 5.8    \\
Heur-GD         & 97.96 $\pm$ 0.00    & -1.93 $\pm$ 0.00    & 2.3    & 93.21 $\pm$ 0.00    & -4.96 $\pm$ 0.00    & 3.4    \\
Heur-LD         & 97.96 $\pm$ 0.00    & -1.93 $\pm$ 0.00    & 2.3    & 94.68 $\pm$ 0.00    & -3.12 $\pm$ 0.00    & 1      \\
Heur-AT         & 91.95 $\pm$ 0.00    & -9.30 $\pm$ 0.00    & 6.8    & 93.54 $\pm$ 0.00    & -4.70 $\pm$ 0.00    & 2      \\
DQN             & 96.71 $\pm$ 0.69    & -3.47 $\pm$ 0.86    & 4.5    & 90.46 $\pm$ 4.25    & -8.60 $\pm$ 5.32    & 4.6    \\
A2C             & 96.93 $\pm$ 0.07    & -3.20 $\pm$ 0.09    & 4.3    & 85.60 $\pm$ 0.64    & -14.65 $\pm$ 0.79   & 6.8    \\ 
\midrule
                & \multicolumn{3}{c}{\textbf{Test Env. Seed 12}} & \multicolumn{3}{c}{\textbf{Test Env. Seed 13}} \\
\cmidrule(lr){2-4} \cmidrule(lr){5-7}
\textbf{Method} & ACC (\%)          & BWT (\%)          & Rank   & ACC (\%)          & BWT (\%)          & Rank   \\
\midrule
Random          & 93.97 $\pm$ 4.60    & -6.60 $\pm$ 5.74    & 2.8    & 91.66 $\pm$ 3.08    & -9.38 $\pm$ 3.85    & 6.4    \\
ETS             & 91.25 $\pm$ 0.00    & -10.08 $\pm$ 0.00   & 5.6    & 91.24 $\pm$ 0.00    & -9.85 $\pm$ 0.00    & 6.6    \\
Heur-GD         & 94.97 $\pm$ 0.00    & -5.26 $\pm$ 0.00    & 4.2    & 95.09 $\pm$ 0.00    & -5.10 $\pm$ 0.00    & 5      \\
Heur-LD         & 96.14 $\pm$ 0.00    & -3.89 $\pm$ 0.00    & 1.8    & 96.23 $\pm$ 0.00    & -3.69 $\pm$ 0.00    & 3.8    \\
Heur-AT         & 95.84 $\pm$ 0.00    & -4.21 $\pm$ 0.00    & 3      & 98.10 $\pm$ 0.00    & -1.38 $\pm$ 0.00    & 1.2    \\
DQN             & 94.46 $\pm$ 3.12    & -6.00 $\pm$ 3.95    & 3.8    & 96.91 $\pm$ 0.90    & -2.83 $\pm$ 1.12    & 2.6    \\
A2C             & 87.67 $\pm$ 0.00    & -14.49 $\pm$ 0.00   & 6.8    & 97.70 $\pm$ 0.52    & -1.87 $\pm$ 0.67    & 2.4    \\
\midrule
                & \multicolumn{3}{c}{\textbf{Test Env. Seed 14}} & \multicolumn{3}{c}{\textbf{Test Env. Seed 15}} \\
\cmidrule(lr){2-4} \cmidrule(lr){5-7}
\textbf{Method} & ACC (\%)          & BWT (\%)          & Rank   & ACC (\%)          & BWT (\%)          & Rank   \\
\midrule
Random          & 94.17 $\pm$ 1.37    & -3.79 $\pm$ 1.73    & 3.6    & 93.74 $\pm$ 0.95    & -4.53 $\pm$ 1.18    & 1.4    \\
ETS             & 90.04 $\pm$ 0.00    & -8.92 $\pm$ 0.00    & 6      & 93.51 $\pm$ 0.00    & -4.81 $\pm$ 0.00    & 1.6    \\
Heur-GD         & 95.37 $\pm$ 0.00    & -2.26 $\pm$ 0.00    & 1.6    & 79.33 $\pm$ 0.00    & -22.05 $\pm$ 0.00   & 7      \\
Heur-LD         & 95.07 $\pm$ 0.00    & -2.65 $\pm$ 0.00    & 3.2    & 92.61 $\pm$ 0.00    & -5.44 $\pm$ 0.00    & 3      \\
Heur-AT         & 81.98 $\pm$ 0.00    & -18.88 $\pm$ 0.00   & 7      & 88.54 $\pm$ 0.00    & -10.50 $\pm$ 0.00   & 4.8    \\
DQN             & 94.47 $\pm$ 2.12    & -3.12 $\pm$ 2.66    & 2.4    & 89.56 $\pm$ 0.59    & -9.25 $\pm$ 0.74    & 4.2    \\
A2C             & 94.61 $\pm$ 0.11    & -2.96 $\pm$ 0.14    & 4.2    & 80.68 $\pm$ 0.24    & -20.34 $\pm$ 0.29   & 6      \\
\midrule
                & \multicolumn{3}{c}{\textbf{Test Env. Seed 16}} & \multicolumn{3}{c}{\textbf{Test Env. Seed 17}} \\
\cmidrule(lr){2-4} \cmidrule(lr){5-7}
\textbf{Method} & ACC (\%)          & BWT (\%)          & Rank   & ACC (\%)          & BWT (\%)          & Rank   \\
\midrule
Random          & 90.96 $\pm$ 1.68    & -7.18 $\pm$ 2.06    & 2.4    & 98.99 $\pm$ 0.26    & -0.66 $\pm$ 0.34    & 3.8    \\
ETS             & 94.41 $\pm$ 0.00    & -2.96 $\pm$ 0.00    & 1      & 98.11 $\pm$ 0.00    & -1.77 $\pm$ 0.00    & 7      \\
Heur-GD         & 73.82 $\pm$ 0.00    & -28.91 $\pm$ 0.00   & 7      & 99.37 $\pm$ 0.00    & -0.24 $\pm$ 0.00    & 1      \\
Heur-LD         & 80.40 $\pm$ 0.00    & -20.66 $\pm$ 0.00   & 6      & 99.32 $\pm$ 0.00    & -0.30 $\pm$ 0.00    & 2      \\
Heur-AT         & 89.24 $\pm$ 0.00    & -9.68 $\pm$ 0.00    & 3.6    & 98.74 $\pm$ 0.00    & -0.99 $\pm$ 0.00    & 4.8    \\
DQN             & 89.39 $\pm$ 2.47    & -9.49 $\pm$ 3.09    & 3.4    & 98.76 $\pm$ 0.31    & -0.97 $\pm$ 0.38    & 5      \\
A2C             & 85.33 $\pm$ 2.66    & -14.62 $\pm$ 3.36   & 4.6    & 98.89 $\pm$ 0.27    & -0.80 $\pm$ 0.33    & 4.4    \\
\midrule
                & \multicolumn{3}{c}{\textbf{Test Env. Seed 18}} & \multicolumn{3}{c}{\textbf{Test Env. Seed 19}} \\
\cmidrule(lr){2-4} \cmidrule(lr){5-7}
\textbf{Method} & ACC (\%)          & BWT (\%)          & Rank   & ACC (\%)          & BWT (\%)          & Rank   \\
\midrule
Random          & 89.92 $\pm$ 3.44    & -11.26 $\pm$ 4.30   & 5.6    & 97.64 $\pm$ 0.79    & -1.58 $\pm$ 1.06    & 1.8    \\
ETS             & 93.56 $\pm$ 0.00    & -6.74 $\pm$ 0.00    & 4.4    & 97.49 $\pm$ 0.00    & -1.81 $\pm$ 0.00    & 2      \\
Heur-GD         & 92.92 $\pm$ 0.00    & -7.31 $\pm$ 0.00    & 5.4    & 95.79 $\pm$ 0.00    & -3.94 $\pm$ 0.00    & 5.4    \\
Heur-LD         & 92.06 $\pm$ 0.00    & -8.40 $\pm$ 0.00    & 6.4    & 93.42 $\pm$ 0.00    & -6.85 $\pm$ 0.00    & 6.8    \\
Heur-AT         & 94.22 $\pm$ 0.00    & -5.66 $\pm$ 0.00    & 2.2    & 96.57 $\pm$ 0.00    & -3.01 $\pm$ 0.00    & 4.2    \\
DQN             & 95.60 $\pm$ 0.74    & -3.92 $\pm$ 0.93    & 1      & 95.50 $\pm$ 1.72    & -4.42 $\pm$ 2.16    & 5      \\
A2C             & 94.06 $\pm$ 0.46    & -5.88 $\pm$ 0.58    & 3      & 97.07 $\pm$ 0.33    & -2.41 $\pm$ 0.40    & 2.8   \\
\bottomrule
\end{tabular}
