# Supplementary material for: Learn the Time to Learn: Replay Scheduling in Continual Learning
Source: arXiv:2209.08660 source file (2023-11-20)
Supplement: Supplementary file 4 [file bubble_plot.tex]

\nextgroupplot[title={Replay Schedule},
height=\figheight,
minor xtick={},
minor ytick={},
tick align=outside,
tick pos=left,
width=\figwidth,
x grid style={white!69.0196078431373!black},
grid=major,
xlabel={Current Task},
xmin=1.5, xmax=5.5,
xtick style={color=black},
xtick={2,3,4,5},
xticklabels={2,3,4,5},
xticklabel style = {font=\tiny},
y grid style={white!69.0196078431373!black},
ylabel={Replayed Task},
%ylabel style={at={(0.5,0.0)},
ymin=0.45, ymax=4.5,
ytick style={color=black},
ytick={1,2,3,4},
yticklabels={1,2,3,4},
yticklabel style = {font=\tiny},
]
\addplot+[
mark=*,
only marks,
scatter,
scatter src=explicit,
scatter/@pre marker code/.code={%
  \expanded{%
    \noexpand\definecolor{thispointdrawcolor}{RGB}{\drawcolor}%
    \noexpand\definecolor{thispointfillcolor}{RGB}{\fillcolor}%
  }%
  \scope[draw=thispointdrawcolor, fill=thispointfillcolor]%
},
visualization depends on={\thisrow{sizedata}/5 \as \perpointmarksize},
visualization depends on={value \thisrow{draw} \as \drawcolor},
visualization depends on={value \thisrow{fill} \as \fillcolor},
%visualization depends on=
%{5*cos(deg(x)) \as \perpointmarksize},
scatter/@pre marker code/.append style=
{/tikz/mark size=\perpointmarksize}
]
table[x=x, y=y, meta=sizedata]{
x  y  draw  fill  sizedata
2 1 31,119,180 31,119,180 17.841241161527712
3 1 31,119,180 31,119,180 0.0
4 1 31,119,180 31,119,180 0.0
5 1 31,119,180 31,119,180 0.0

3 2 255,127,14 255,127,14 17.841241161527712
4 2 255,127,14 255,127,14 17.841241161527712
5 2 255,127,14 255,127,14 12.6156626101008

4 3 44,160,44 44,160,44 0.0
5 3 44,160,44 44,160,44 12.6156626101008

};
