# Supplementary material for: Learn the Time to Learn: Replay Scheduling in Continual Learning
Source: arXiv:2209.08660 source file (2023-11-20)
Supplement: Supplementary file 6 [file finetune.tex]

\nextgroupplot[title=Fine-tuning (ACC: 89.84\%),
height=\figheight,
legend cell align={left},
legend style={
  nodes={scale=0.8},
  fill opacity=0.8,
  draw opacity=1,
  text opacity=1,
  at={(5.32,0.02)},
  anchor=south west,
  draw=white!80!black
},
minor xtick={},
minor ytick={0.55,0.65,0.75,0.85,0.95,1.05},
tick align=outside,
tick pos=left,
width=\figwidth,
x grid style={white!69.0196078431373!black},
xmajorgrids,
xlabel={Task},
xmin=0.8, xmax=5.2,
xtick style={color=black},
xtick={1,2,3,4,5},
xticklabels={1,2,3,4,5},
y grid style={white!69.0196078431373!black},
ymajorgrids,
yminorgrids,
ylabel={Accuracy},
ymin=0.491, ymax=1.01,
ytick style={color=black},
ytick={0.5,0.6,0.7,0.8,0.9,1.0},
yticklabels={50, 60, 70, 80, 90, 100}
]
\addplot [line width=1.5pt, color0, mark=*, mark size=1.5, mark options={solid}]
table {%
1 0.999527215957642
2 0.994799077510834
3 0.652009427547455
4 0.552718698978424
5 0.712529540061951
};\addlegendentry{Task 1}
\addplot [line width=1.5pt, color1, mark=*, mark size=1.5, mark options={solid}]
table {%
2 0.996572017669678
3 0.974045038223267
4 0.952987253665924
5 0.81292849779129
};\addlegendentry{Task 2}
\addplot [line width=1.5pt, color2, mark=*, mark size=1.5, mark options={solid}]
table {%
3 0.997865557670593
4 0.954642474651337
5 0.97438633441925
};\addlegendentry{Task 3}
\addplot [line width=1.5pt, color3, mark=*, mark size=1.5, mark options={solid}]
table {%
4 0.998489439487457
5 0.996475338935852
};\addlegendentry{Task 4}
\addplot [line width=1.5pt, color4, mark=*, mark size=1.5, mark options={solid}]
table {%
5 0.995461404323578
};\addlegendentry{Task 5}
