# Supplementary material for: Learn the Time to Learn: Replay Scheduling in Continual Learning
Source: arXiv:2209.08660 source file (2023-11-20)
Supplement: Supplementary file 7 [file rs_mcts.tex]

\nextgroupplot[title=MCTS (ACC: 98.24\%),
height=\figheight,
legend cell align={left},
legend style={
  nodes={scale=0.9},
  fill opacity=0.8,
  draw opacity=1,
  text opacity=1,
  at={(3.72,0.28)},
  anchor=south west,
  draw=white!80!black
},
minor xtick={},
minor ytick={0.55,0.65,0.75,0.85,0.95,1.05},
tick align=outside,
tick pos=left,
width=\figwidth,
x grid style={white!69.0196078431373!black},
xmajorgrids,
xlabel={Task},
xmin=0.8, xmax=5.2,
xtick style={color=black},
xtick={1,2,3,4,5},
xticklabels={1,2,3,4,5},
y grid style={white!69.0196078431373!black},
ymajorgrids,
yminorgrids,
ylabel={Accuracy},
ymin=0.491, ymax=1.01,
ytick style={color=black},
ytick={0.5,0.6,0.7,0.8,0.9,1.0},
yticklabels={50, 60, 70, 80, 90, 100}
]
\addplot [line width=1.5pt, color0, mark=*, mark size=1.5, mark options={solid}]
table {%
1 0.999527215957642
2 0.99858158826828
3 0.999527215957642
4 0.996690332889557
5 0.998108744621277
};
\addplot [line width=1.5pt, color1, mark=*, mark size=1.5, mark options={solid}]
table {%
2 0.994613111019135
3 0.961312413215637
4 0.946131229400635
5 0.953476965427399
};
\addplot [line width=1.5pt, color2, mark=*, mark size=1.5, mark options={solid}]
table {%
3 0.998399138450623
4 0.961579501628876
5 0.978655278682709
};
\addplot [line width=1.5pt, color3, mark=*, mark size=1.5, mark options={solid}]
table {%
4 0.99899297952652
5 0.994461238384247
};
\addplot [line width=1.5pt, color4, mark=*, mark size=1.5, mark options={solid}]
table {%
5 0.992435693740845
};
