# Supplementary material for: Learn the Time to Learn: Replay Scheduling in Continual Learning
Source: arXiv:2209.08660 source file (2023-11-20)
Supplement: Supplementary file 8 [file CIFAR100_rewards.tex]

\nextgroupplot[title=S-CIFAR-100,
height=\figheight,
minor xtick={25, 75},
minor ytick={0.48, 0.52, 0.56},
tick align=outside,
tick pos=left,
width=\figwidth,
x grid style={white!69.0196078431373!black},
xlabel={Iteration},
xmajorgrids,
xminorgrids,
xmin=0, xmax=101,
xtick style={color=black},
xtick={-25,0,50,100,125},%xtick={-25,0,25,50,75,100,125},
xticklabels={-25,0,50,100,125},%xticklabels={-25,0,25,50,75,100,125},
y grid style={white!69.0196078431373!black},
ymajorgrids,
yminorgrids,
ymin=0.472152, ymax=0.581,
ytick style={color=black},
ytick={0.46, 0.5, 0.54, 0.58},
yticklabels={0.46, 50, 54, 58}
]
\addplot [line width=1.5pt, color0]
table {%
1 0.539879977703094
100 0.539879977703094
};

\addplot [line width=1.5pt, color1, style={dashed}]
table {%
1 0.47696
100 0.47696
};

\addplot [line width=1.5pt, color2, style={dashdotted}]
table {%
1 0.57312
100 0.57312
};

\addplot [line width=1.5pt, color3]
table {%
1 0.539879977703094
2 0.543919920921326
3 0.555779993534088
4 0.555899977684021
5 0.555899977684021
6 0.555899977684021
7 0.555899977684021
8 0.560000002384186
9 0.563799977302551
10 0.563799977302551
11 0.563799977302551
12 0.563799977302551
13 0.563799977302551
14 0.563799977302551
15 0.563799977302551
16 0.563799977302551
17 0.563799977302551
18 0.563799977302551
19 0.563799977302551
20 0.563459992408752
21 0.563459992408752
22 0.563459992408752
23 0.563459992408752
24 0.563459992408752
25 0.563459992408752
26 0.563459992408752
27 0.563459992408752
28 0.563459992408752
29 0.563459992408752
30 0.563459992408752
31 0.563459992408752
32 0.563459992408752
33 0.563459992408752
34 0.563459992408752
35 0.563459992408752
36 0.563459992408752
37 0.563459992408752
38 0.563459992408752
39 0.563459992408752
40 0.563459992408752
41 0.563459992408752
42 0.56497997045517
43 0.56497997045517
44 0.56497997045517
45 0.565619945526123
46 0.565619945526123
47 0.565619945526123
48 0.565619945526123
49 0.565619945526123
50 0.565619945526123
51 0.567999958992004
52 0.567999958992004
53 0.567999958992004
54 0.567999958992004
55 0.567999958992004
56 0.567999958992004
57 0.567999958992004
58 0.567999958992004
59 0.567999958992004
60 0.567999958992004
61 0.567999958992004
62 0.567999958992004
63 0.567999958992004
64 0.567999958992004
65 0.567999958992004
66 0.567999958992004
67 0.567999958992004
68 0.567999958992004
69 0.567999958992004
70 0.567999958992004
71 0.567999958992004
72 0.566319942474365
73 0.566319942474365
74 0.566319942474365
75 0.565959930419922
76 0.565959930419922
77 0.565959930419922
78 0.565959930419922
79 0.565959930419922
80 0.565959930419922
81 0.565959930419922
82 0.565959930419922
83 0.565959930419922
84 0.565959930419922
85 0.565959930419922
86 0.565959930419922
87 0.565959930419922
88 0.565959930419922
89 0.565959930419922
90 0.565959930419922
91 0.565959930419922
92 0.565959930419922
93 0.565959930419922
94 0.565959930419922
95 0.565959930419922
96 0.565959930419922
97 0.565959930419922
98 0.565959930419922
99 0.565959930419922
100 0.565959930419922
};
