# Supplementary material for: Learn the Time to Learn: Replay Scheduling in Continual Learning
Source: arXiv:2209.08660 source file (2023-11-20)
Supplement: Supplementary file 9 [file FashionMNIST_rewards.tex]

\nextgroupplot[title=S-FashionMNIST,
height=\figheight,
minor xtick={25, 75},
minor ytick={},
tick align=outside,
tick pos=left,
width=\figwidth,
x grid style={white!69.0196078431373!black},
xlabel={Iteration},
xmajorgrids,
xminorgrids,
xmin=0, xmax=101,
xtick style={color=black},
xtick={-25,0,50,100,125},%xtick={-25,0,25,50,75,100,125},
xticklabels={-25,0,50,100,125},%xticklabels={-25,0,25,50,75,100,125},
y grid style={white!69.0196078431373!black},
ymajorgrids,
ymin=0.955, ymax=1.0, %ymax=0.991,
ytick style={color=black},
ytick={0.92,0.94,0.96,0.97,0.98,0.99,1.0},
yticklabels={92,94,96,97,98,99,100},
]
\addplot [line width=1.5pt, color0]
table {%
1 0.9582200050354
100 0.9582200050354
};
%\addlegendentry{Random}
\addplot [line width=1.5pt, color1, style={dashed}]
table {%
1 0.95814
100 0.95814
};
%\addlegendentry{ETS}
\addplot [line width=1.5pt, color2, style={dashdotted}]
table {%
1 0.97094
100 0.97094
};
%\addlegendentry{Heur}
\addplot [line width=1.5pt, color3]
table {%
1 0.9582200050354
2 0.969580054283142
3 0.970239996910095
4 0.970239996910095
5 0.972180008888245
6 0.972180008888245
7 0.972780048847198
8 0.97382003068924
9 0.97382003068924
10 0.97382003068924
11 0.97382003068924
12 0.97382003068924
13 0.974880039691925
14 0.975259959697723
15 0.975259959697723
16 0.975259959697723
17 0.975259959697723
18 0.977100014686584
19 0.977100014686584
20 0.977800011634827
21 0.977800011634827
22 0.977800011634827
23 0.978839993476868
24 0.978839993476868
25 0.978839993476868
26 0.978960037231445
27 0.978960037231445
28 0.978960037231445
29 0.9792799949646
30 0.9792799949646
31 0.9792799949646
32 0.979800045490265
33 0.980080008506775
34 0.980080008506775
35 0.980080008506775
36 0.98089998960495
37 0.98089998960495
38 0.98089998960495
39 0.98089998960495
40 0.98089998960495
41 0.98089998960495
42 0.98089998960495
43 0.98089998960495
44 0.98089998960495
45 0.98089998960495
46 0.98089998960495
47 0.98089998960495
48 0.98089998960495
49 0.98089998960495
50 0.98089998960495
51 0.98089998960495
52 0.98089998960495
53 0.98089998960495
54 0.98089998960495
55 0.98089998960495
56 0.98089998960495
57 0.98089998960495
58 0.982640087604523
59 0.982640087604523
60 0.982640087604523
61 0.982640087604523
62 0.982640087604523
63 0.982640087604523
64 0.982640087604523
65 0.982640087604523
66 0.982640087604523
67 0.982920050621033
68 0.982920050621033
69 0.982920050621033
70 0.982920050621033
71 0.982920050621033
72 0.982920050621033
73 0.982800006866455
74 0.982800006866455
75 0.982639968395233
76 0.982639968395233
77 0.982639968395233
78 0.982639968395233
79 0.982639968395233
80 0.982639968395233
81 0.982639968395233
82 0.982639968395233
83 0.982639968395233
84 0.982639968395233
85 0.982639968395233
86 0.982639968395233
87 0.982620060443878
88 0.982620060443878
89 0.982620060443878
90 0.982620060443878
91 0.982620060443878
92 0.982620060443878
93 0.982620060443878
94 0.982620060443878
95 0.982620060443878
96 0.982620060443878
97 0.982620060443878
98 0.982740044593811
99 0.982740044593811
100 0.982740044593811
};
%\addlegendentry{RS-MCTS}
\addplot [line width=1.5pt, color4]
table {%
1 0.98508
100 0.98508
};
%\addlegendentry{BFS}
\addplot [line width=1.5pt, color5]
table {%
1 0.99336
100 0.99336
};
%\addlegendentry{Joint}
