# Supplementary material for: Learn the Time to Learn: Replay Scheduling in Continual Learning
Source: arXiv:2209.08660 source file (2023-11-20)
Supplement: Supplementary file 10 [file MNIST_rewards.tex]

\nextgroupplot[title=S-MNIST,
height=\figheight,
legend cell align={left},
legend columns=1,
legend style={
  nodes={scale=0.95},%{scale=0.8},
  fill opacity=0.8,
  draw opacity=1,
  text opacity=1,
  at={(4.20,-0.35)},%{(8.15,-0.05)},
  anchor=south west,
  draw=white!80!black
},
minor xtick={25, 75},
minor ytick={0.95, 0.97, 0.99},
tick align=outside,
tick pos=left,
width=\figwidth,
x grid style={white!69.0196078431373!black},
xlabel={Iteration},
xmajorgrids,
xminorgrids,
xmin=0, xmax=101,
xtick style={color=black},
xtick={-25,0,50,100,125},%xtick={-25,0,25,50,75,100,125},
xticklabels={-25,0,50,100,125},%xticklabels={-25,0,25,50,75,100,125},
y grid style={white!69.0196078431373!black},
ylabel={ACC (\%)},
ymajorgrids,
yminorgrids,
ymin=0.938084134, ymax=1.0, %ymax=0.984917426,
ytick style={color=black},
ytick={0.90,0.92,0.94,0.96,0.98,1.0},
yticklabels={90,92,94,96,98,100}
]
\addplot [line width=1.5pt, color0, mark options={solid}]
table {%
1 0.959084630012512
100 0.959084630012512
};
\addlegendentry{Random}
\addplot [line width=1.5pt, color1, style={dashed}]
table {%
1 0.94021292
100 0.94021292
};
\addlegendentry{ETS}
\addplot [line width=1.5pt, color2, style={dashdotted}]
table {%
1 0.96024116
100 0.96024116
};
\addlegendentry{Heuristic}
\addplot [line width=1.5pt, color3]
table {%
1 0.959084630012512
2 0.96649968624115
3 0.967570662498474
4 0.968766689300537
5 0.968943953514099
6 0.969228386878967
7 0.969228386878967
8 0.972156524658203
9 0.972156524658203
10 0.972156524658203
11 0.972027599811554
12 0.972027599811554
13 0.972027599811554
14 0.971873462200165
15 0.972598731517792
16 0.972422778606415
17 0.972422778606415
18 0.972376048564911
19 0.972171783447266
20 0.976440250873566
21 0.976440250873566
22 0.976578116416931
23 0.976578116416931
24 0.976578116416931
25 0.97786808013916
26 0.97786808013916
27 0.97786808013916
28 0.97786808013916
29 0.97786808013916
30 0.97786808013916
31 0.97786808013916
32 0.97786808013916
33 0.97786808013916
34 0.97786808013916
35 0.97786808013916
36 0.978223025798798
37 0.978223025798798
38 0.978223025798798
39 0.978212535381317
40 0.978212535381317
41 0.978469491004944
42 0.978469491004944
43 0.978469491004944
44 0.978469491004944
45 0.978469491004944
46 0.978469491004944
47 0.978469491004944
48 0.978469491004944
49 0.978469491004944
50 0.978469491004944
51 0.978469491004944
52 0.978469491004944
53 0.978469491004944
54 0.978469491004944
55 0.978469491004944
56 0.978469491004944
57 0.978469491004944
58 0.978469491004944
59 0.978469491004944
60 0.978469491004944
61 0.978469491004944
62 0.978469491004944
63 0.978469491004944
64 0.978469491004944
65 0.978469491004944
66 0.978469491004944
67 0.978469491004944
68 0.978469491004944
69 0.978469491004944
70 0.978469491004944
71 0.978469491004944
72 0.978469491004944
73 0.978469491004944
74 0.978469491004944
75 0.978469491004944
76 0.978469491004944
77 0.978469491004944
78 0.978469491004944
79 0.978469491004944
80 0.978469491004944
81 0.978469491004944
82 0.978469491004944
83 0.978469491004944
84 0.978469491004944
85 0.978469491004944
86 0.978469491004944
87 0.978654503822327
88 0.978654503822327
89 0.978654503822327
90 0.978654503822327
91 0.978654503822327
92 0.978992760181427
93 0.978992760181427
94 0.979289412498474
95 0.979289412498474
96 0.979289412498474
97 0.979289412498474
98 0.979289412498474
99 0.979289412498474
100 0.979289412498474
};
\addlegendentry{Ours}
\addplot [line width=1.5pt, color4]
table {%
1 0.98278864
100 0.98278864
};
\addlegendentry{BFS}
\addplot [line width=1.5pt, color5]
table {%
1 0.9975396
100 0.9975396
};
\addlegendentry{Joint}
