# Supplementary material for: Learn the Time to Learn: Replay Scheduling in Continual Learning
Source: arXiv:2209.08660 source file (2023-11-20)
Supplement: Supplementary file 11 [file PermutedMNIST_rewards.tex]

\nextgroupplot[title=P-MNIST,
height=\figheight,
minor xtick={25, 75},
minor ytick={0.72, 0.74, 0.76},
tick align=outside,
tick pos=left,
width=\figwidth,
x grid style={white!69.0196078431373!black},
xlabel={Iteration},
xmajorgrids,
xminorgrids,
xmin=0, xmax=101,
xtick style={color=black},
xtick={-25,0,50,100,125},%xtick={-25,0,25,50,75,100,125},
xticklabels={-25,0,50,100,125},%xticklabels={-25,0,25,50,75,100,125},
y grid style={white!69.0196078431373!black},
ylabel={ACC (\%)},
ymajorgrids,
yminorgrids, 
ymin=0.7081526, ymax=0.771,
ytick style={color=black},
ytick={0.7,0.71, 0.73, 0.75, 0.77},
yticklabels={70, 71, 73, 75, 77},
]
\addplot [line width=1.5pt, color0]
table {%
1 0.724425971508026
100 0.724425971508026
};
%\addlegendentry{Random}
\addplot [line width=1.5pt, color1, style={dashed}]
table {%
1 0.710946
100 0.710946
};
\addplot [line width=1.5pt, color2, style={dashdotted}]
table {%
1 0.766814
100 0.766814
};
\addplot [line width=1.5pt, color3]
table {%
1 0.724425971508026
2 0.731194078922272
3 0.741815984249115
4 0.747211992740631
5 0.747211992740631
6 0.747211992740631
7 0.747233986854553
8 0.748315930366516
9 0.748315930366516
10 0.748315930366516
11 0.748315930366516
12 0.748315930366516
13 0.751919984817505
14 0.751919984817505
15 0.751919984817505
16 0.753744006156921
17 0.753744006156921
18 0.753744006156921
19 0.753744006156921
20 0.753744006156921
21 0.753744006156921
22 0.753744006156921
23 0.753744006156921
24 0.753744006156921
25 0.753744006156921
26 0.753744006156921
27 0.753744006156921
28 0.755731999874115
29 0.755731999874115
30 0.755731999874115
31 0.755731999874115
32 0.755731999874115
33 0.755731999874115
34 0.755731999874115
35 0.755731999874115
36 0.755731999874115
37 0.755731999874115
38 0.755731999874115
39 0.757443964481354
40 0.757443964481354
41 0.757443964481354
42 0.757443964481354
43 0.759189963340759
44 0.759189963340759
45 0.759189963340759
46 0.759871959686279
47 0.759871959686279
48 0.759871959686279
49 0.759871959686279
50 0.759871959686279
51 0.759871959686279
52 0.759871959686279
53 0.759871959686279
54 0.759871959686279
55 0.759871959686279
56 0.759871959686279
57 0.759871959686279
58 0.761359989643097
59 0.761359989643097
60 0.761359989643097
61 0.761359989643097
62 0.761359989643097
63 0.761359989643097
64 0.761359989643097
65 0.761359989643097
66 0.761359989643097
67 0.761359989643097
68 0.761359989643097
69 0.761359989643097
70 0.761359989643097
71 0.761359989643097
72 0.761359989643097
73 0.761359989643097
74 0.761359989643097
75 0.761359989643097
76 0.761359989643097
77 0.761359989643097
78 0.761359989643097
79 0.761359989643097
80 0.761359989643097
81 0.761359989643097
82 0.763378024101257
83 0.763378024101257
84 0.763378024101257
85 0.763378024101257
86 0.763378024101257
87 0.763378024101257
88 0.763378024101257
89 0.763378024101257
90 0.763378024101257
91 0.763378024101257
92 0.763378024101257
93 0.763378024101257
94 0.763378024101257
95 0.763378024101257
96 0.763378024101257
97 0.763378024101257
98 0.763378024101257
99 0.763378024101257
100 0.763378024101257
};
