# Supplementary material for: Learn the Time to Learn: Replay Scheduling in Continual Learning
Source: arXiv:2209.08660 source file (2023-11-20)
Supplement: Supplementary file 12 [file miniImagenet_rewards.tex]

\nextgroupplot[title=S-miniImagenet,
height=\figheight,
minor xtick={25,75},
minor ytick={0.465, 0.465, 0.475, 0.485, 0.495},
tick align=outside,
tick pos=left,
width=\figwidth,
x grid style={white!69.0196078431373!black},
xlabel={Iteration},
xmajorgrids,
xminorgrids,
xmin=0, xmax=101,
xtick style={color=black},
xtick={-25,0,50,100,125},%xtick={-25,0,25,50,75,100,125},
xticklabels={-25,0,50,100,125},%xticklabels={-25,0,25,50,75,100,125},
y grid style={white!69.0196078431373!black},
ymajorgrids,
yminorgrids,
ymin=0.468083999929428, ymax=0.50363600148201,
ytick style={color=black},
ytick={0.46, 0.47, 0.48, 0.49, 0.5, 0.51},
yticklabels={46, 47, 48, 49, 50, 51}
]
\addplot [line width=1.5pt, color0]
table {%
1 0.480820029973984
100 0.480820029973984
};

\addplot [line width=1.5pt, color1, style={dashed}]
table {%
1 0.4697
100 0.4697
};

\addplot [line width=1.5pt, color2, style={dashdotted}]
table {%
1 0.49664
100 0.49664
};

\addplot [line width=1.5pt, color3]
table {%
1 0.480820029973984
2 0.487500041723251
3 0.489940017461777
4 0.492440044879913
5 0.492440044879913
6 0.494700014591217
7 0.496280014514923
8 0.499839961528778
9 0.499839961528778
10 0.499440014362335
11 0.498420000076294
12 0.498420000076294
13 0.498420000076294
14 0.498420000076294
15 0.498420000076294
16 0.498420000076294
17 0.498420000076294
18 0.498420000076294
19 0.498420000076294
20 0.498420000076294
21 0.498420000076294
22 0.498420000076294
23 0.498420000076294
24 0.498420000076294
25 0.498420000076294
26 0.498420000076294
27 0.498420000076294
28 0.498420000076294
29 0.498420000076294
30 0.498420000076294
31 0.498420000076294
32 0.498420000076294
33 0.498420000076294
34 0.498420000076294
35 0.498420000076294
36 0.498420000076294
37 0.498420000076294
38 0.498420000076294
39 0.498420000076294
40 0.498420000076294
41 0.498420000076294
42 0.498420000076294
43 0.498420000076294
44 0.498420000076294
45 0.498420000076294
46 0.498420000076294
47 0.498420000076294
48 0.498420000076294
49 0.498420000076294
50 0.499619960784912
51 0.499619960784912
52 0.499619960784912
53 0.499619960784912
54 0.499619960784912
55 0.499619960784912
56 0.499619960784912
57 0.499619960784912
58 0.499619960784912
59 0.499619960784912
60 0.499619960784912
61 0.499619960784912
62 0.499619960784912
63 0.499619960784912
64 0.499619960784912
65 0.499619960784912
66 0.499619960784912
67 0.499619960784912
68 0.499619960784912
69 0.499619960784912
70 0.499619960784912
71 0.499619960784912
72 0.499619960784912
73 0.499619960784912
74 0.499619960784912
75 0.500059962272644
76 0.500059962272644
77 0.500059962272644
78 0.500059962272644
79 0.501500010490417
80 0.501500010490417
81 0.502020001411438
82 0.502020001411438
83 0.502020001411438
84 0.502020001411438
85 0.502020001411438
86 0.502020001411438
87 0.502020001411438
88 0.502020001411438
89 0.502020001411438
90 0.502020001411438
91 0.502020001411438
92 0.502020001411438
93 0.502020001411438
94 0.502020001411438
95 0.502020001411438
96 0.502020001411438
97 0.502020001411438
98 0.502020001411438
99 0.502020001411438
100 0.502020001411438
};
