# Supplementary material for: Learn the Time to Learn: Replay Scheduling in Continual Learning
Source: arXiv:2209.08660 source file (2023-11-20)
Supplement: Supplementary file 13 [file notMNIST_rewards.tex]

\nextgroupplot[title=S-notMNIST,
height=\figheight,
minor xtick={25,75},
minor ytick={0.91, 0.93, 0.95},%{0.92, 0.94, 0.96},
tick align=outside,
tick pos=left,
width=\figwidth,
x grid style={white!69.0196078431373!black},
xlabel={Iteration},
xmajorgrids,
xminorgrids,
xmin=0, xmax=101,
xtick style={color=black},
xtick={-25,0,50,100,125},%xtick={-25,0,25,50,75,100,125},
xticklabels={-25,0,50,100,125},%xticklabels={-25,0,25,50,75,100,125},
y grid style={white!69.0196078431373!black},
ymajorgrids,
yminorgrids, 
ymin=0.899, ymax=0.968,%ymax=0.961,
ytick style={color=black},
ytick={0.9, 0.92, 0.94, 0.96, 0.98 },%{0.9, 0.91, 0.93, 0.95 },
yticklabels={90, 92, 94, 96, 98 }%{90, 91, 93, 95}
]
\addplot [line width=1.5pt, color0]
table {%
1 0.923885941505432
100 0.923885941505432
};
%\addlegendentry{Random}
\addplot [line width=1.5pt, color1, style={dashed}]
table {%
1 0.91013312
100 0.91013312
};
%\addlegendentry{ETS}
\addplot [line width=1.5pt, color2, style={dashdotted}]
table {%
1 0.91260732
100 0.91260732
};
%\addlegendentry{Heur}
\addplot [line width=1.5pt, color3]
table {%
1 0.923885941505432
2 0.924565613269806
3 0.934316277503967
4 0.93102616071701
5 0.929313182830811
6 0.936463952064514
7 0.936463952064514
8 0.938537895679474
9 0.938537895679474
10 0.936725318431854
11 0.936725318431854
12 0.933971762657166
13 0.933971762657166
14 0.939128279685974
15 0.939128279685974
16 0.939128279685974
17 0.939128279685974
18 0.940870583057404
19 0.940870583057404
20 0.940870583057404
21 0.940870583057404
22 0.941275954246521
23 0.941275954246521
24 0.941275954246521
25 0.941275954246521
26 0.9381343126297
27 0.93654453754425
28 0.938980221748352
29 0.93954610824585
30 0.93954610824585
31 0.93954610824585
32 0.93954610824585
33 0.93954610824585
34 0.93954610824585
35 0.93954610824585
36 0.93954610824585
37 0.93954610824585
38 0.93954610824585
39 0.93954610824585
40 0.93954610824585
41 0.93954610824585
42 0.93954610824585
43 0.943730056285858
44 0.943730056285858
45 0.943730056285858
46 0.943730056285858
47 0.946393609046936
48 0.946393609046936
49 0.946393609046936
50 0.946393609046936
51 0.946393609046936
52 0.946393609046936
53 0.946393609046936
54 0.946393609046936
55 0.946393609046936
56 0.946393609046936
57 0.946393609046936
58 0.946393609046936
59 0.946393609046936
60 0.946393609046936
61 0.946393609046936
62 0.946393609046936
63 0.946393609046936
64 0.946393609046936
65 0.946393609046936
66 0.946393609046936
67 0.946393609046936
68 0.946393609046936
69 0.946393609046936
70 0.946393609046936
71 0.946393609046936
72 0.946393609046936
73 0.946393609046936
74 0.946393609046936
75 0.946393609046936
76 0.946393609046936
77 0.946393609046936
78 0.946393609046936
79 0.946393609046936
80 0.946393609046936
81 0.946393609046936
82 0.946393609046936
83 0.946393609046936
84 0.946393609046936
85 0.946393609046936
86 0.946393609046936
87 0.946393609046936
88 0.946393609046936
89 0.946393609046936
90 0.946393609046936
91 0.946393609046936
92 0.946393609046936
93 0.946393609046936
94 0.946393609046936
95 0.946393609046936
96 0.946393609046936
97 0.946393609046936
98 0.946393609046936
99 0.946393609046936
100 0.946393609046936
};
%\addlegendentry{RS-MCTS}
\addplot [line width=1.5pt, color4]
table {%
1 0.95536152
100 0.95536152
};
%\addlegendentry{BFS}
\addplot [line width=1.5pt, color5]
table {%
1 0.96119168
100 0.96119168
};
%\addlegendentry{Joint}
