# Supplementary material for: Learn the Time to Learn: Replay Scheduling in Continual Learning
Source: arXiv:2209.08660 source file (2023-11-20)
Supplement: Supplementary file 14 [file memory_usage_10task_datasets_barplot.tex]

\nextgroupplot[title={Memory Usage for 10-task Permuted MNIST },
ybar,
bar width = 4pt,
height=\figheight,
legend cell align={left},
legend columns=2,
legend style={
  fill opacity=0.9,
  draw opacity=1,
  text opacity=1,
  at={(0.03,0.7)},
  anchor=south west,
  draw=white!80!black
},
minor xtick={},
minor ytick={},
tick align=outside,
tick pos=left,
width=\figwidth,
x grid style={white!69.0196078431373!black},
xlabel={Task},
xmin=1.5, xmax=10.5,
xtick style={color=black},
xtick={2,3,4,5,6,7,8,9,10},
xticklabels={2,3,4,5,6,7,8,9,10},
y grid style={white!69.0196078431373!black},
ymajorgrids,
ylabel={\#Replayed Samples},
ymin=0.0, ymax=102,
ytick style={color=black},
ytick={0,10,20,30,40,50,60,70,80,90,100},
yticklabels={0,10,20,30,40,50,60,70,80,90,100}
]

\addplot [draw=black, fill=color0] coordinates {
(2,10)
(3,20)
(4,30)
(5,40)
(6,50)
(7,50)
(8,50)
(9,50)
(10,50)
};\addlegendentry{Ours}

\addplot [draw=black, fill=color1] coordinates {
(2,10)
(3,20)
(4,30)
(5,40)
(6,50)
(7,60)
(8,70)
(9,80)
(10,90)
};\addlegendentry{Baselines}
