# Supplementary material for: Learn the Time to Learn: Replay Scheduling in Continual Learning
Source: arXiv:2209.08660 source file (2023-11-20)
Supplement: Supplementary file 15 [file memory_usage_20task_datasets_barplot.tex]

\nextgroupplot[title={Memory Usage for the 20-task Datasets},
ybar,
bar width = 4pt,
height=\figheight,
legend cell align={left},
legend columns=2,
legend style={
  fill opacity=0.9,
  draw opacity=1,
  text opacity=1,
  at={(0.03,0.7)},
  anchor=south west,
  draw=white!80!black
},
minor xtick={},
minor ytick={},
tick align=outside,
tick pos=left,
width=\figwidth,
x grid style={white!69.0196078431373!black},
xlabel={Task},
xmin=1.5, xmax=20.5,
xtick style={color=black},
xtick={2,3,4,5,6,7,8,9,10,11,12,13,14,15,16,17,18,19,20},
xticklabels={2,3,4,5,6,7,8,9,10,11,12,13,14,15,16,17,18,19,20},
y grid style={white!69.0196078431373!black},
ymajorgrids,
ylabel={\#Replayed Samples},
ymin=0.0, ymax=102,
ytick style={color=black},
ytick={0,10,20,30,40,50,60,70,80,90,100},
yticklabels={0,10,20,30,40,50,60,70,80,90,100}
]

\addplot [draw=black, fill=color0] coordinates {
(2,5)
(3,10)
(4,15)
(5,20)
(6,25)
(7,30)
(8,35)
(9,40)
(10,45)
(11,50)
(12,50)
(13,50)
(14,50)
(15,50)
(16,50)
(17,50)
(18,50)
(19,50)
(20,50)
};\addlegendentry{Ours}

\addplot [draw=black, fill=color1] coordinates {
(2,5)
(3,10)
(4,15)
(5,20)
(6,25)
(7,30)
(8,35)
(9,40)
(10,45)
(11,50)
(12,55)
(13,60)
(14,65)
(15,70)
(16,75)
(17,80)
(18,85)
(19,90)
(20,95)
};\addlegendentry{Baselines}
