# Supplementary material for: Learn the Time to Learn: Replay Scheduling in Continual Learning
Source: arXiv:2209.08660 source file (2023-11-20)
Supplement: Supplementary file 17 [file rewards_env1.tex]

\nextgroupplot[title=Seed 10,
height=\figheight,
legend cell align={left},
legend columns=-1,
legend style={
  fill opacity=0.8,
  draw opacity=1,
  text opacity=1,
  at={(0.10,1.29)},
  anchor=south west,
  draw=white!80!black
},
minor xtick={25, 75},
minor ytick={},
tick align=outside,
tick pos=left,
width=\figwidth,
x grid style={white!69.0196078431373!black},
xlabel={Eval. Steps},
xminorgrids,
xmajorgrids,
xmin=-3.95, xmax=104.95,
xtick style={color=black},
xtick={-25,0,50,100,125},
xticklabels={-25,0,50,100,125},
y grid style={white!69.0196078431373!black},
ylabel={ACC (\%)},
ymajorgrids,
ymin=0.83, ymax=0.89,
ytick style={color=black},
ytick={0.83,0.84,0.85,0.86,0.87,0.88,0.89},
yticklabels={83,84,85,86,87,88,89}
]
\addplot [semithick, color0]
table {%
1 0.862333333492279
2 0.887299990653992
3 0.860200003782908
4 0.847733334700267
5 0.844633336861928
6 0.846200001239776
7 0.846200001239776
8 0.845266668001811
9 0.84663333495458
10 0.845500004291534
11 0.845500004291534
12 0.845266668001811
13 0.845500004291534
14 0.847800000508626
15 0.845500004291534
16 0.845500004291534
17 0.845500004291534
18 0.845500004291534
19 0.845500004291534
20 0.845500004291534
21 0.845500004291534
22 0.845500004291534
23 0.845500004291534
24 0.845500004291534
25 0.845500004291534
26 0.845500004291534
27 0.845500004291534
28 0.845500004291534
29 0.850333340962728
30 0.845500004291534
31 0.845500004291534
32 0.845500004291534
33 0.845500004291534
34 0.850333340962728
35 0.850333340962728
36 0.845500004291534
37 0.845500004291534
38 0.845500004291534
39 0.850333340962728
40 0.845500004291534
41 0.850333340962728
42 0.845500004291534
43 0.845500004291534
44 0.845500004291534
45 0.850333340962728
46 0.845500004291534
47 0.845500004291534
48 0.850333340962728
49 0.845500004291534
50 0.850333340962728
51 0.845500004291534
52 0.845500004291534
53 0.850333340962728
54 0.854500007629394
55 0.845500004291534
56 0.845500004291534
57 0.845500004291534
58 0.850333340962728
59 0.850333340962728
60 0.845500004291534
61 0.845500004291534
62 0.845500004291534
63 0.845500004291534
64 0.854500007629395
65 0.850333340962728
66 0.845500004291534
67 0.845500004291534
68 0.845500004291534
69 0.845500004291534
70 0.845500004291534
71 0.850333340962728
72 0.850333340962728
73 0.850333340962728
74 0.845500004291534
75 0.850333340962728
76 0.845500004291534
77 0.850333340962728
78 0.845500004291534
79 0.850333340962728
80 0.845500004291534
81 0.853833337624868
82 0.845500004291534
83 0.855166677633921
84 0.859333344300588
85 0.845500004291534
86 0.845500004291534
87 0.854500007629395
88 0.850333340962728
89 0.850333340962728
90 0.850333340962728
91 0.850333340962728
92 0.855166677633921
93 0.849666670958201
94 0.845500004291534
95 0.840733333428701
96 0.840966669718424
97 0.845266668001811
98 0.854500007629395
99 0.854500007629394
100 0.845500004291534
};
\addlegendentry{A2C}
\addplot [semithick, color1]
table {%
1 0.864133334159851
2 0.855000003178914
3 0.849366660912832
4 0.846766670544942
5 0.863299997647603
6 0.845399995644887
7 0.85489999850591
8 0.84576667547226
9 0.839133330186208
10 0.854566669464111
11 0.85103333791097
12 0.850766674677531
13 0.857833325862885
14 0.849833337465922
15 0.849399999777476
16 0.847166665395101
17 0.847900001207987
18 0.840466674168905
19 0.845766667524974
20 0.840499997138977
21 0.844099998474121
22 0.845766667524974
23 0.841500000158946
24 0.850033338864644
25 0.84363333384196
26 0.850633343060811
27 0.845866668224335
28 0.849966669082642
29 0.845799998442332
30 0.83846667210261
31 0.834366663297017
32 0.844533328215281
33 0.839699999491374
34 0.851266662279765
35 0.844333334763845
36 0.844100002447764
37 0.846200001239777
38 0.845100005467733
39 0.858233332633972
40 0.838366663455963
41 0.846200001239777
42 0.847100003560384
43 0.8439333319664
44 0.844600001970927
45 0.850166666507721
46 0.84600000778834
47 0.84396667877833
48 0.83793332974116
49 0.842866675059001
50 0.84796667098999
51 0.841199998060862
52 0.862266663710276
53 0.845433330535889
54 0.858399999141693
55 0.856466666857401
56 0.851366674900055
57 0.850500003496806
58 0.862299998601278
59 0.851266662279765
60 0.867766666412354
61 0.841233328978221
62 0.858699997266134
63 0.857266668478648
64 0.858699997266134
65 0.85760000149409
66 0.849400007724762
67 0.837433342138926
68 0.847133338451385
69 0.870166671276093
70 0.846300001939138
71 0.856600002447764
72 0.844500001271566
73 0.848533328374227
74 0.866333329677582
75 0.86416666507721
76 0.853733336925507
77 0.860399993260701
78 0.867066657543182
79 0.860633325576782
80 0.865333330631256
81 0.865333330631256
82 0.865766664346059
83 0.857899995644887
84 0.843533333142598
85 0.851166661580404
86 0.866466657320658
87 0.850066657861074
88 0.873899992307027
89 0.846233328183492
90 0.865333330631256
91 0.867533326148987
92 0.865333330631256
93 0.860633325576782
94 0.856766668955485
95 0.861833341916402
96 0.851366670926412
97 0.865333330631256
98 0.878599997361501
99 0.873899992307027
100 0.871166662375132
};
\addlegendentry{DQN}
\addplot [semithick, color2]
table {%
1 0.860766666666667
100 0.860766666666667
};
\addlegendentry{Random}
\addplot [semithick, color3]
table {%
1 0.871
100 0.871
};
\addlegendentry{ETS}
\addplot [semithick, color4]
table {%
1 0.8631
100 0.8631
};
\addlegendentry{Heur-GD}
\addplot [semithick, color5, dash pattern=on 1pt off 3pt on 3pt off 3pt]
table {%
1 0.8667
100 0.8667
};
\addlegendentry{Heur-LD}
\addplot [semithick, color6, dashed]
table {%
1 0.8594
100 0.8594
};
\addlegendentry{Heur-AT}
