# Supplementary material for: Learn the Time to Learn: Replay Scheduling in Continual Learning
Source: arXiv:2209.08660 source file (2023-11-20)
Supplement: Supplementary file 18 [file rewards_env10.tex]

\nextgroupplot[title=Seed 19,
height=\figheight,
legend cell align={left},
legend style={
  fill opacity=0.8,
  draw opacity=1,
  text opacity=1,
  at={(0.5,0.09)},
  anchor=south,
  draw=white!80!black
},
minor xtick={25, 75},
minor ytick={},
tick align=outside,
tick pos=left,
width=\figwidth,
x grid style={white!69.0196078431373!black},
xlabel={Eval. Steps},
xminorgrids,
xmajorgrids,
xmin=-3.95, xmax=104.95,
xtick style={color=black},
xtick={-25,0,50,100,125},
xticklabels={-25,0,50,100,125},
y grid style={white!69.0196078431373!black},
ymajorgrids,
ymin=0.731755009293556, ymax=0.822944995760918,
ytick style={color=black},
ytick={0.72,0.74,0.76,0.78,0.8,0.82,0.84},
yticklabels={72,74,76,78,80,82,84}
]
\addplot [semithick, color0]
table {%
1 0.753933334350586
2 0.735900008678436
3 0.775166662534078
4 0.798000001907349
5 0.805466667811076
6 0.818799996376038
7 0.794933334986369
8 0.809466656049093
9 0.784666673342387
10 0.800799997647603
11 0.794933334986369
12 0.800799997647603
13 0.787466669082642
14 0.805466667811076
15 0.796133327484131
16 0.818799996376038
17 0.805466667811076
18 0.787466669082642
19 0.800799997647603
20 0.814133326212565
21 0.814133326212565
22 0.80479998588562
23 0.790266664822896
24 0.814133326212565
25 0.792133339246114
26 0.809466656049093
27 0.809466656049093
28 0.808266663551331
29 0.809466656049093
30 0.814133326212565
31 0.818799996376038
32 0.814133326212565
33 0.787466669082642
34 0.791999999682109
35 0.818799996376038
36 0.800799997647603
37 0.80479998588562
38 0.818799996376038
39 0.799199994405111
40 0.796133327484131
41 0.809466656049093
42 0.796133327484131
43 0.809466656049093
44 0.80479998588562
45 0.80479998588562
46 0.80479998588562
47 0.809466656049093
48 0.80479998588562
49 0.799199994405111
50 0.803666659196218
51 0.809466656049093
52 0.809466656049093
53 0.80533332824707
54 0.80479998588562
55 0.799199994405111
56 0.80479998588562
57 0.80479998588562
58 0.800666658083598
59 0.796133327484131
60 0.803666659196218
61 0.80479998588562
62 0.80479998588562
63 0.80479998588562
64 0.796533330281576
65 0.803666659196218
66 0.799199994405111
67 0.80479998588562
68 0.80479998588562
69 0.80479998588562
70 0.80479998588562
71 0.80479998588562
72 0.80479998588562
73 0.80479998588562
74 0.80479998588562
75 0.80479998588562
76 0.80479998588562
77 0.80479998588562
78 0.80479998588562
79 0.800666658083598
80 0.80479998588562
81 0.80479998588562
82 0.80479998588562
83 0.80479998588562
84 0.80479998588562
85 0.80479998588562
86 0.80479998588562
87 0.80479998588562
88 0.800666658083598
89 0.80479998588562
90 0.80479998588562
91 0.80479998588562
92 0.80479998588562
93 0.80479998588562
94 0.80479998588562
95 0.80479998588562
96 0.80479998588562
97 0.80479998588562
98 0.800666658083598
99 0.80479998588562
100 0.80479998588562
};
%\addlegendentry{a2c, gae, envs=10, lr=0.0003, act=tanh}
\addplot [semithick, color1]
table {%
1 0.753533331553141
2 0.760299996534983
3 0.776099995772044
4 0.774000004927317
5 0.764400001366933
6 0.773000005880992
7 0.779333329200745
8 0.773633337020874
9 0.786400000254313
10 0.782933334509532
11 0.794199999173482
12 0.793599998950958
13 0.792500003178914
14 0.785566667715708
15 0.799933322270711
16 0.779499999682108
17 0.79913334051768
18 0.80116666952769
19 0.792500007152557
20 0.793099995454152
21 0.790000001589457
22 0.795366668701172
23 0.79663333495458
24 0.800433333714803
25 0.807866668701172
26 0.801800000667572
27 0.79656666914622
28 0.791433334350586
29 0.799366660912832
30 0.797699999809265
31 0.801433336734772
32 0.795133332411448
33 0.793900005022685
34 0.797299993038178
35 0.806766672929128
36 0.801133334636688
37 0.803866672515869
38 0.789866669972738
39 0.802900004386902
40 0.805633342266083
41 0.802900004386902
42 0.7964333375295
43 0.81409999926885
44 0.79853333234787
45 0.806699999173482
46 0.789199999968211
47 0.80446666876475
48 0.812366664409637
49 0.806333339214325
50 0.802533332506816
51 0.793800004323324
52 0.793833331267039
53 0.806266673405965
54 0.802800003687541
55 0.786333334445953
56 0.795700001716614
57 0.786333334445953
58 0.795966668923696
59 0.797733338673909
60 0.797733338673909
61 0.788366671403249
62 0.788366671403249
63 0.791266671816508
64 0.791366668542226
65 0.788366671403249
66 0.796266674995422
67 0.782866664727529
68 0.780133334795634
69 0.79306667248408
70 0.790300003687541
71 0.780133334795634
72 0.776666665077209
73 0.780133334795634
74 0.77303333679835
75 0.784966667493184
76 0.780399998029073
77 0.791133332252503
78 0.789266669750214
79 0.783199997742971
80 0.786799999078115
81 0.78333332935969
82 0.798633329073588
83 0.792199993133545
84 0.787899998823802
85 0.794199999173482
86 0.792466672261556
87 0.794199999173482
88 0.771266671021779
89 0.789000002543132
90 0.79313333829244
91 0.786733333269755
92 0.786733333269755
93 0.792466672261556
94 0.789866669972738
95 0.768666668732961
96 0.774399999777476
97 0.781233334541321
98 0.784133330980937
99 0.791633323828379
100 0.797966663042704
};
%\addlegendentry{DQN, n train envs=10, lr=0.00003}
\addplot [semithick, color2]
table {%
1 0.739533333333333
100 0.739533333333333
};
%\addlegendentry{Random}
\addplot [semithick, color3]
table {%
1 0.7767
100 0.7767
};
%\addlegendentry{ETS}
\addplot [semithick, color4]
table {%
1 0.7787
100 0.7787
};
%\addlegendentry{Heur-GD}
\addplot [semithick, color5, dash pattern=on 1pt off 3pt on 3pt off 3pt]
table {%
1 0.775
100 0.775
};
%\addlegendentry{Heur-LD}
\addplot [semithick, color6, dashed]
table {%
1 0.7787
100 0.7787
};
%\addlegendentry{Heur-AT}
