# Supplementary material for: Learn the Time to Learn: Replay Scheduling in Continual Learning
Source: arXiv:2209.08660 source file (2023-11-20)
Supplement: Supplementary file 19 [file rewards_env2.tex]

\nextgroupplot[title=Seed 11,
height=\figheight,
legend cell align={left},
legend style={
  fill opacity=0.8,
  draw opacity=1,
  text opacity=1,
  at={(0.97,0.03)},
  anchor=south east,
  draw=white!80!black
},
minor xtick={25, 75},
minor ytick={},
tick align=outside,
tick pos=left,
width=\figwidth,
x grid style={white!69.0196078431373!black},
xlabel={Eval. Steps},
xminorgrids,
xmajorgrids,
xmin=-3.95, xmax=104.95,
xtick style={color=black},
xtick={-25,0,50,100,125},
xticklabels={-25,0,50,100,125},
y grid style={white!69.0196078431373!black},
ymajorgrids,
ymin=0.725908333004316, ymax=0.84,
ytick style={color=black},
ytick={0.72,0.74,0.76,0.78,0.8,0.82,0.84},
yticklabels={72,74,76,78,80,82,84}
]
\addplot [semithick, color0]
table {%
1 0.800666662057241
2 0.798399996757507
3 0.800233328342438
4 0.783200005690257
5 0.784200000762939
6 0.764900004863739
7 0.792166666189829
8 0.804733331998189
9 0.81146666208903
10 0.82279999256134
11 0.82279999256134
12 0.794466666380564
13 0.82279999256134
14 0.784200000762939
15 0.813766662279765
16 0.82279999256134
17 0.80349999666214
18 0.82279999256134
19 0.792166666189829
20 0.775166670481364
21 0.784200000762939
22 0.794466666380564
23 0.81146666208903
24 0.794466666380564
25 0.80349999666214
26 0.794466666380564
27 0.783133335908254
28 0.772866670290629
29 0.805566668510437
30 0.772866670290629
31 0.764900004863739
32 0.824866664409637
33 0.824866664409637
34 0.829000008106232
35 0.807633340358734
36 0.815833334128062
37 0.817066673437754
38 0.786266672611237
39 0.829000008106232
40 0.807633340358734
41 0.829000008106232
42 0.807633340358734
43 0.829000008106232
44 0.831433339913686
45 0.807633340358734
46 0.817066673437754
47 0.803899999459584
48 0.807633340358734
49 0.831433339913686
50 0.817066673437754
51 0.829000008106232
52 0.800233336289724
53 0.829000008106232
54 0.809666669368744
55 0.817066673437754
56 0.829000008106232
57 0.807633340358734
58 0.829000008106232
59 0.807633340358734
60 0.829000008106232
61 0.829000008106232
62 0.805133338769277
63 0.829000008106232
64 0.821600004037221
65 0.817066673437754
66 0.829000008106232
67 0.829000008106232
68 0.817066673437754
69 0.829000008106232
70 0.829000008106232
71 0.815400012334188
72 0.829000008106232
73 0.819300003846486
74 0.829000008106232
75 0.817066673437754
76 0.829000008106232
77 0.829000008106232
78 0.829000008106232
79 0.829000008106232
80 0.829000008106232
81 0.829000008106232
82 0.812166666984558
83 0.829000008106232
84 0.829000008106232
85 0.829000008106232
86 0.829000008106232
87 0.829000008106232
88 0.817066673437754
89 0.829000008106232
90 0.812166666984558
91 0.829000008106232
92 0.829000008106232
93 0.812166666984558
94 0.829000008106232
95 0.812166666984558
96 0.817066673437754
97 0.829000008106232
98 0.812166666984558
99 0.829000008106232
100 0.829000008106232
};
%\addlegendentry{a2c, gae, envs=10, lr=0.0003, act=tanh}
\addplot [semithick, color1]
table {%
1 0.798399996757507
2 0.800266659259796
3 0.795066658655803
4 0.820999999841054
5 0.791233332951864
6 0.787599996725718
7 0.799466665585836
8 0.800099996725718
9 0.789166680971781
10 0.794499997297923
11 0.787333333492279
12 0.795866668224335
13 0.790433327356974
14 0.811800003051758
15 0.781266661485036
16 0.800833340485891
17 0.800066661834717
18 0.788900005817413
19 0.798366657892863
20 0.791633335749308
21 0.781833326816559
22 0.790300003687541
23 0.809833339850108
24 0.808933333555857
25 0.772366658846537
26 0.806666664282481
27 0.800066657861074
28 0.795866656303406
29 0.801366662979126
30 0.811433327198029
31 0.806099998950958
32 0.794733329614004
33 0.791699993610382
34 0.792500003178914
35 0.804166666666667
36 0.794733329614004
37 0.790799999237061
38 0.794100002447764
39 0.808566665649414
40 0.784766666094462
41 0.7996333360672
42 0.812066666285197
43 0.7996333360672
44 0.7996333360672
45 0.804766658941905
46 0.79760000705719
47 0.795700005690257
48 0.7996333360672
49 0.795800002415975
50 0.796566657225291
51 0.795600001017253
52 0.790133325258891
53 0.801466663678487
54 0.801466663678487
55 0.806966666380564
56 0.80313333272934
57 0.788266662756602
58 0.806966666380564
59 0.801499994595845
60 0.797666660944621
61 0.801466663678487
62 0.801499994595845
63 0.800066661834717
64 0.806966666380564
65 0.809033326307932
66 0.809033326307932
67 0.805133338769277
68 0.809033326307932
69 0.805199992656708
70 0.806966666380564
71 0.803199998537699
72 0.806966666380564
73 0.806966666380564
74 0.796866659323375
75 0.795033331712087
76 0.806966666380564
77 0.809033326307932
78 0.795033331712087
79 0.795033331712087
80 0.795033331712087
81 0.796866659323375
82 0.797666660944621
83 0.795033331712087
84 0.791199998060862
85 0.795033331712087
86 0.795033331712087
87 0.798900000254313
88 0.791199998060862
89 0.795033331712087
90 0.799433334668477
91 0.791199998060862
92 0.787366664409637
93 0.791199998060862
94 0.795033331712087
95 0.791199998060862
96 0.791199998060862
97 0.791199998060862
98 0.791199998060862
99 0.79303332567215
100 0.791199998060862
};
%\addlegendentry{DQN, n train envs=10, lr=0.00003}
\addplot [semithick, color2]
table {%
1 0.730933333333333
100 0.730933333333333
};
%\addlegendentry{Random}
\addplot [semithick, color3]
table {%
1 0.7516
100 0.7516
};
%\addlegendentry{ETS}
\addplot [semithick, color4]
table {%
1 0.7945
100 0.7945
};
%\addlegendentry{Heur-GD}
\addplot [semithick, color5, dash pattern=on 1pt off 3pt on 3pt off 3pt]
table {%
1 0.8164
100 0.8164
};
%\addlegendentry{Heur-LD}
\addplot [semithick, color6, dashed]
table {%
1 0.8112
100 0.8112
};
%\addlegendentry{Heur-AT}
