# Supplementary material for: Learn the Time to Learn: Replay Scheduling in Continual Learning
Source: arXiv:2209.08660 source file (2023-11-20)
Supplement: Supplementary file 20 [file rewards_env3.tex]

\nextgroupplot[title=Seed 12,
height=\figheight,
legend cell align={left},
legend style={
  fill opacity=0.8,
  draw opacity=1,
  text opacity=1,
  at={(0.5,0.91)},
  anchor=north,
  draw=white!80!black
},
minor xtick={25, 75},
minor ytick={},
tick align=outside,
tick pos=left,
width=\figwidth,
x grid style={white!69.0196078431373!black},
xlabel={Eval. Steps},
xminorgrids,
xmajorgrids,
xmin=-3.95, xmax=104.95,
xtick style={color=black},
xtick={-25,0,50,100,125},
xticklabels={-25,0,50,100,125},
y grid style={white!69.0196078431373!black},
ymajorgrids,
ymin=0.85, ymax=0.90,
ytick style={color=black},
ytick={0.85,0.86,0.87,0.88,0.89,0.9},
yticklabels={85,86,87,88,89,90}
]
\addplot [semithick, color0]
table {%
1 0.869400000572205
2 0.866699993610382
3 0.877433335781097
4 0.868900008996328
5 0.863866678873698
6 0.863900017738342
7 0.868000014623006
8 0.862233336766561
9 0.868866670131684
10 0.863033338387807
11 0.867166674137115
12 0.863033338387807
13 0.862233336766561
14 0.863866678873698
15 0.862199997901916
16 0.863900017738342
17 0.863866678873698
18 0.862999999523163
19 0.862233336766561
20 0.863066677252452
21 0.863066677252452
22 0.86139999628067
23 0.86139999628067
24 0.863066677252452
25 0.863033338387807
26 0.862233336766561
27 0.863066677252452
28 0.868000014623006
29 0.865733337402344
30 0.863066677252452
31 0.863900017738342
32 0.863066677252452
33 0.863033338387807
34 0.870966668923696
35 0.866566677888234
36 0.862233336766561
37 0.86139999628067
38 0.863900017738342
39 0.867766666412354
40 0.862199997901916
41 0.866866672039032
42 0.862233336766561
43 0.865833334128062
44 0.86139999628067
45 0.865833334128062
46 0.86139999628067
47 0.862233336766561
48 0.866033331553141
49 0.86139999628067
50 0.867266662915548
51 0.86139999628067
52 0.871500007311503
53 0.866666674613953
54 0.875100004673004
55 0.865833334128062
56 0.86139999628067
57 0.86139999628067
58 0.870466669400533
59 0.866633331775665
60 0.870266671975454
61 0.86139999628067
62 0.86139999628067
63 0.865833334128062
64 0.875100004673004
65 0.871700000762939
66 0.863133331139882
67 0.866033331553141
68 0.865833334128062
69 0.870466669400533
70 0.86139999628067
71 0.866033331553141
72 0.870666666825612
73 0.866033331553141
74 0.866033331553141
75 0.870466669400533
76 0.866033331553141
77 0.870666666825612
78 0.86139999628067
79 0.866033331553141
80 0.86139999628067
81 0.870666666825612
82 0.86139999628067
83 0.870666666825612
84 0.875300002098083
85 0.870666666825612
86 0.866033331553141
87 0.870666666825612
88 0.866033331553141
89 0.870666666825612
90 0.870666666825612
91 0.866033331553141
92 0.875300002098083
93 0.866033331553141
94 0.870466669400533
95 0.870666666825612
96 0.86139999628067
97 0.875300002098083
98 0.870666666825612
99 0.875300002098083
100 0.866033331553141
};
%\addlegendentry{a2c, gae, envs=10, lr=0.0003, act=tanh}
\addplot [semithick, color1]
table {%
1 0.866833333174388
2 0.874633340040843
3 0.867633338769277
4 0.866500000158946
5 0.866400003433228
6 0.869200007120768
7 0.866000004609426
8 0.863366675376892
9 0.867000003655752
10 0.87150000333786
11 0.867033338546753
12 0.864400001366933
13 0.867066665490468
14 0.862933333714803
15 0.868800004323324
16 0.858600000540415
17 0.864133330186208
18 0.877333335081736
19 0.867833332220713
20 0.870466669400533
21 0.859666669368744
22 0.876933332284291
23 0.864566671848297
24 0.866466665267944
25 0.865899999936422
26 0.859766666094462
27 0.863200004895528
28 0.863800001144409
29 0.866933333873749
30 0.867233331998189
31 0.856299996376038
32 0.868233327070872
33 0.861666671435038
34 0.863200004895528
35 0.861100002129873
36 0.86850000222524
37 0.86696666876475
38 0.867733339468638
39 0.863733339309692
40 0.869800003369649
41 0.866666658719381
42 0.863166666030884
43 0.862466669082642
44 0.864800000190735
45 0.861299999554952
46 0.861666671435038
47 0.870766667524974
48 0.861333338419596
49 0.865699998537699
50 0.859500002861023
51 0.859766666094462
52 0.862100001176198
53 0.865166672070821
54 0.858433338006337
55 0.860366670290629
56 0.862300006548564
57 0.862100001176198
58 0.860366670290629
59 0.859500002861023
60 0.860366670290629
61 0.860366670290629
62 0.860366670290629
63 0.85710000594457
64 0.85600000222524
65 0.859533333778381
66 0.857366669178009
67 0.854533338546753
68 0.860366670290629
69 0.863433337211609
70 0.860366670290629
71 0.863433337211609
72 0.858033335208893
73 0.858666674296061
74 0.860366670290629
75 0.858033335208893
76 0.853866664568583
77 0.865666667620341
78 0.858033335208893
79 0.856333339214325
80 0.858666674296061
81 0.858033335208893
82 0.860366670290629
83 0.858666674296061
84 0.860366670290629
85 0.860366670290629
86 0.860366670290629
87 0.860366670290629
88 0.858666674296061
89 0.856333339214325
90 0.861966669559479
91 0.860366670290629
92 0.860366670290629
93 0.858900002638499
94 0.860366670290629
95 0.860366670290629
96 0.857066667079926
97 0.857066667079926
98 0.857066667079926
99 0.857066667079926
100 0.853533339500427
};
%\addlegendentry{DQN, n train envs=10, lr=0.00003}
\addplot [semithick, color2]
table {%
1 0.875566666666667
100 0.875566666666667
};
%\addlegendentry{Random}
\addplot [semithick, color3]
table {%
1 0.8553
100 0.8553
};
%\addlegendentry{ETS}
\addplot [semithick, color4]
table {%
1 0.8976
100 0.8976
};
%\addlegendentry{Heur-GD}
\addplot [semithick, color5, dash pattern=on 1pt off 3pt on 3pt off 3pt]
table {%
1 0.8752
100 0.8752
};
%\addlegendentry{Heur-LD}
\addplot [semithick, color6, dashed]
table {%
1 0.8957
100 0.8957
};
%\addlegendentry{Heur-AT}
