# Supplementary material for: Learn the Time to Learn: Replay Scheduling in Continual Learning
Source: arXiv:2209.08660 source file (2023-11-20)
Supplement: Supplementary file 21 [file rewards_env4.tex]

\nextgroupplot[title=Seed 13,
height=\figheight,
legend cell align={left},
legend style={
  fill opacity=0.8,
  draw opacity=1,
  text opacity=1,
  at={(0.5,0.09)},
  anchor=south,
  draw=white!80!black
},
minor xtick={25, 75},
minor ytick={},
tick align=outside,
tick pos=left,
width=\figwidth,
x grid style={white!69.0196078431373!black},
xlabel={Eval. Steps},
xminorgrids,
xmajorgrids,
xmin=-3.95, xmax=104.95,
xtick style={color=black},
xtick={-25,0,50,100,125},
xticklabels={-25,0,50,100,125},
y grid style={white!69.0196078431373!black},
ymajorgrids,
ymin=0.766089999723435, ymax=0.82,
ytick style={color=black},
ytick={0.76,0.77,0.78,0.79,0.8,0.81,0.82},
yticklabels={76,77,78,79,80,81,82}
]
\addplot [semithick, color0]
table {%
1 0.795866672197978
2 0.78270001411438
3 0.797366674741109
4 0.812333337465922
5 0.807566654682159
6 0.809599999586741
7 0.809599999586741
8 0.812633331616719
9 0.811666671435038
10 0.811733333269755
11 0.81170000632604
12 0.810566659768422
13 0.813033334414164
14 0.81453332901001
15 0.816333333651225
16 0.81453332901001
17 0.815499997138977
18 0.815499997138977
19 0.815499997138977
20 0.815499997138977
21 0.815499997138977
22 0.815499997138977
23 0.815499997138977
24 0.815499997138977
25 0.815499997138977
26 0.815499997138977
27 0.815499997138977
28 0.815499997138977
29 0.815499997138977
30 0.815499997138977
31 0.815499997138977
32 0.815499997138977
33 0.816300002733866
34 0.816700005531311
35 0.816700005531311
36 0.816700005531311
37 0.816700005531311
38 0.816700005531311
39 0.816700005531311
40 0.816700005531311
41 0.816700005531311
42 0.816700005531311
43 0.816700005531311
44 0.816700005531311
45 0.816700005531311
46 0.816700005531311
47 0.816700005531311
48 0.816700005531311
49 0.816700005531311
50 0.816700005531311
51 0.816700005531311
52 0.816700005531311
53 0.816700005531311
54 0.816700005531311
55 0.816700005531311
56 0.816700005531311
57 0.816700005531311
58 0.816700005531311
59 0.811466670036316
60 0.816700005531311
61 0.816700005531311
62 0.815466666221619
63 0.811466670036316
64 0.815466666221619
65 0.815466666221619
66 0.812999987602234
67 0.815466666221619
68 0.814233326911926
69 0.815466666221619
70 0.814233326911926
71 0.816266667842865
72 0.814233326911926
73 0.812999987602234
74 0.814233326911926
75 0.814233326911926
76 0.812999987602234
77 0.814233326911926
78 0.812999987602234
79 0.8128666639328
80 0.811933322747548
81 0.812099993228912
82 0.813866662979126
83 0.814233326911926
84 0.811933322747548
85 0.812999987602234
86 0.813166662057241
87 0.814233326911926
88 0.812999987602234
89 0.813166658083598
90 0.812999987602234
91 0.812633323669434
92 0.812999987602234
93 0.812999987602234
94 0.815033328533173
95 0.812999987602234
96 0.812999987602234
97 0.812999987602234
98 0.812999987602234
99 0.812999987602234
100 0.811933322747548
};
%\addlegendentry{a2c, gae, envs=10, lr=0.0003, act=tanh}
\addplot [semithick, color1]
table {%
1 0.799166663487752
2 0.800333336989085
3 0.804266663392385
4 0.790233329931895
5 0.804466660817464
6 0.808233336607615
7 0.805666665236155
8 0.810966674486796
9 0.804799997806549
10 0.803966661294301
11 0.809100008010864
12 0.81096666653951
13 0.809766670068105
14 0.805333340167999
15 0.809500002861023
16 0.813900009791056
17 0.809100008010864
18 0.805400005976359
19 0.812933333714803
20 0.810566675662994
21 0.812766671180725
22 0.809799993038178
23 0.811933322747548
24 0.809799993038178
25 0.814133334159851
26 0.813966663678487
27 0.809799993038178
28 0.816000004609426
29 0.811033328374227
30 0.811366657416026
31 0.809966659545898
32 0.812933325767517
33 0.812933325767517
34 0.813333328564962
35 0.812833329041799
36 0.811699990431468
37 0.814533336957296
38 0.810666664441427
39 0.812933325767517
40 0.814133334159851
41 0.811066667238871
42 0.807533331712087
43 0.807766664028168
44 0.812966664632161
45 0.811233337720235
46 0.81096666653951
47 0.811033328374227
48 0.812666658560435
49 0.81306666135788
50 0.812133324146271
51 0.811466658115387
52 0.811633328596751
53 0.809266666571299
54 0.81096666653951
55 0.811199998855591
56 0.811199998855591
57 0.810466667016347
58 0.810466667016347
59 0.810466667016347
60 0.802399996916453
61 0.80313333272934
62 0.800266667207082
63 0.796600008010864
64 0.808199997742971
65 0.807833329836527
66 0.802066663901011
67 0.810466667016347
68 0.807833329836527
69 0.810466667016347
70 0.802399996916453
71 0.812866671880086
72 0.809233331680298
73 0.809233331680298
74 0.800266667207082
75 0.801500002543131
76 0.800266667207082
77 0.809233331680298
78 0.809233331680298
79 0.812333329518636
80 0.806166660785675
81 0.800266667207082
82 0.805699992179871
83 0.814299996693929
84 0.801500002543131
85 0.810466667016347
86 0.812966668605804
87 0.801500002543131
88 0.810466667016347
89 0.810433328151703
90 0.810466667016347
91 0.810466667016347
92 0.810466667016347
93 0.809933332602183
94 0.805166665712992
95 0.810799996058146
96 0.800199997425079
97 0.801566664377848
98 0.799500000476837
99 0.803733336925507
100 0.808066662152608
};
%\addlegendentry{DQN, n train envs=10, lr=0.00003}
\addplot [semithick, color2]
table {%
1 0.7985
100 0.7985
};
%\addlegendentry{Random}
\addplot [semithick, color3]
table {%
1 0.7685
100 0.7685
};
%\addlegendentry{ETS}
\addplot [semithick, color4]
table {%
1 0.7893
100 0.7893
};
%\addlegendentry{Heur-GD}
\addplot [semithick, color5, dash pattern=on 1pt off 3pt on 3pt off 3pt]
table {%
1 0.8081
100 0.8081
};
%\addlegendentry{Heur-LD}
\addplot [semithick, color6, dashed]
table {%
1 0.8019
100 0.8019
};
%\addlegendentry{Heur-AT}
