# Supplementary material for: Learn the Time to Learn: Replay Scheduling in Continual Learning
Source: arXiv:2209.08660 source file (2023-11-20)
Supplement: Supplementary file 22 [file rewards_env5.tex]

\nextgroupplot[title=Seed 14,
height=\figheight,
legend cell align={left},
legend style={
  fill opacity=0.8,
  draw opacity=1,
  text opacity=1,
  at={(0.5,0.09)},
  anchor=south,
  draw=white!80!black
},
minor xtick={25, 75},
minor ytick={},
tick align=outside,
tick pos=left,
width=\figwidth,
x grid style={white!69.0196078431373!black},
xlabel={Eval. Steps},
xminorgrids,
xmajorgrids,
xmin=-3.95, xmax=104.95,
xtick style={color=black},
xtick={-25,0,50,100,125},
xticklabels={-25,0,50,100,125},
y grid style={white!69.0196078431373!black},
ylabel={ACC (\%)},
ymajorgrids,
ymin=0.773365, ymax=0.873135,
ytick style={color=black},
ytick={0.76,0.78,0.8,0.82,0.84,0.86,0.88},
yticklabels={76,78,80,82,84,86,88}
]
\addplot [semithick, color0]
table {%
1 0.850099996725718
2 0.834599995613098
3 0.863500003019969
4 0.862599996725718
5 0.857299995422363
6 0.855499994754791
7 0.860233330726624
8 0.861633332570394
9 0.862033331394196
10 0.861766664187113
11 0.860233330726624
12 0.859466663996378
13 0.860899996757507
14 0.857799994945526
15 0.859466663996378
16 0.855499994754791
17 0.857299995422363
18 0.861266664663951
19 0.860599998633067
20 0.855499994754791
21 0.855499994754791
22 0.857666663328806
23 0.863200000921885
24 0.855499994754791
25 0.857666663328806
26 0.857666663328806
27 0.857666663328806
28 0.855499994754791
29 0.858433330059052
30 0.857666663328806
31 0.855499994754791
32 0.855499994754791
33 0.855499994754791
34 0.862033331394196
35 0.855499994754791
36 0.855499994754791
37 0.857666663328806
38 0.855499994754791
39 0.855499994754791
40 0.855499994754791
41 0.855499994754791
42 0.855499994754791
43 0.855499994754791
44 0.859833331902822
45 0.857666663328806
46 0.857666663328806
47 0.857666663328806
48 0.855499994754791
49 0.857666663328806
50 0.857666663328806
51 0.857666663328806
52 0.855499994754791
53 0.861266664663951
54 0.862000000476837
55 0.857666663328806
56 0.855499994754791
57 0.855499994754791
58 0.855499994754791
59 0.857666663328806
60 0.855499994754791
61 0.859833331902822
62 0.859833331902822
63 0.857666663328806
64 0.861266664663951
65 0.855499994754791
66 0.855499994754791
67 0.857666663328806
68 0.857666663328806
69 0.855499994754791
70 0.857666663328806
71 0.862000000476837
72 0.855499994754791
73 0.855499994754791
74 0.855499994754791
75 0.855499994754791
76 0.862000000476837
77 0.859833331902822
78 0.855499994754791
79 0.856633325417837
80 0.859833331902822
81 0.859833331902822
82 0.857666663328806
83 0.856633325417837
84 0.857666663328806
85 0.855499994754791
86 0.859833331902822
87 0.859833331902822
88 0.858799993991852
89 0.859833331902822
90 0.857666663328806
91 0.859833331902822
92 0.856633325417837
93 0.855933332443237
94 0.857666663328806
95 0.859833331902822
96 0.857666663328806
97 0.855499994754791
98 0.857666663328806
99 0.859833331902822
100 0.859833331902822
};
%\addlegendentry{a2c, gae, envs=10, lr=0.0003, act=tanh}
\addplot [semithick, color1]
table {%
1 0.814466667175293
2 0.849566666285197
3 0.844299999872844
4 0.843799996376038
5 0.849666666984558
6 0.848233334223429
7 0.850866667429606
8 0.845033331712087
9 0.855433336893717
10 0.84766667286555
11 0.845833337306976
12 0.84600000778834
13 0.853500000635783
14 0.845766663551331
15 0.848666659990946
16 0.856899996598562
17 0.853966669241587
18 0.838900009791056
19 0.851900001366933
20 0.853166667620341
21 0.840933338801066
22 0.850733331839243
23 0.849966661135356
24 0.841633331775665
25 0.849433334668477
26 0.845766671498617
27 0.849533331394196
28 0.854766662915548
29 0.849233337243398
30 0.853166659673055
31 0.840866669019063
32 0.848500005404154
33 0.846366671721141
34 0.848466670513153
35 0.848266673088074
36 0.845333329836528
37 0.855733331044515
38 0.85313333272934
39 0.849766663710276
40 0.83939999739329
41 0.85313333272934
42 0.848499997456869
43 0.854299994309743
44 0.845766659577687
45 0.843699995676676
46 0.845866668224335
47 0.847966663042704
48 0.848199995358785
49 0.848666659990946
50 0.848399992783864
51 0.849199994405111
52 0.846899998188019
53 0.835300004482269
54 0.846999994913737
55 0.841533327102661
56 0.846733327706655
57 0.848766668637594
58 0.843666660785675
59 0.846466660499573
60 0.849933326244354
61 0.846466660499573
62 0.850499999523163
63 0.827633333206177
64 0.844799999396006
65 0.848933327198028
66 0.834533329804738
67 0.846599996089935
68 0.847599995136261
69 0.844766660531362
70 0.841999999682108
71 0.843799996376038
72 0.832866664727529
73 0.844333326816559
74 0.846133335431417
75 0.848633337020874
76 0.840899995962779
77 0.841899995009105
78 0.842199997107188
79 0.845233333110809
80 0.844599997997284
81 0.842799993356069
82 0.854866663614909
83 0.835533328851064
84 0.849333329995473
85 0.850833336512248
86 0.841899995009105
87 0.846533330281576
88 0.847799996534983
89 0.847499998410543
90 0.852333331108093
91 0.846799997488658
92 0.857099997997284
93 0.846799997488658
94 0.844899996121725
95 0.855200000603994
96 0.847866662343343
97 0.849399995803833
98 0.846799997488658
99 0.846799997488658
100 0.846799997488658
};
%\addlegendentry{DQN, n train envs=10, lr=0.00003}
\addplot [semithick, color2]
table {%
1 0.831866666666667
100 0.831866666666667
};
%\addlegendentry{Random}
\addplot [semithick, color3]
table {%
1 0.7779
100 0.7779
};
%\addlegendentry{ETS}
\addplot [semithick, color4]
table {%
1 0.8686
100 0.8686
};
%\addlegendentry{Heur-GD}
\addplot [semithick, color5, dash pattern=on 1pt off 3pt on 3pt off 3pt]
table {%
1 0.84
100 0.84
};
%\addlegendentry{Heur-LD}
\addplot [semithick, color6, dashed]
table {%
1 0.8657
100 0.8657
};
%\addlegendentry{Heur-AT}
