# Supplementary material for: Learn the Time to Learn: Replay Scheduling in Continual Learning
Source: arXiv:2209.08660 source file (2023-11-20)
Supplement: Supplementary file 23 [file rewards_env6.tex]

\nextgroupplot[title=Seed 15,
height=\figheight,
legend cell align={left},
legend style={
  fill opacity=0.8,
  draw opacity=1,
  text opacity=1,
  at={(0.97,0.03)},
  anchor=south east,
  draw=white!80!black
},
minor xtick={25, 75},
minor ytick={},
tick align=outside,
tick pos=left,
width=\figwidth,
x grid style={white!69.0196078431373!black},
xlabel={Eval. Steps},
xminorgrids,
xmajorgrids,
xmin=-3.95, xmax=104.95,
xtick style={color=black},
xtick={-25,0,50,100,125},
xticklabels={-25,0,50,100,125},
y grid style={white!69.0196078431373!black},
ymajorgrids,
ymin=0.795768337051074, ymax=0.851465010046959,
ytick style={color=black},
ytick={0.79,0.8,0.81,0.82,0.83,0.84,0.85,0.86},
yticklabels={79,80,81,82,83,84,85,86}
]
\addplot [semithick, color0]
table {%
1 0.809100000063578
2 0.798300004005432
3 0.821366667747498
4 0.826866670449575
5 0.826533329486847
6 0.823666667938232
7 0.825433333714803
8 0.823833334445953
9 0.818466671307882
10 0.822533333301544
11 0.829399995009104
12 0.829666662216186
13 0.835233322779338
14 0.837833329041799
15 0.837299990653992
16 0.837833329041799
17 0.837299990653992
18 0.837299990653992
19 0.837299990653992
20 0.837299990653992
21 0.837299990653992
22 0.837299990653992
23 0.837299990653992
24 0.837299990653992
25 0.837299990653992
26 0.837299990653992
27 0.837299990653992
28 0.837299990653992
29 0.837299990653992
30 0.84296665986379
31 0.840133325258891
32 0.845799994468689
33 0.845799994468689
34 0.845799994468689
35 0.845799994468689
36 0.845799994468689
37 0.845799994468689
38 0.845799994468689
39 0.845799994468689
40 0.845799994468689
41 0.845799994468689
42 0.845799994468689
43 0.845799994468689
44 0.845799994468689
45 0.845799994468689
46 0.845799994468689
47 0.845799994468689
48 0.845799994468689
49 0.845799994468689
50 0.845799994468689
51 0.845799994468689
52 0.845799994468689
53 0.845799994468689
54 0.845799994468689
55 0.845799994468689
56 0.845799994468689
57 0.845799994468689
58 0.845799994468689
59 0.842599999904632
60 0.845799994468689
61 0.845799994468689
62 0.845799994468689
63 0.845799994468689
64 0.846300001939138
65 0.846300001939138
66 0.847300016880035
67 0.846300001939138
68 0.846333336830139
69 0.846300001939138
70 0.846300001939138
71 0.846699996789297
72 0.846800009409587
73 0.845866664250692
74 0.847400005658468
75 0.846333336830139
76 0.845899999141693
77 0.845899999141693
78 0.847433340549469
79 0.845866664250692
80 0.848466670513153
81 0.845899999141693
82 0.846966667970022
83 0.845866664250692
84 0.847099999586741
85 0.845899999141693
86 0.845899999141693
87 0.848933343092601
88 0.845899999141693
89 0.848466670513153
90 0.846366671721141
91 0.845899999141693
92 0.845866664250692
93 0.845899999141693
94 0.846366671721141
95 0.845899999141693
96 0.845899999141693
97 0.848466670513153
98 0.846366671721141
99 0.845899999141693
100 0.845899999141693
};
%\addlegendentry{a2c, gae, envs=10, lr=0.0003, act=tanh}
\addplot [semithick, color1]
table {%
1 0.835166668891907
2 0.847099999586741
3 0.842033330599467
4 0.839433340231578
5 0.848699998855591
6 0.848800003528595
7 0.844233330090841
8 0.846799993515015
9 0.847366670767466
10 0.840366665522258
11 0.848299996058146
12 0.844866669178009
13 0.838833336035411
14 0.841166671117147
15 0.845366664727529
16 0.844833334287008
17 0.843866662184397
18 0.839366674423218
19 0.848933343092601
20 0.846600000063578
21 0.846566673119863
22 0.845899999141693
23 0.842200001080831
24 0.845899999141693
25 0.848466670513153
26 0.847200004259745
27 0.845899999141693
28 0.833266667524974
29 0.846600000063578
30 0.8349999944369
31 0.829833332697551
32 0.833766671021779
33 0.845333337783813
34 0.826366666952769
35 0.83933333158493
36 0.831199999650319
37 0.831600002447764
38 0.837400003274282
39 0.831633329391479
40 0.837300002574921
41 0.837033335367839
42 0.826799996693929
43 0.827566667397817
44 0.830833331743876
45 0.82966666618983
46 0.822699999809265
47 0.834266670544942
48 0.833766671021779
49 0.835066672166188
50 0.83846667210261
51 0.837833333015442
52 0.825766666730245
53 0.82813333272934
54 0.831733338038127
55 0.833766671021779
56 0.833766671021779
57 0.831866669654846
58 0.84203333457311
59 0.842933332920074
60 0.838933332761129
61 0.837833329041799
62 0.837833329041799
63 0.839733330408732
64 0.839733330408732
65 0.840299999713898
66 0.837833329041799
67 0.843933335940043
68 0.839733330408732
69 0.843933335940043
70 0.839733330408732
71 0.83909999926885
72 0.84056666692098
73 0.838666665554047
74 0.839533332983653
75 0.84313333829244
76 0.84056666692098
77 0.84099999666214
78 0.840866669019063
79 0.840866669019063
80 0.841933333873749
81 0.843833335240682
82 0.841866668065389
83 0.841933333873749
84 0.844500005245209
85 0.844500005245209
86 0.844500005245209
87 0.844500005245209
88 0.844500005245209
89 0.844500005245209
90 0.844500005245209
91 0.844500005245209
92 0.844500005245209
93 0.843000002702077
94 0.841933333873749
95 0.841933333873749
96 0.843833335240682
97 0.841366676489512
98 0.83663334051768
99 0.83663334051768
100 0.834166669845581
};
%\addlegendentry{DQN, n train envs=10, lr=0.00003}
\addplot [semithick, color2]
table {%
1 0.8486
100 0.8486
};
%\addlegendentry{Random}
\addplot [semithick, color3]
table {%
1 0.8378
100 0.8378
};
%\addlegendentry{ETS}
\addplot [semithick, color4]
table {%
1 0.8352
100 0.8352
};
%\addlegendentry{Heur-GD}
\addplot [semithick, color5, dash pattern=on 1pt off 3pt on 3pt off 3pt]
table {%
1 0.8408
100 0.8408
};
%\addlegendentry{Heur-LD}
\addplot [semithick, color6, dashed]
table {%
1 0.8408
100 0.8408
};
%\addlegendentry{Heur-AT}
