# Supplementary material for: Learn the Time to Learn: Replay Scheduling in Continual Learning
Source: arXiv:2209.08660 source file (2023-11-20)
Supplement: Supplementary file 24 [file rewards_env7.tex]

\nextgroupplot[title=Seed 16,
height=\figheight,
legend cell align={left},
legend style={
  fill opacity=0.8,
  draw opacity=1,
  text opacity=1,
  at={(0.97,0.03)},
  anchor=south east,
  draw=white!80!black
},
minor xtick={25, 75},
minor ytick={},
tick align=outside,
tick pos=left,
width=\figwidth,
x grid style={white!69.0196078431373!black},
xlabel={Eval. Steps},
xminorgrids,
xmajorgrids,
xmin=-3.95, xmax=104.95,
xtick style={color=black},
xtick={-25,0,50,100,125},
xticklabels={-25,0,50,100,125},
y grid style={white!69.0196078431373!black},
ymajorgrids,
ymin=0.84, ymax=0.89,
ytick style={color=black},
ytick={0.84,0.85,0.86,0.87,0.88,0.89},
yticklabels={84,85,86,87,88,89}
]
\addplot [semithick, color0]
table {%
1 0.850666666030884
2 0.846299993991852
3 0.865166668097178
4 0.870766667524974
5 0.862966660658519
6 0.864999997615814
7 0.864999997615814
8 0.861966661612193
9 0.86256666580836
10 0.856666668256124
11 0.856666668256124
12 0.861966661612193
13 0.854866663614909
14 0.855766665935516
15 0.853433334827423
16 0.854066661993663
17 0.848399996757507
18 0.848399996757507
19 0.848399996757507
20 0.848399996757507
21 0.848399996757507
22 0.848399996757507
23 0.848399996757507
24 0.848399996757507
25 0.848399996757507
26 0.848399996757507
27 0.848399996757507
28 0.848399996757507
29 0.848399996757507
30 0.854066661993663
31 0.854066661993663
32 0.848399996757507
33 0.846200001239777
34 0.848399996757507
35 0.848399996757507
36 0.857566662629445
37 0.85043332974116
38 0.85146666765213
39 0.850299998124441
40 0.855966663360596
41 0.855700000127157
42 0.853799998760223
43 0.858633335431417
44 0.862833329041799
45 0.858899998664856
46 0.855700000127157
47 0.858633335431417
48 0.855700000127157
49 0.854100000858307
50 0.855700000127157
51 0.854100000858307
52 0.862833329041799
53 0.863999998569489
54 0.871566657225291
55 0.854100000858307
56 0.860233334700267
57 0.856433339913686
58 0.856866669654846
59 0.859800004959106
60 0.855266670385996
61 0.871566657225291
62 0.862833329041799
63 0.854100000858307
64 0.863999998569489
65 0.854100000858307
66 0.865166668097178
67 0.863999998569489
68 0.871566657225291
69 0.862833329041799
70 0.880299985408783
71 0.880299985408783
72 0.856433339913686
73 0.871566657225291
74 0.872733326752981
75 0.866333333651225
76 0.880299985408783
77 0.880299985408783
78 0.880299985408783
79 0.871566657225291
80 0.880299985408783
81 0.880299985408783
82 0.880299985408783
83 0.873899992307027
84 0.880299985408783
85 0.880299985408783
86 0.880299985408783
87 0.872733326752981
88 0.880299985408783
89 0.880299985408783
90 0.872733326752981
91 0.880299985408783
92 0.871566657225291
93 0.880299985408783
94 0.872733326752981
95 0.880299985408783
96 0.880299985408783
97 0.880299985408783
98 0.873899992307027
99 0.880299985408783
100 0.880299985408783
};
%\addlegendentry{a2c, gae, envs=10, lr=0.0003, act=tanh}
\addplot [semithick, color1]
table {%
1 0.863933332761129
2 0.873733325799306
3 0.870266664028168
4 0.864566667874654
5 0.860766669114431
6 0.878533327579498
7 0.868366666634877
8 0.869766668478648
9 0.867200005054474
10 0.862699997425079
11 0.863933332761129
12 0.864833331108093
13 0.859266670544942
14 0.864966654777527
15 0.864566663901011
16 0.862433330217997
17 0.863700000445048
18 0.865400000413259
19 0.868600006898244
20 0.873099990685781
21 0.861100002129873
22 0.876599987347921
23 0.876533321539561
24 0.880299985408783
25 0.877033325036367
26 0.871533326307933
27 0.880299985408783
28 0.874366652965546
29 0.879666654268901
30 0.879599992434184
31 0.873766664663951
32 0.877699991067251
33 0.877699991067251
34 0.87683333158493
35 0.88003333012263
36 0.880133326848348
37 0.877866657574972
38 0.88076665798823
39 0.879233316580454
40 0.872199988365173
41 0.882499996821086
42 0.878666655222575
43 0.880233323574066
44 0.881966662406921
45 0.875633331139882
46 0.87383333047231
47 0.880233323574066
48 0.880233323574066
49 0.880666661262512
50 0.880599991480509
51 0.880666661262512
52 0.878433318932851
53 0.869833330313365
54 0.880233323574066
55 0.879033323129018
56 0.878166663646698
57 0.877099998792013
58 0.878166663646698
59 0.878166663646698
60 0.876166665554047
61 0.876366670926412
62 0.880233323574066
63 0.880233323574066
64 0.880233323574066
65 0.875433337688446
66 0.877233330408732
67 0.878166663646698
68 0.878166663646698
69 0.878166663646698
70 0.877966658274333
71 0.878999996185303
72 0.874366664886475
73 0.880233323574066
74 0.880233323574066
75 0.872333339850108
76 0.87949998776118
77 0.885500001907349
78 0.880299985408783
79 0.882533331712087
80 0.881300000349681
81 0.879299994309743
82 0.877833342552185
83 0.876633338133494
84 0.872933332125346
85 0.879200005531311
86 0.877900000413259
87 0.877900000413259
88 0.876500006516774
89 0.880433336893717
90 0.880433336893717
91 0.87590000629425
92 0.880233323574066
93 0.880233323574066
94 0.882499996821086
95 0.879966660340627
96 0.878933330376943
97 0.871200009187063
98 0.879200005531311
99 0.878166663646698
100 0.876233327388763
};
%\addlegendentry{DQN, n train envs=10, lr=0.00003}
\addplot [semithick, color2]
table {%
1 0.874133333333333
100 0.874133333333333
};
%\addlegendentry{Random}
\addplot [semithick, color3]
table {%
1 0.878
100 0.878
};
%\addlegendentry{ETS}
\addplot [semithick, color4]
table {%
1 0.8677
100 0.8677
};
%\addlegendentry{Heur-GD}
\addplot [semithick, color5, dash pattern=on 1pt off 3pt on 3pt off 3pt]
table {%
1 0.8651
100 0.8651
};
%\addlegendentry{Heur-LD}
\addplot [semithick, color6, dashed]
table {%
1 0.8677
100 0.8677
};
%\addlegendentry{Heur-AT}
