# Supplementary material for: Learn the Time to Learn: Replay Scheduling in Continual Learning
Source: arXiv:2209.08660 source file (2023-11-20)
Supplement: Supplementary file 25 [file rewards_env8.tex]

\nextgroupplot[title=Seed 17,
height=\figheight,
legend cell align={left},
legend style={
  fill opacity=0.8,
  draw opacity=1,
  text opacity=1,
  at={(0.5,0.09)},
  anchor=south,
  draw=white!80!black
},
minor xtick={25, 75},
minor ytick={},
tick align=outside,
tick pos=left,
width=\figwidth,
x grid style={white!69.0196078431373!black},
xlabel={Eval. Steps},
xminorgrids,
xmajorgrids,
xmin=-3.95, xmax=104.95,
xtick style={color=black},
xtick={-25,0,50,100,125},
xticklabels={-25,0,50,100,125},
y grid style={white!69.0196078431373!black},
ymajorgrids,
ymin=0.699, ymax=0.775004995894432,
ytick style={color=black},
ytick={0.7,0.71,0.72,0.73,0.74,0.75,0.76,0.77,0.78},
yticklabels={70,71,72,73,74,75,76,77,78}
]
\addplot [semithick, color0]
table {%
1 0.758266663551331
2 0.739199995994568
3 0.770433326562246
4 0.755733335018158
5 0.752833338578542
6 0.748066679636637
7 0.74850001335144
8 0.74850001335144
9 0.755066672960917
10 0.746466676394145
11 0.746466676394145
12 0.74850001335144
13 0.746466676394145
14 0.747333335876465
15 0.754300006230672
16 0.757200002670288
17 0.754300006230672
18 0.757200002670288
19 0.759533333778381
20 0.758366668224335
21 0.758366668224335
22 0.761366665363312
23 0.758366668224335
24 0.758366668224335
25 0.758366668224335
26 0.759533333778381
27 0.758366668224335
28 0.757200002670288
29 0.760066668192546
30 0.758366668224335
31 0.757200002670288
32 0.757200002670288
33 0.757200002670288
34 0.757200002670288
35 0.757200002670288
36 0.757200002670288
37 0.757200002670288
38 0.757200002670288
39 0.757200002670288
40 0.757200002670288
41 0.757200002670288
42 0.757200002670288
43 0.757200002670288
44 0.757200002670288
45 0.757200002670288
46 0.757200002670288
47 0.757200002670288
48 0.757200002670288
49 0.757200002670288
50 0.757200002670288
51 0.757200002670288
52 0.757200002670288
53 0.757200002670288
54 0.757200002670288
55 0.757200002670288
56 0.757200002670288
57 0.757200002670288
58 0.757200002670288
59 0.757200002670288
60 0.757200002670288
61 0.757200002670288
62 0.757200002670288
63 0.757200002670288
64 0.757200002670288
65 0.757200002670288
66 0.757200002670288
67 0.757200002670288
68 0.757200002670288
69 0.757200002670288
70 0.757200002670288
71 0.757200002670288
72 0.757200002670288
73 0.757200002670288
74 0.757200002670288
75 0.757200002670288
76 0.757200002670288
77 0.757200002670288
78 0.757200002670288
79 0.757200002670288
80 0.757200002670288
81 0.757200002670288
82 0.757200002670288
83 0.757200002670288
84 0.757200002670288
85 0.757200002670288
86 0.757200002670288
87 0.757200002670288
88 0.757200002670288
89 0.757200002670288
90 0.757200002670288
91 0.757200002670288
92 0.757200002670288
93 0.757200002670288
94 0.757200002670288
95 0.757200002670288
96 0.757200002670288
97 0.757200002670288
98 0.757200002670288
99 0.757200002670288
100 0.757200002670288
};
%\addlegendentry{a2c, gae, envs=10, lr=0.0003, act=tanh}
\addplot [semithick, color1]
table {%
1 0.739199995994568
2 0.739199995994568
3 0.740900003910065
4 0.742899998029073
5 0.749633328119914
6 0.760200003782908
7 0.759233331680298
8 0.76046667098999
9 0.762933333714803
10 0.770799998442332
11 0.762133340040843
12 0.76593333085378
13 0.771599996089935
14 0.762833333015442
15 0.75343333085378
16 0.749766663710276
17 0.755633330345154
18 0.755633330345154
19 0.756299996376038
20 0.763533329963684
21 0.759166661898295
22 0.761566662788391
23 0.757866668701172
24 0.760033337275187
25 0.749000000953674
26 0.758699997266134
27 0.760800000031789
28 0.763899993896484
29 0.763633334636688
30 0.761433327198029
31 0.758699997266134
32 0.765966665744782
33 0.761033328374227
34 0.766366664568583
35 0.768833331267039
36 0.765966665744782
37 0.766500000158946
38 0.768699995676676
39 0.765966665744782
40 0.766500000158946
41 0.766500000158946
42 0.750666666030884
43 0.750666666030884
44 0.765733337402344
45 0.728600001335144
46 0.766366664568583
47 0.758166662851969
48 0.750033338864644
49 0.750033338864644
50 0.75753333568573
51 0.741033331553141
52 0.728600001335144
53 0.728600001335144
54 0.748533328374227
55 0.748533328374227
56 0.743300000826518
57 0.748533328374227
58 0.748533328374227
59 0.75753333568573
60 0.748533328374227
61 0.750033338864644
62 0.75753333568573
63 0.7442999958992
64 0.758166662851969
65 0.760599998633067
66 0.750666666030884
67 0.738166670004527
68 0.73566666841507
69 0.734933336575826
70 0.735966662565867
71 0.738399998346965
72 0.737666670481364
73 0.735333335399628
74 0.760599998633067
75 0.738299997647603
76 0.73566666841507
77 0.733333333333333
78 0.739333327611288
79 0.735966662565867
80 0.735966662565867
81 0.738399998346965
82 0.738399998346965
83 0.738399998346965
84 0.741599996884664
85 0.740033336480459
86 0.735333335399628
87 0.756933331489563
88 0.736366665363312
89 0.735333335399628
90 0.735966662565867
91 0.733399999141693
92 0.751600003242493
93 0.735333335399628
94 0.758700001239777
95 0.756300004323323
96 0.754033331076304
97 0.735333335399628
98 0.762799998124441
99 0.751600003242493
100 0.751600003242493
};
%\addlegendentry{DQN, n train envs=10, lr=0.00003}
\addplot [semithick, color2]
table {%
1 0.7168
100 0.7168
};
%\addlegendentry{Random}
\addplot [semithick, color3]
table {%
1 0.7035
100 0.7035
};
%\addlegendentry{ETS}
\addplot [semithick, color4]
table {%
1 0.7414
100 0.7414
};
%\addlegendentry{Heur-GD}
\addplot [semithick, color5, dash pattern=on 1pt off 3pt on 3pt off 3pt]
table {%
1 0.7608
100 0.7608
};
%\addlegendentry{Heur-LD}
\addplot [semithick, color6, dashed]
table {%
1 0.7644
100 0.7644
};
%\addlegendentry{Heur-AT}
