# Supplementary material for: Learn the Time to Learn: Replay Scheduling in Continual Learning
Source: arXiv:2209.08660 source file (2023-11-20)
Supplement: Supplementary file 26 [file rewards_env9.tex]

\nextgroupplot[title=Seed 18,
height=\figheight,
legend cell align={left},
legend style={
  fill opacity=0.8,
  draw opacity=1,
  text opacity=1,
  at={(0.03,0.03)},
  anchor=south west,
  draw=white!80!black
},
minor xtick={25, 75},
minor ytick={},
tick align=outside,
tick pos=left,
width=\figwidth,
x grid style={white!69.0196078431373!black},
xlabel={Eval. Steps},
xminorgrids,
xmajorgrids,
xmin=-3.95, xmax=104.95,
xtick style={color=black},
xtick={-25,0,50,100,125},
xticklabels={-25,0,50,100,125},
y grid style={white!69.0196078431373!black},
ylabel={ACC (\%)},
ymajorgrids,
ymin=0.867104990553856, ymax=0.899995000449816,
ytick style={color=black},
ytick={0.87,0.88,0.89,0.9,0.91},
yticklabels={87,88,89,90,91}
]
\addplot [semithick, color0]
table {%
1 0.883633327484131
2 0.874599993228912
3 0.891466665267944
4 0.887800006071726
5 0.888266666730245
6 0.887933337688446
7 0.891700001557668
8 0.896366663773855
9 0.89546666542689
10 0.895799994468689
11 0.895799994468689
12 0.896366663773855
13 0.895799994468689
14 0.896366663773855
15 0.895799994468689
16 0.895799994468689
17 0.895799994468689
18 0.895799994468689
19 0.895799994468689
20 0.895799994468689
21 0.895799994468689
22 0.895799994468689
23 0.895799994468689
24 0.895799994468689
25 0.895799994468689
26 0.895799994468689
27 0.895166663328807
28 0.895166663328807
29 0.894733329614004
30 0.894533332188924
31 0.895166663328807
32 0.894533332188924
33 0.894533332188924
34 0.893900001049042
35 0.894533332188924
36 0.893900001049042
37 0.893900001049042
38 0.893900001049042
39 0.893900001049042
40 0.893900001049042
41 0.893900001049042
42 0.894533332188924
43 0.893900001049042
44 0.893900001049042
45 0.893900001049042
46 0.893900001049042
47 0.894533332188924
48 0.893900001049042
49 0.893900001049042
50 0.893900001049042
51 0.893900001049042
52 0.893900001049042
53 0.893900001049042
54 0.893900001049042
55 0.893900001049042
56 0.893900001049042
57 0.893900001049042
58 0.893900001049042
59 0.893900001049042
60 0.893900001049042
61 0.893900001049042
62 0.893900001049042
63 0.893900001049042
64 0.895600001017253
65 0.893900001049042
66 0.893900001049042
67 0.893900001049042
68 0.893900001049042
69 0.893900001049042
70 0.893900001049042
71 0.895600001017253
72 0.893900001049042
73 0.893900001049042
74 0.893900001049042
75 0.893900001049042
76 0.893900001049042
77 0.893900001049042
78 0.893900001049042
79 0.893900001049042
80 0.893900001049042
81 0.893900001049042
82 0.895600001017253
83 0.893900001049042
84 0.893900001049042
85 0.893900001049042
86 0.897300000985463
87 0.895600001017253
88 0.895600001017253
89 0.895600001017253
90 0.893266665935516
91 0.895600001017253
92 0.895600001017253
93 0.895600001017253
94 0.895600001017253
95 0.894966665903727
96 0.893266665935516
97 0.895600001017253
98 0.897300000985463
99 0.897300000985463
100 0.893266665935516
};
%\addlegendentry{a2c, gae, envs=10, lr=0.0003, act=tanh}
\addplot [semithick, color1]
table {%
1 0.87653333346049
2 0.885633333524068
3 0.888966671625773
4 0.89406666358312
5 0.88590000073115
6 0.895766667524974
7 0.883733332157135
8 0.893966666857402
9 0.892666669686635
10 0.890233337879181
11 0.895899991194407
12 0.887200005849202
13 0.886033336321513
14 0.890966661771139
15 0.885500005880992
16 0.888766670227051
17 0.88953332901001
18 0.880000003178914
19 0.891633335749308
20 0.886400000254313
21 0.891166671117147
22 0.891200002034505
23 0.886100002129873
24 0.880466663837433
25 0.888633334636688
26 0.88720000187556
27 0.880033334096273
28 0.888633334636688
29 0.885566663742065
30 0.882100001970927
31 0.88736666838328
32 0.885133337974548
33 0.887666670481364
34 0.883266671498617
35 0.891133332252502
36 0.887833333015442
37 0.881233330567678
38 0.884299997488658
39 0.891966664791107
40 0.887800002098084
41 0.887000000476837
42 0.881733330090841
43 0.891500000158946
44 0.883666666348775
45 0.894399996598562
46 0.88756666580836
47 0.880333332220713
48 0.891266663869222
49 0.883433330059051
50 0.891266663869222
51 0.883599996566772
52 0.880533329645793
53 0.887166670958201
54 0.880700000127157
55 0.880700000127157
56 0.880700000127157
57 0.880333332220713
58 0.880333332220713
59 0.88756666580836
60 0.882366673151652
61 0.884299997488658
62 0.880333332220713
63 0.884200000762939
64 0.884033338228861
65 0.875799997647603
66 0.883100001017253
67 0.88479999701182
68 0.878366661071777
69 0.877533336480459
70 0.884200000762939
71 0.881166672706604
72 0.878366661071777
73 0.878366661071777
74 0.877366673946381
75 0.885333335399628
76 0.873799999554952
77 0.881466662883759
78 0.876666665077209
79 0.875266667207082
80 0.875566665331523
81 0.87186666727066
82 0.868599991003672
83 0.869999992847443
84 0.869999992847443
85 0.875566665331523
86 0.880733338991801
87 0.8753666639328
88 0.880899997552236
89 0.880366671085358
90 0.877300004164378
91 0.884366663297017
92 0.880366671085358
93 0.877900000413259
94 0.87256666024526
95 0.871066657702128
96 0.871666665871938
97 0.872599999109904
98 0.879266663392385
99 0.888700000445048
100 0.881766664981842
};
%\addlegendentry{DQN, n train envs=10, lr=0.00003}
\addplot [semithick, color2]
table {%
1 0.869733333333333
100 0.869733333333333
};
%\addlegendentry{Random}
\addplot [semithick, color3]
table {%
1 0.8832
100 0.8832
};
%\addlegendentry{ETS}
\addplot [semithick, color4]
table {%
1 0.8859
100 0.8859
};
%\addlegendentry{Heur-GD}
\addplot [semithick, color5, dash pattern=on 1pt off 3pt on 3pt off 3pt]
table {%
1 0.8985
100 0.8985
};
%\addlegendentry{Heur-LD}
\addplot [semithick, color6, dashed]
table {%
1 0.8859
100 0.8859
};
%\addlegendentry{Heur-AT}
