# Supplementary material for: Learn the Time to Learn: Replay Scheduling in Continual Learning
Source: arXiv:2209.08660 source file (2023-11-20)
Supplement: Supplementary file 27 [file groupplot.tex]

\pgfplotsset{every axis title/.append style={at={(0.5,0.85)}}}
\pgfplotsset{every tick label/.append style={font=\scriptsize}}
\pgfplotsset{every major tick/.append style={major tick length=2pt}}
\pgfplotsset{every minor tick/.append style={minor tick length=1pt}}
\pgfplotsset{every axis x label/.append style={at={(0.5,-0.22)}}}
\pgfplotsset{every axis y label/.append style={at={(-0.30,0.5)}}}
% [inline block 0: 1 envs, 56162 chars -> data_tex | \begin{tikzpicture} \tikzstyle{every node}=[font=\scriptsize]...]
