# Supplementary material for: Learn the Time to Learn: Replay Scheduling in Continual Learning
Source: arXiv:2209.08660 source file (2023-11-20)
Supplement: Supplementary file 28 [file rewards_env1.tex]

\nextgroupplot[title=Seed 0,
height=\figheight,
legend cell align={left},
legend columns=-1,
legend style={
  fill opacity=0.8,
  draw opacity=1,
  text opacity=1,
  at={(0.10,1.29)},
  anchor=south west,
  draw=white!80!black
},
minor xtick={25, 75},
minor ytick={},
tick align=outside,
tick pos=left,
width=\figwidth,
x grid style={white!69.0196078431373!black},
xlabel={Eval. Steps},
xminorgrids,
xmajorgrids,
xmin=-3.95, xmax=104.95,
xtick style={color=black},
xtick={-25,0,50,100,125},
xticklabels={-25,0,50,100,125},
y grid style={white!69.0196078431373!black},
ylabel={ACC (\%)},
ymajorgrids,
ymin=0.88, ymax=0.982,
ytick style={color=black},
ytick={0.88,0.9,0.92,0.94,0.96,0.98,1},
yticklabels={88,90,92,94,96,98,100}
]
\addplot [semithick, color0]
table {%
1 0.973199999332428
2 0.974833333492279
3 0.974899995326996
4 0.97279999256134
5 0.945633323987325
6 0.921266663074494
7 0.919900000095367
8 0.895533335208893
9 0.922833335399628
10 0.89553333123525
11 0.895500000317891
12 0.89559999704361
13 0.894133329391479
14 0.89559999704361
15 0.895566666126251
16 0.895566666126251
17 0.895566666126251
18 0.892666661739349
19 0.895566666126251
20 0.894099998474121
21 0.89559999704361
22 0.894133329391479
23 0.894133329391479
24 0.894133329391479
25 0.894133329391479
26 0.894133329391479
27 0.892666661739349
28 0.894133329391479
29 0.919866661230723
30 0.894133329391479
31 0.945733328660329
32 0.918299996852875
33 0.918399993578593
34 0.921399998664856
35 0.9471333305041
36 0.918466663360596
37 0.919933331012726
38 0.919866661230723
39 0.944266661008199
40 0.944333330790202
41 0.944266661008199
42 0.944333330790202
43 0.972933328151703
44 0.971766666571299
45 0.974466669559479
46 0.972933332125346
47 0.971366663773855
48 0.944099994500478
49 0.970066658655802
50 0.975933337211609
51 0.972999997933706
52 0.970066658655802
53 0.974166667461395
54 0.945500000317891
55 0.971533330281575
56 0.947200000286102
57 0.971466660499573
58 0.947200000286102
59 0.970066658655802
60 0.946166662375132
61 0.972866662343343
62 0.972933332125346
63 0.974466669559479
64 0.974333329995473
65 0.975633335113525
66 0.971533330281575
67 0.973000001907348
68 0.916566665967305
69 0.97279999256134
70 0.972866662343343
71 0.975866667429606
72 0.947200000286102
73 0.972833335399628
74 0.974333333969116
75 0.974333333969116
76 0.972699995835622
77 0.970066658655802
78 0.972866662343343
79 0.975666666030884
80 0.947766673564911
81 0.974466669559479
82 0.974466669559479
83 0.972999997933706
84 0.94693333307902
85 0.974333333969116
86 0.974300003051758
87 0.975766670703888
88 0.974466669559479
89 0.972266666094462
90 0.971533330281575
91 0.975633335113525
92 0.975933337211609
93 0.975633335113525
94 0.945566666126251
95 0.976966667175293
96 0.975800001621246
97 0.973433331648509
98 0.948666663964589
99 0.975666666030884
100 0.94706666469574
};
\addlegendentry{A2C}
\addplot [semithick, color1]
table {%
1 0.972600003083547
2 0.932433334986369
3 0.960266665617625
4 0.923233338197072
5 0.973600002129873
6 0.974799998601278
7 0.9189333319664
8 0.918400005499522
9 0.91906666358312
10 0.945900003115336
11 0.971166670322418
12 0.973633333047231
13 0.975266663233439
14 0.947366666793823
15 0.923400004704793
16 0.943766673405965
17 0.973533340295156
18 0.945166671276093
19 0.923500001430511
20 0.973933327198028
21 0.945633331934611
22 0.973733329772949
23 0.945600001017253
24 0.946366671721141
25 0.973266661167145
26 0.946000003814697
27 0.947766669591268
28 0.891600000858307
29 0.94686666727066
30 0.891633331775665
31 0.943099999427795
32 0.946166666348775
33 0.944733329614003
34 0.890733329455058
35 0.891733336448669
36 0.914899996916453
37 0.945933334032695
38 0.977599998315175
39 0.888966663678487
40 0.9185666680336
41 0.934566668669383
42 0.918400001525879
43 0.916133332252502
44 0.946566665172577
45 0.88933333158493
46 0.972533337275187
47 0.920333337783814
48 0.972900001207987
49 0.917733339468638
50 0.917866663138072
51 0.919433331489563
52 0.971200001239777
53 0.914999997615814
54 0.889400001366933
55 0.946033330758413
56 0.917900002002716
57 0.918899997075399
58 0.947300000985464
59 0.919599997997284
60 0.888899997870127
61 0.890233333905538
62 0.944533336162567
63 0.94706666469574
64 0.942100004355113
65 0.947233331203461
66 0.945133336385091
67 0.919933331012726
68 0.973066667715708
69 0.969099994500478
70 0.919099998474121
71 0.919099998474121
72 0.948099998633067
73 0.976933332284292
74 0.944000005722046
75 0.976133330663045
76 0.934266666571299
77 0.948299996058146
78 0.948166664441426
79 0.927799999713898
80 0.975766666730245
81 0.963433329264323
82 0.948800003528595
83 0.948299992084503
84 0.918499998251597
85 0.940799995263418
86 0.950999995072683
87 0.976266662279765
88 0.974766667683919
89 0.94729999701182
90 0.946600000063578
91 0.94613333940506
92 0.947366666793823
93 0.948233326276143
94 0.964299992720286
95 0.975899990399678
96 0.976266662279765
97 0.948233326276143
98 0.946666657924652
99 0.971599996089935
100 0.97543332974116
};
\addlegendentry{DQN}
\addplot [semithick, color2]
table {%
1 0.946366666666667
100 0.946366666666667
};
\addlegendentry{Random}
\addplot [semithick, color3]
table {%
1 0.971
100 0.971
};
\addlegendentry{ETS}
\addplot [semithick, color4]
table {%
1 0.979
100 0.979
};
\addlegendentry{Heur-GD}
\addplot [semithick, color5, dash pattern=on 1pt off 3pt on 3pt off 3pt]
table {%
1 0.9759
100 0.9759
};
\addlegendentry{Heur-LD}
\addplot [semithick, color6, dashed]
table {%
1 0.9741
100 0.9741
};
\addlegendentry{Heur-AT}
