# Supplementary material for: Learn the Time to Learn: Replay Scheduling in Continual Learning
Source: arXiv:2209.08660 source file (2023-11-20)
Supplement: Supplementary file 29 [file rewards_env10.tex]

\nextgroupplot[title=Seed 9,
height=\figheight,
legend cell align={left},
legend style={
  fill opacity=0.8,
  draw opacity=1,
  text opacity=1,
  at={(0.5,0.91)},
  anchor=north,
  draw=white!80!black
},
minor xtick={25, 75},
minor ytick={},
tick align=outside,
tick pos=left,
width=\figwidth,
x grid style={white!69.0196078431373!black},
xlabel={Eval. Steps},
xminorgrids,
xmajorgrids,
xmin=-3.95, xmax=104.95,
xtick style={color=black},
xtick={-25,0,50,100,125},
xticklabels={-25,0,50,100,125},
y grid style={white!69.0196078431373!black},
ymajorgrids,
ymin=0.889279995059967, ymax=0.98,
ytick style={color=black},
ytick={0.88,0.9,0.92,0.94,0.96,0.98},
yticklabels={88,90,92,94,96,98}
]
\addplot [semithick, color0]
table {%
1 0.94449999332428
2 0.95056666135788
3 0.917299997806549
4 0.914699995517731
5 0.902766660849253
6 0.933133327960968
7 0.933133327960968
8 0.939966662724813
9 0.925566665331523
10 0.929666662216187
11 0.91936666170756
12 0.904299998283386
13 0.904299998283386
14 0.904299998283386
15 0.9221333305041
16 0.9221333305041
17 0.939966662724813
18 0.89516666730245
19 0.898033332824707
20 0.9221333305041
21 0.904299998283386
22 0.904299998283386
23 0.904299998283386
24 0.898033332824707
25 0.904299998283386
26 0.898033332824707
27 0.898033332824707
28 0.898033332824707
29 0.904299998283386
30 0.904299998283386
31 0.904299998283386
32 0.898033332824707
33 0.904299998283386
34 0.904299998283386
35 0.898033332824707
36 0.904299998283386
37 0.899533327420552
38 0.904299998283386
39 0.904299998283386
40 0.898033332824707
41 0.904299998283386
42 0.893266661961873
43 0.904299998283386
44 0.904299998283386
45 0.904299998283386
46 0.904299998283386
47 0.904299998283386
48 0.904299998283386
49 0.904299998283386
50 0.904299998283386
51 0.904299998283386
52 0.904299998283386
53 0.904299998283386
54 0.904299998283386
55 0.904299998283386
56 0.904299998283386
57 0.904299998283386
58 0.904299998283386
59 0.904299998283386
60 0.904299998283386
61 0.904299998283386
62 0.904299998283386
63 0.904299998283386
64 0.904299998283386
65 0.904299998283386
66 0.904299998283386
67 0.904299998283386
68 0.904299998283386
69 0.904299998283386
70 0.904299998283386
71 0.904299998283386
72 0.904299998283386
73 0.904299998283386
74 0.904299998283386
75 0.904299998283386
76 0.904299998283386
77 0.904299998283386
78 0.904299998283386
79 0.904299998283386
80 0.904299998283386
81 0.904299998283386
82 0.904299998283386
83 0.904299998283386
84 0.904299998283386
85 0.904299998283386
86 0.904299998283386
87 0.904299998283386
88 0.904299998283386
89 0.904299998283386
90 0.904299998283386
91 0.904299998283386
92 0.904299998283386
93 0.904299998283386
94 0.904299998283386
95 0.911633332570394
96 0.904299998283386
97 0.904299998283386
98 0.904299998283386
99 0.904299998283386
100 0.911633332570394
};
%\addlegendentry{a2c, gae, envs=10, lr=0.0003, act=tanh}
\addplot [semithick, color1]
table {%
1 0.921499999364217
2 0.93506666024526
3 0.948166664441426
4 0.926099991798401
5 0.935066668192546
6 0.949166659514109
7 0.932433327039083
8 0.970266675949097
9 0.961166671911875
10 0.967199997107188
11 0.944033332665761
12 0.972833331425985
13 0.942299997806549
14 0.938566664854685
15 0.942966655890147
16 0.942166662216187
17 0.904133323828379
18 0.945999995867411
19 0.913666665554047
20 0.906133329868317
21 0.949299995104472
22 0.920733332633972
23 0.963966655731201
24 0.957366661230723
25 0.958799993991852
26 0.926366666952769
27 0.961699994405111
28 0.961366669336955
29 0.963899997870127
30 0.918666668732961
31 0.922300000985463
32 0.958633335431417
33 0.956299996376038
34 0.946833332379659
35 0.938366667429606
36 0.931699995199839
37 0.955200000603994
38 0.937466661135356
39 0.916633335749308
40 0.94283332824707
41 0.919699994723002
42 0.924333333969116
43 0.912799994150797
44 0.942533334096273
45 0.946099996566772
46 0.935499993960063
47 0.938499999046326
48 0.916999999682109
49 0.933266667524974
50 0.955699992179871
51 0.939299996693929
52 0.92960000038147
53 0.951266662279765
54 0.948366665840149
55 0.932000001271566
56 0.941633327802022
57 0.940266664822896
58 0.909233331680298
59 0.93566666841507
60 0.943066664536794
61 0.957133324940999
62 0.941066658496857
63 0.951933336257934
64 0.94706666469574
65 0.939433332284291
66 0.9246333360672
67 0.945233337084452
68 0.934666665395101
69 0.931433327992757
70 0.938433337211609
71 0.920500004291534
72 0.946366667747498
73 0.938933336734772
74 0.955033334096273
75 0.938499999046326
76 0.953533327579498
77 0.961133329073588
78 0.922599999109904
79 0.920166663328807
80 0.957799998919169
81 0.927099998792012
82 0.948866665363312
83 0.932533331712087
84 0.89883333047231
85 0.922233339150747
86 0.939733334382375
87 0.954999999205271
88 0.938366663455963
89 0.946866671244303
90 0.938933336734772
91 0.939300000667572
92 0.946666665871938
93 0.941399999459585
94 0.953966665267944
95 0.921233328183492
96 0.949600001176198
97 0.94686666727066
98 0.949466665585836
99 0.942700000603994
100 0.954933329423269
};
%\addlegendentry{DQN, n train envs=30}
\addplot [semithick, color2]
table {%
1 0.973
100 0.973
};
%\addlegendentry{Random}
\addplot [semithick, color3]
table {%
1 0.9671
100 0.9671
};
%\addlegendentry{ETS}
\addplot [semithick, color4]
table {%
1 0.9527
100 0.9527
};
%\addlegendentry{Heur-GD}
\addplot [semithick, color5, dash pattern=on 1pt off 3pt on 3pt off 3pt]
table {%
1 0.9002
100 0.9002
};
%\addlegendentry{Heur-LD}
\addplot [semithick, color6, dashed]
table {%
1 0.9029
100 0.9029
};
%\addlegendentry{Heur-AT}
