# Supplementary material for: Learn the Time to Learn: Replay Scheduling in Continual Learning
Source: arXiv:2209.08660 source file (2023-11-20)
Supplement: Supplementary file 30 [file rewards_env2.tex]

\nextgroupplot[title=Seed 1,
height=\figheight,
legend cell align={left},
legend style={
  fill opacity=0.8,
  draw opacity=1,
  text opacity=1,
  at={(0.97,0.03)},
  anchor=south east,
  draw=white!80!black
},
minor xtick={25, 75},
minor ytick={},
tick align=outside,
tick pos=left,
width=\figwidth,
x grid style={white!69.0196078431373!black},
xlabel={Eval. Steps},
xminorgrids,
xmajorgrids,
xmin=-3.95, xmax=104.95,
xtick style={color=black},
xtick={-25,0,50,100,125},
xticklabels={-25,0,50,100,125},
y grid style={white!69.0196078431373!black},
ymajorgrids,
ymin=0.854905004700025, ymax=0.962595010399818,
ytick style={color=black},
ytick={0.84,0.86,0.88,0.9,0.92,0.94,0.96,0.98},
yticklabels={84,86,88,90,92,94,96,98}
]
\addplot [semithick, color0]
table {%
1 0.924066670735677
2 0.911366661389669
3 0.938500006993612
4 0.941500008106232
5 0.945533339182536
6 0.943866674105326
7 0.947966674963633
8 0.95060000816981
9 0.951466675599416
10 0.947033341725667
11 0.947033341725667
12 0.951000010967255
13 0.951333343982697
14 0.951000010967255
15 0.951000010967255
16 0.951000010967255
17 0.950800009568532
18 0.955333344141642
19 0.951000010967255
20 0.951666676998138
21 0.945600012938182
22 0.952300012111664
23 0.949600013097127
24 0.9550000111262
25 0.951266678174337
26 0.957700010140737
27 0.930266670385997
28 0.945333341757456
29 0.918533333142598
30 0.94900000890096
31 0.926099995772044
32 0.919266664981842
33 0.942000007629395
34 0.905199992656708
35 0.93100000222524
36 0.920233333110809
37 0.919999996821086
38 0.93100000222524
39 0.919999996821086
40 0.931233338514964
41 0.916199998060862
42 0.931466674804687
43 0.931233338514964
44 0.920233333110809
45 0.931233338514964
46 0.920233333110809
47 0.930466667811076
48 0.942466680208842
49 0.931233338514964
50 0.942700016498566
51 0.931466674804687
52 0.931466666857402
53 0.942700016498566
54 0.942466680208842
55 0.930466667811076
56 0.942700016498566
57 0.942466680208842
58 0.94270000855128
59 0.930466667811076
60 0.920233333110809
61 0.930466667811076
62 0.920233325163523
63 0.931466674804687
64 0.931466674804687
65 0.931466674804687
66 0.941700009504954
67 0.941700009504954
68 0.920233333110809
69 0.941700009504954
70 0.931466674804687
71 0.942700016498566
72 0.942700016498566
73 0.930466667811076
74 0.941700009504954
75 0.930100007851919
76 0.941700009504954
77 0.930466667811076
78 0.930466667811076
79 0.930466667811076
80 0.930100007851919
81 0.930466667811076
82 0.941700009504954
83 0.930466667811076
84 0.940700002511342
85 0.941700009504954
86 0.941700009504954
87 0.929466660817464
88 0.939699995517731
89 0.930466667811076
90 0.940700002511342
91 0.929466660817464
92 0.939699995517731
93 0.930466667811076
94 0.919233326117198
95 0.929466660817464
96 0.929466660817464
97 0.920233333110809
98 0.920233333110809
99 0.941700009504954
100 0.919233326117198
};
%\addlegendentry{a2c, gae, envs=10, lr=0.0003, act=tanh}
\addplot [semithick, color1]
table {%
1 0.900799989700317
2 0.912233340740204
3 0.91263333161672
4 0.928866664568583
5 0.908866663773855
6 0.90889999071757
7 0.927533332506816
8 0.891566665967305
9 0.899466673533122
10 0.914566667874654
11 0.937033327420553
12 0.910133334000905
13 0.914766669273376
14 0.907233341534933
15 0.934766670068105
16 0.927966666221618
17 0.921366663773855
18 0.93866666952769
19 0.940600005785624
20 0.939800004164378
21 0.89859999815623
22 0.936033336321513
23 0.93260000149409
24 0.941900006930033
25 0.944600009918213
26 0.859800004959106
27 0.941400003433227
28 0.924700001875559
29 0.941266667842865
30 0.921700004736583
31 0.888233335812887
32 0.931266665458679
33 0.904833336671193
34 0.930966671307882
35 0.895066666603088
36 0.925733335812887
37 0.894133337338765
38 0.911666671435038
39 0.931633329391479
40 0.922200004259745
41 0.9121333360672
42 0.938533333937327
43 0.909999998410543
44 0.90293333530426
45 0.9064333319664
46 0.916133332252502
47 0.922466667493184
48 0.922466667493184
49 0.922466667493184
50 0.916199998060862
51 0.933999999364217
52 0.937000000476837
53 0.893700003623962
54 0.920366668701172
55 0.940266664822896
56 0.906733334064484
57 0.932999996344248
58 0.943666660785675
59 0.923433331648509
60 0.940099994341532
61 0.929866659641266
62 0.941633331775665
63 0.94883333047231
64 0.89816666841507
65 0.925533334414164
66 0.905799996852875
67 0.896833332379659
68 0.890966665744782
69 0.927433335781097
70 0.943099999427795
71 0.941200006008148
72 0.922533329327901
73 0.94256667693456
74 0.913033334414164
75 0.942700012524923
76 0.94699999888738
77 0.938700000445048
78 0.936299999554952
79 0.914599998792013
80 0.915766664346059
81 0.908499999841054
82 0.927266673247019
83 0.927900008360545
84 0.928466665744781
85 0.920866676171621
86 0.928833325703939
87 0.928266668319702
88 0.921433333555857
89 0.933300006389618
90 0.932666671276093
91 0.928233337402344
92 0.928266668319702
93 0.928233337402344
94 0.891733336448669
95 0.913099996248881
96 0.913099996248881
97 0.927066663901011
98 0.927466662724813
99 0.929166666666667
100 0.929166666666667
};
%\addlegendentry{DQN, n train envs=30}
\addplot [semithick, color2]
table {%
1 0.938733333333333
100 0.938733333333333
};
%\addlegendentry{Random}
\addplot [semithick, color3]
table {%
1 0.941
100 0.941
};
%\addlegendentry{ETS}
\addplot [semithick, color4]
table {%
1 0.9501
100 0.9501
};
%\addlegendentry{Heur-GD}
\addplot [semithick, color5, dash pattern=on 1pt off 3pt on 3pt off 3pt]
table {%
1 0.9003
100 0.9003
};
%\addlegendentry{Heur-LD}
\addplot [semithick, color6, dashed]
table {%
1 0.9409
100 0.9409
};
%\addlegendentry{Heur-AT}
