# Supplementary material for: Learn the Time to Learn: Replay Scheduling in Continual Learning
Source: arXiv:2209.08660 source file (2023-11-20)
Supplement: Supplementary file 31 [file rewards_env3.tex]

\nextgroupplot[title=Seed 2,
height=\figheight,
legend cell align={left},
legend style={
  fill opacity=0.8,
  draw opacity=1,
  text opacity=1,
  at={(0.5,0.09)},
  anchor=south,
  draw=white!80!black
},
minor xtick={25, 75},
minor ytick={},
tick align=outside,
tick pos=left,
width=\figwidth,
x grid style={white!69.0196078431373!black},
xlabel={Eval. Steps},
xminorgrids,
xmajorgrids,
xmin=-3.95, xmax=104.95,
xtick style={color=black},
xtick={-25,0,50,100,125},
xticklabels={-25,0,50,100,125},
y grid style={white!69.0196078431373!black},
ymajorgrids,
ymin=0.86, ymax=0.982280000700951,
ytick style={color=black},
ytick={0.86,0.88,0.9,0.92,0.94,0.96,0.98,1},
yticklabels={86,88,90,92,94,96,98,100}
]
\addplot [semithick, color0]
table {%
1 0.968699999650319
2 0.962933333714803
3 0.966999999682109
4 0.976800000667572
5 0.975900002320607
6 0.946600004037221
7 0.954800005753835
8 0.941700005531311
9 0.95563333829244
10 0.948633337020874
11 0.948633337020874
12 0.962100005149841
13 0.966700005531311
14 0.962100005149841
15 0.951900005340576
16 0.951900005340576
17 0.941700005531311
18 0.971300005912781
19 0.951900005340576
20 0.956500005722046
21 0.962100005149841
22 0.966700005531311
23 0.966700005531311
24 0.966700005531311
25 0.966700005531311
26 0.962100005149841
27 0.971300005912781
28 0.962100005149841
29 0.962100005149841
30 0.966700005531311
31 0.966700005531311
32 0.968866670131683
33 0.971300005912781
34 0.962100005149841
35 0.962100005149841
36 0.966700005531311
37 0.966700005531311
38 0.966700005531311
39 0.966700005531311
40 0.971300005912781
41 0.971300005912781
42 0.971300005912781
43 0.971300005912781
44 0.971300005912781
45 0.966700005531311
46 0.962100005149841
47 0.966700005531311
48 0.966700005531311
49 0.966700005531311
50 0.976200004418691
51 0.971300005912781
52 0.966700005531311
53 0.966700005531311
54 0.966700005531311
55 0.966700005531311
56 0.966700005531311
57 0.962100005149841
58 0.966700005531311
59 0.971300005912781
60 0.961833333969116
61 0.971300005912781
62 0.962100005149841
63 0.966700005531311
64 0.97590000629425
65 0.966700005531311
66 0.966700005531311
67 0.962100005149841
68 0.968866670131683
69 0.966700005531311
70 0.971300005912781
71 0.971300005912781
72 0.971300005912781
73 0.959666669368744
74 0.966700005531311
75 0.966700005531311
76 0.962100005149841
77 0.971300005912781
78 0.971300005912781
79 0.966700005531311
80 0.962100005149841
81 0.966700005531311
82 0.966700005531311
83 0.971300005912781
84 0.97590000629425
85 0.966700005531311
86 0.971300005912781
87 0.968866670131683
88 0.966700005531311
89 0.968866670131683
90 0.971300005912781
91 0.961833333969116
92 0.967000003655751
93 0.971300005912781
94 0.964266669750213
95 0.971300005912781
96 0.966700005531311
97 0.957233333587647
98 0.97590000629425
99 0.976200004418691
100 0.971300005912781
};
%\addlegendentry{a2c, gae, envs=10, lr=0.0003, act=tanh}
\addplot [semithick, color1]
table {%
1 0.964833335081736
2 0.916833341121674
3 0.928633340199788
4 0.961433331171672
5 0.957066663106283
6 0.952766672770182
7 0.967800001303355
8 0.9682000041008
9 0.96850000222524
10 0.949233333269755
11 0.940300003687541
12 0.967266670862834
13 0.964433344205221
14 0.967666661739349
15 0.972566668192546
16 0.95956666469574
17 0.946899998188019
18 0.970433338483175
19 0.969000005722046
20 0.965500005086263
21 0.970399995644887
22 0.971033334732056
23 0.962599996725718
24 0.969533336162567
25 0.963700004418691
26 0.96476666132609
27 0.964900008837382
28 0.971666665871938
29 0.964833335081736
30 0.970566662152608
31 0.967666669686635
32 0.965733329455058
33 0.965533343950908
34 0.965066667397817
35 0.966233332951864
36 0.964233338832855
37 0.958200001716614
38 0.956566667556763
39 0.956566667556763
40 0.957133336861928
41 0.957833337783813
42 0.962600004673004
43 0.937933341662089
44 0.959266666571299
45 0.936633344491323
46 0.9367666721344
47 0.940500005086263
48 0.969966673851013
49 0.941133340199788
50 0.9396333416303
51 0.93956667582194
52 0.968733334541321
53 0.966900010903676
54 0.951666673024495
55 0.936633344491323
56 0.959866678714752
57 0.959366675217946
58 0.96756667693456
59 0.929033346970876
60 0.970699997742971
61 0.966700005531311
62 0.928800006707509
63 0.967066669464111
64 0.95930001338323
65 0.970100009441376
66 0.962866671880086
67 0.964533336957296
68 0.96996666987737
69 0.932900007565816
70 0.93343334197998
71 0.931833338737488
72 0.970100009441376
73 0.923100010553996
74 0.968666672706604
75 0.968666672706604
76 0.972133338451385
77 0.938133343060811
78 0.93343334197998
79 0.971733339627584
80 0.936700002352397
81 0.934000007311503
82 0.934000007311503
83 0.939833343029022
84 0.936733337243398
85 0.959000007311503
86 0.969633332888285
87 0.954600012302399
88 0.96366666952769
89 0.948300004005432
90 0.965166668097178
91 0.945866668224335
92 0.958700009187063
93 0.958833340803782
94 0.952500009536743
95 0.959833331902822
96 0.959566672643026
97 0.953933338324229
98 0.95586667060852
99 0.96346667210261
100 0.956200007597605
};
%\addlegendentry{DQN, n train envs=30}
\addplot [semithick, color2]
table {%
1 0.948566666666667
100 0.948566666666667
};
%\addlegendentry{Random}
\addplot [semithick, color3]
table {%
1 0.8672
100 0.8672
};
%\addlegendentry{ETS}
\addplot [semithick, color4]
table {%
1 0.9741
100 0.9741
};
%\addlegendentry{Heur-GD}
\addplot [semithick, color5, dash pattern=on 1pt off 3pt on 3pt off 3pt]
table {%
1 0.973
100 0.973
};
%\addlegendentry{Heur-LD}
\addplot [semithick, color6, dashed]
table {%
1 0.9765
100 0.9765
};
%\addlegendentry{Heur-AT}
