# Supplementary material for: Learn the Time to Learn: Replay Scheduling in Continual Learning
Source: arXiv:2209.08660 source file (2023-11-20)
Supplement: Supplementary file 32 [file rewards_env4.tex]

\nextgroupplot[title=Seed 3,
height=\figheight,
legend cell align={left},
legend style={
  fill opacity=0.8,
  draw opacity=1,
  text opacity=1,
  at={(0.97,0.03)},
  anchor=south east,
  draw=white!80!black
},
minor xtick={25, 75},
minor ytick={},
tick align=outside,
tick pos=left,
width=\figwidth,
x grid style={white!69.0196078431373!black},
xlabel={Eval. Steps},
xminorgrids,
xmajorgrids,
xmin=-3.95, xmax=104.95,
xtick style={color=black},
xtick={-25,0,50,100,125},
xticklabels={-25,0,50,100,125},
y grid style={white!69.0196078431373!black},
ymajorgrids,
ymin=0.86, ymax=1.0,
ytick style={color=black},
ytick={0.86,0.88,0.9,0.92,0.94,0.96,0.98,1,1.02},
yticklabels={86,88,90,92,94,96,98,100,102}
]
\addplot [semithick, color0]
table {%
1 0.980333340167999
2 0.950200005372365
3 0.956466670831044
4 0.986600005626678
5 0.987900006771088
6 0.972866674264272
7 0.985166668891907
8 0.966766675313314
9 0.973800007502238
10 0.961633336544037
11 0.96603334347407
12 0.968300008773804
13 0.967600003878275
14 0.968300008773804
15 0.968300008773804
16 0.968300008773804
17 0.967533342043559
18 0.966899998982747
19 0.968300008773804
20 0.967600003878275
21 0.954633339246114
22 0.967600003878275
23 0.974566674232483
24 0.967600003878275
25 0.967600003878275
26 0.958633331457774
27 0.966199994087219
28 0.953933334350586
29 0.949666659037272
30 0.947833335399628
31 0.946966660022736
32 0.978600001335144
33 0.975499999523163
34 0.941399991512299
35 0.956466662883758
36 0.964899996916453
37 0.973533336321513
38 0.952166660626729
39 0.969333330790202
40 0.987766675154368
41 0.973000001907349
42 0.987100005149841
43 0.959233327706655
44 0.96739999850591
45 0.973000001907349
46 0.958299998442332
47 0.982033332188924
48 0.98823333978653
49 0.950499999523163
50 0.98663334051768
51 0.955300001303355
52 0.964166669050852
53 0.962733340263367
54 0.973433335622152
55 0.94050000111262
56 0.932833329836527
57 0.973000001907349
58 0.923499997456868
59 0.952766664822896
60 0.947366670767466
61 0.980600003401438
62 0.954866667588552
63 0.951933332284292
64 0.923499997456868
65 0.92513333161672
66 0.938533325990041
67 0.966666662693024
68 0.978133340676626
69 0.935366666316986
70 0.922500002384186
71 0.984433337052663
72 0.984433337052663
73 0.93609999815623
74 0.920133328437805
75 0.921466668446859
76 0.9035666624705
77 0.926433332761129
78 0.938766666253408
79 0.925633339087168
80 0.964633333683014
81 0.969333330790202
82 0.935366666316986
83 0.984566668669383
84 0.97806666692098
85 0.952766664822896
86 0.951033333937327
87 0.934666665395101
88 0.932833329836527
89 0.96660000483195
90 0.950033334891001
91 0.97806666692098
92 0.984566668669383
93 0.952766664822896
94 0.981466666857401
95 0.950300002098084
96 0.956466670831044
97 0.948666663964589
98 0.936233329772949
99 0.952766664822896
100 0.904933329423269
};
%\addlegendentry{a2c, gae, envs=10, lr=0.0003, act=tanh}
\addplot [semithick, color1]
table {%
1 0.95220000743866
2 0.936033324400584
3 0.956433335940043
4 0.94633332490921
5 0.914999993642171
6 0.86746666431427
7 0.938133331139882
8 0.932800006866455
9 0.97186666727066
10 0.921766662597656
11 0.889733330408732
12 0.948099994659424
13 0.949033339818319
14 0.953600005308787
15 0.928133328755697
16 0.978533335526784
17 0.911299999554952
18 0.945233333110809
19 0.932133344809214
20 0.946733331680298
21 0.935400001207987
22 0.943466663360596
23 0.976699999968211
24 0.984266670544942
25 0.898866665363312
26 0.940299995740255
27 0.957833337783814
28 0.984366671244303
29 0.960033333301544
30 0.951299997170766
31 0.909833335876465
32 0.952366662025452
33 0.968433332443237
34 0.988400002320608
35 0.952900004386902
36 0.980666673183441
37 0.985866661866506
38 0.984766662120819
39 0.969666667779287
40 0.945433330535889
41 0.969866669178009
42 0.985866657892863
43 0.970033327738444
44 0.991133332252502
45 0.984700004259745
46 0.989666672547658
47 0.985766657193502
48 0.983566665649414
49 0.98449999888738
50 0.942466668287913
51 0.9521333416303
52 0.968733326594035
53 0.979999999205271
54 0.98063333829244
55 0.976333324114482
56 0.949266672134399
57 0.977566679318746
58 0.966600008805593
59 0.971533334255218
60 0.976300005118052
61 0.981966666380564
62 0.980866662661235
63 0.978666671117147
64 0.979500007629394
65 0.980366663138072
66 0.985233334700267
67 0.941033327579498
68 0.987266671657562
69 0.983400007088979
70 0.962699993451436
71 0.973699998855591
72 0.988599995772044
73 0.944933338960012
74 0.973499997456869
75 0.973233338197072
76 0.980566668510437
77 0.971033338705699
78 0.982233337561289
79 0.957433338960012
80 0.983299998442332
81 0.983433326085409
82 0.948199995358785
83 0.987400003274282
84 0.980033342043559
85 0.960199999809265
86 0.981033329168956
87 0.954533330599467
88 0.982366673151652
89 0.951699992020925
90 0.976433328787486
91 0.983166666825612
92 0.965666667620341
93 0.976099995772044
94 0.96586666504542
95 0.985700007279714
96 0.979633327325185
97 0.972033337752024
98 0.974866664409637
99 0.965400000413259
100 0.966266663869222
};
%\addlegendentry{DQN, n train envs=30}
\addplot [semithick, color2]
table {%
1 0.942533333333333
100 0.942533333333333
};
%\addlegendentry{Random}
\addplot [semithick, color3]
table {%
1 0.8944
100 0.8944
};
%\addlegendentry{ETS}
\addplot [semithick, color4]
table {%
1 0.9669
100 0.9669
};
%\addlegendentry{Heur-GD}
\addplot [semithick, color5, dash pattern=on 1pt off 3pt on 3pt off 3pt]
table {%
1 0.9061
100 0.9061
};
%\addlegendentry{Heur-LD}
\addplot [semithick, color6, dashed]
table {%
1 0.994
100 0.994
};
%\addlegendentry{Heur-AT}
