# Supplementary material for: Learn the Time to Learn: Replay Scheduling in Continual Learning
Source: arXiv:2209.08660 source file (2023-11-20)
Supplement: Supplementary file 33 [file rewards_env5.tex]

\nextgroupplot[title=Seed 4,
height=\figheight,
legend cell align={left},
legend style={
  fill opacity=0.8,
  draw opacity=1,
  text opacity=1,
  at={(0.97,0.03)},
  anchor=south east,
  draw=white!80!black
},
minor xtick={25, 75},
minor ytick={0.775, 0.825, 0.875, 0.925, 0.975},
tick align=outside,
tick pos=left,
width=\figwidth,
x grid style={white!69.0196078431373!black},
xlabel={Eval. Steps},
xminorgrids,
xmajorgrids,
xmin=-3.95, xmax=104.95,
xtick style={color=black},
xtick={-25,0,50,100,125},
xticklabels={-25,0,50,100,125},
y grid style={white!69.0196078431373!black},
ylabel={ACC (\%)},
yminorgrids,
ymajorgrids,
ymin=0.75, ymax=0.929473329186439,
ytick style={color=black},
ytick={0.75,0.8,0.85,0.9,0.95},
yticklabels={75,80,85,90,95}
]
\addplot [semithick, color0]
table {%
1 0.887033331394195
2 0.921599996089935
3 0.841399999459585
4 0.817900002002716
5 0.816366664568583
6 0.817900002002716
7 0.817900002002716
8 0.818933343887329
9 0.838766674200694
10 0.818933343887329
11 0.82370001077652
12 0.82370001077652
13 0.82370001077652
14 0.82370001077652
15 0.82370001077652
16 0.81456667582194
17 0.81456667582194
18 0.827233334382375
19 0.81456667582194
20 0.80543334086736
21 0.80543334086736
22 0.788333336512248
23 0.788333336512248
24 0.822333343823751
25 0.788333336512248
26 0.780366667111715
27 0.764133334159851
28 0.780366667111715
29 0.772399997711182
30 0.772399997711182
31 0.772399997711182
32 0.772399997711182
33 0.772399997711182
34 0.772399997711182
35 0.772399997711182
36 0.772399997711182
37 0.772399997711182
38 0.772399997711182
39 0.772399997711182
40 0.764133334159851
41 0.776766665776571
42 0.772399997711182
43 0.809866666793823
44 0.772399997711182
45 0.772399997711182
46 0.772399997711182
47 0.772399997711182
48 0.772399997711182
49 0.772399997711182
50 0.772399997711182
51 0.772399997711182
52 0.809866666793823
53 0.809866666793823
54 0.847333335876465
55 0.809866666793823
56 0.859700000286102
57 0.847333335876465
58 0.884800004959107
59 0.772399997711182
60 0.848766664663951
61 0.859700000286102
62 0.847333335876465
63 0.897166669368744
64 0.859700000286102
65 0.893100003401438
66 0.809866666793823
67 0.847333335876465
68 0.900033326943715
69 0.884800004959107
70 0.897166669368744
71 0.818166665236155
72 0.909533333778381
73 0.847333335876465
74 0.884800004959107
75 0.847333335876465
76 0.884800004959107
77 0.896000003814697
78 0.884800004959107
79 0.897166669368744
80 0.884800004959107
81 0.897166669368744
82 0.884800004959107
83 0.847333335876465
84 0.908366668224335
85 0.908366668224335
86 0.858533334732056
87 0.858533334732056
88 0.896000003814697
89 0.908366668224335
90 0.897166669368744
91 0.897166669368744
92 0.896000003814697
93 0.907200002670288
94 0.896000003814697
95 0.896000003814697
96 0.896000003814697
97 0.907200002670288
98 0.907200002670288
99 0.907200002670288
100 0.918400001525879
};
%\addlegendentry{a2c, gae, envs=10, lr=0.0003, act=tanh}
\addplot [semithick, color1]
table {%
1 0.846366675694783
2 0.82970001300176
3 0.896766662597656
4 0.855066665013631
5 0.828266676266988
6 0.89239999850591
7 0.863933340708415
8 0.903566666444143
9 0.909766662120819
10 0.90049999554952
11 0.907333330313365
12 0.914799996217092
13 0.862166663010915
14 0.8903666694959
15 0.860133322079976
16 0.877999997138977
17 0.91010000705719
18 0.899700001875559
19 0.864866665999095
20 0.859866666793823
21 0.915699990590413
22 0.873133333524068
23 0.903799998760223
24 0.861900003751119
25 0.874233337243398
26 0.865033336480459
27 0.868933335940043
28 0.892633338769277
29 0.864699999491374
30 0.840733329455058
31 0.904566665490468
32 0.90760000149409
33 0.90760000149409
34 0.913533329963684
35 0.905266670385997
36 0.909099996089935
37 0.908133327960968
38 0.897999997933706
39 0.903566670417786
40 0.901566668351491
41 0.908133327960968
42 0.907366669178009
43 0.90349999666214
44 0.87103332678477
45 0.909599995613098
46 0.913766666253408
47 0.901166665554047
48 0.910699995358785
49 0.904899994532267
50 0.876166665554047
51 0.876166665554047
52 0.8714333375295
53 0.904899994532267
54 0.913800001144409
55 0.900999999046326
56 0.900999999046326
57 0.89833333492279
58 0.909499994913737
59 0.879266667366028
60 0.88156666358312
61 0.87096666097641
62 0.913800001144409
63 0.903033336003621
64 0.903033336003621
65 0.903033336003621
66 0.880733331044515
67 0.905366663138072
68 0.866466661294301
69 0.917933324972788
70 0.911533331871033
71 0.908533334732056
72 0.904899994532267
73 0.909866666793823
74 0.885966670513153
75 0.904899994532267
76 0.874033335844676
77 0.883600000540416
78 0.88156666358312
79 0.887633323669434
80 0.881600002447764
81 0.882233325640361
82 0.876166665554047
83 0.884100000063578
84 0.873233326276143
85 0.876166665554047
86 0.876166665554047
87 0.876166665554047
88 0.876166665554047
89 0.875700000921885
90 0.868933335940043
91 0.902900000413259
92 0.902900000413259
93 0.865700002511342
94 0.873033332824707
95 0.873033332824707
96 0.873033332824707
97 0.873033332824707
98 0.875066669782003
99 0.865900003910065
100 0.913366663455963
};
%\addlegendentry{DQN, n train envs=30}
\addplot [semithick, color2]
table {%
1 0.844933333333333
100 0.844933333333333
};
%\addlegendentry{Random}
\addplot [semithick, color3]
table {%
1 0.8707
100 0.8707
};
%\addlegendentry{ETS}
\addplot [semithick, color4]
table {%
1 0.9129
100 0.9129
};
%\addlegendentry{Heur-GD}
\addplot [semithick, color5, dash pattern=on 1pt off 3pt on 3pt off 3pt]
table {%
1 0.8675
100 0.8675
};
%\addlegendentry{Heur-LD}
\addplot [semithick, color6, dashed]
table {%
1 0.8328
100 0.8328
};
%\addlegendentry{Heur-AT}
