# Supplementary material for: Learn the Time to Learn: Replay Scheduling in Continual Learning
Source: arXiv:2209.08660 source file (2023-11-20)
Supplement: Supplementary file 34 [file rewards_env6.tex]

\nextgroupplot[title=Seed 5,
height=\figheight,
legend cell align={left},
legend style={fill opacity=0.8, draw opacity=1, text opacity=1, draw=white!80!black},
minor xtick={25, 75},
minor ytick={},
tick align=outside,
tick pos=left,
width=\figwidth,
x grid style={white!69.0196078431373!black},
xlabel={Eval. Steps},
xminorgrids,
xmajorgrids,
xmin=-3.95, xmax=104.95,
xtick style={color=black},
xtick={-25,0,50,100,125},
xticklabels={-25,0,50,100,125},
y grid style={white!69.0196078431373!black},
ymajorgrids,
ymin=0.835075005292892, ymax=0.933891669511795,
ytick style={color=black},
ytick={0.82,0.84,0.86,0.88,0.9,0.92,0.94},
yticklabels={82,84,86,88,90,92,94}
]
\addplot [semithick, color0]
table {%
1 0.896133335431417
2 0.900733331839244
3 0.875399990876516
4 0.882933330535889
5 0.879633335272471
6 0.897400001684825
7 0.903033332029978
8 0.894133337338766
9 0.899766671657562
10 0.901766665776571
11 0.897766665617625
12 0.902133329709371
13 0.913400002320607
14 0.901766665776571
15 0.913400002320607
16 0.902133329709371
17 0.90140000184377
18 0.908866671721141
19 0.919033332665761
20 0.919033332665761
21 0.909800004959107
22 0.899500000476837
23 0.911766672134399
24 0.913400002320607
25 0.92940000295639
26 0.92940000295639
27 0.867966667811076
28 0.890799999237061
29 0.868899997075399
30 0.869633336861928
31 0.868899997075399
32 0.868899997075399
33 0.868899997075399
34 0.868899997075399
35 0.87316666841507
36 0.868899997075399
37 0.868899997075399
38 0.868899997075399
39 0.874099997679393
40 0.879299998283386
41 0.879299998283386
42 0.879299998283386
43 0.874099997679393
44 0.874099997679393
45 0.879299998283386
46 0.878599997361501
47 0.879299998283386
48 0.879299998283386
49 0.879299998283386
50 0.879299998283386
51 0.879299998283386
52 0.879299998283386
53 0.879299998283386
54 0.879299998283386
55 0.879299998283386
56 0.879299998283386
57 0.879299998283386
58 0.879299998283386
59 0.879299998283386
60 0.879299998283386
61 0.879299998283386
62 0.879299998283386
63 0.879299998283386
64 0.879299998283386
65 0.879299998283386
66 0.879299998283386
67 0.879299998283386
68 0.879299998283386
69 0.879299998283386
70 0.879299998283386
71 0.879299998283386
72 0.879299998283386
73 0.879299998283386
74 0.879299998283386
75 0.879299998283386
76 0.879299998283386
77 0.879299998283386
78 0.879299998283386
79 0.879299998283386
80 0.879299998283386
81 0.879299998283386
82 0.879299998283386
83 0.879299998283386
84 0.879299998283386
85 0.879299998283386
86 0.879299998283386
87 0.879299998283386
88 0.879299998283386
89 0.879299998283386
90 0.879299998283386
91 0.879299998283386
92 0.879299998283386
93 0.879299998283386
94 0.879299998283386
95 0.879299998283386
96 0.879299998283386
97 0.879299998283386
98 0.879299998283386
99 0.879299998283386
100 0.879299998283386
};
%\addlegendentry{a2c, gae, envs=10, lr=0.0003, act=tanh}
\addplot [semithick, color1]
table {%
1 0.915700006484986
2 0.886466666062673
3 0.907866664727529
4 0.893233338991801
5 0.881733334064484
6 0.890699998537699
7 0.914533332983653
8 0.879299998283386
9 0.893000002702077
10 0.877300000190735
11 0.904433329900106
12 0.870966668923696
13 0.861199998855591
14 0.882633336385091
15 0.903100001811981
16 0.881400005022685
17 0.897333339850108
18 0.881166664759318
19 0.897599991162618
20 0.877733333905538
21 0.911433331171672
22 0.878733336925507
23 0.878866664568583
24 0.86176666021347
25 0.847333327929179
26 0.839566671848297
27 0.856599998474121
28 0.853766659895579
29 0.879199997584025
30 0.89773332675298
31 0.866033331553141
32 0.878533327579498
33 0.875599996248881
34 0.843799996376038
35 0.91109999815623
36 0.885766665140788
37 0.862899998823802
38 0.876433324813843
39 0.866033327579498
40 0.848900000254313
41 0.84743332862854
42 0.857499992847443
43 0.857499992847443
44 0.84980000257492
45 0.895199990272522
46 0.872833331425985
47 0.858699997266134
48 0.870566666126251
49 0.876499994595846
50 0.901333336035411
51 0.86503332455953
52 0.880499998728434
53 0.879399995009104
54 0.86520000298818
55 0.842633326848348
56 0.873333326975504
57 0.87229999701182
58 0.882966661453247
59 0.889366654555003
60 0.875733323891958
61 0.891266655921936
62 0.851433324813843
63 0.850700000921885
64 0.884533333778381
65 0.88296666542689
66 0.870333329836527
67 0.920566670099894
68 0.877299996217092
69 0.904666674137116
70 0.865833334128062
71 0.85256667137146
72 0.87530001004537
73 0.865833334128062
74 0.881433335940043
75 0.873766664663951
76 0.862133328119914
77 0.885666660467784
78 0.879399991035461
79 0.863266658782959
80 0.857033336162567
81 0.842266662915548
82 0.896600004037221
83 0.886966669559479
84 0.853266668319702
85 0.867799993356069
86 0.885266661643982
87 0.894799995422363
88 0.866699993610382
89 0.843166661262512
90 0.898700002829234
91 0.88303333123525
92 0.912533326943715
93 0.906366662184397
94 0.857533331712087
95 0.8807000041008
96 0.859266666571299
97 0.888566668828328
98 0.87659999926885
99 0.883433334032694
100 0.874700005849202
};
%\addlegendentry{DQN, n train envs=30}
\addplot [semithick, color2]
table {%
1 0.901833333333333
100 0.901833333333333
};
%\addlegendentry{Random}
\addplot [semithick, color3]
table {%
1 0.9153
100 0.9153
};
%\addlegendentry{ETS}
\addplot [semithick, color4]
table {%
1 0.9033
100 0.9033
};
%\addlegendentry{Heur-GD}
\addplot [semithick, color5, dash pattern=on 1pt off 3pt on 3pt off 3pt]
table {%
1 0.8801
100 0.8801
};
%\addlegendentry{Heur-LD}
\addplot [semithick, color6, dashed]
table {%
1 0.9053
100 0.9053
};
%\addlegendentry{Heur-AT}
