# Supplementary material for: Learn the Time to Learn: Replay Scheduling in Continual Learning
Source: arXiv:2209.08660 source file (2023-11-20)
Supplement: Supplementary file 35 [file rewards_env7.tex]

\nextgroupplot[title=Seed 6,
height=\figheight,
legend cell align={left},
legend style={
  fill opacity=0.8,
  draw opacity=1,
  text opacity=1,
  at={(0.5,0.91)},
  anchor=north,
  draw=white!80!black
},
minor xtick={25, 75},
minor ytick={0.775, 0.825, 0.875, 0.925, 0.975},
tick align=outside,
tick pos=left,
width=\figwidth,
x grid style={white!69.0196078431373!black},
xlabel={Eval. Steps},
xminorgrids,
xmajorgrids,
xmin=-3.95, xmax=104.95,
xtick style={color=black},
xtick={-25,0,50,100,125},
xticklabels={-25,0,50,100,125},
y grid style={white!69.0196078431373!black},
yminorgrids,
ymajorgrids,
ymin=0.75047, ymax=0.96453,
ytick style={color=black},
ytick={0.75,0.8,0.85,0.9,0.95,0.975},
yticklabels={75,80,85,90,95,975}
]
\addplot [semithick, color0]
table {%
1 0.912899998823802
2 0.907566662629445
3 0.927833330631256
4 0.933099997043609
5 0.915600001811981
6 0.933099997043609
7 0.915600001811981
8 0.92199999888738
9 0.912899994850159
10 0.92199999888738
11 0.9182000041008
12 0.9182000041008
13 0.863533333937327
14 0.9182000041008
15 0.9182000041008
16 0.92316666841507
17 0.870333333810171
18 0.808866663773855
19 0.8653666694959
20 0.8653666694959
21 0.812533334891001
22 0.777799999713898
23 0.777799999713898
24 0.8653666694959
25 0.779633335272471
26 0.779633335272471
27 0.79956667025884
28 0.79956667025884
29 0.819500005245209
30 0.797733334700267
31 0.797733334700267
32 0.797733334700267
33 0.819500005245209
34 0.819500005245209
35 0.819500005245209
36 0.819500005245209
37 0.819500005245209
38 0.819500005245209
39 0.819500005245209
40 0.819500005245209
41 0.797733334700267
42 0.819500005245209
43 0.819500005245209
44 0.819500005245209
45 0.819500005245209
46 0.819500005245209
47 0.819500005245209
48 0.819500005245209
49 0.819500005245209
50 0.819500005245209
51 0.819500005245209
52 0.819500005245209
53 0.819500005245209
54 0.819500005245209
55 0.819500005245209
56 0.819500005245209
57 0.819500005245209
58 0.861299995581309
59 0.819500005245209
60 0.819500005245209
61 0.819500005245209
62 0.819500005245209
63 0.819500005245209
64 0.819500005245209
65 0.850366667906443
66 0.819500005245209
67 0.819500005245209
68 0.852033332983653
69 0.819500005245209
70 0.824133336544037
71 0.819500005245209
72 0.914799992243449
73 0.800233336289724
74 0.881233330567678
75 0.847100003560384
76 0.852033332983653
77 0.852033332983653
78 0.850366667906443
79 0.850366667906443
80 0.852033332983653
81 0.913766658306122
82 0.882899995644887
83 0.85140000184377
84 0.850366667906443
85 0.850299998124441
86 0.850366667906443
87 0.847266670068105
88 0.85196666320165
89 0.850366667906443
90 0.894999996821086
91 0.862466669082642
92 0.862399999300639
93 0.879099996884664
94 0.85196666320165
95 0.910033329327901
96 0.847200000286102
97 0.893266661961873
98 0.8471333305041
99 0.879799997806549
100 0.883866659800212
};
%\addlegendentry{a2c, gae, envs=10, lr=0.0003, act=tanh}
\addplot [semithick, color1]
table {%
1 0.905266670385997
2 0.864233334859212
3 0.810099999109904
4 0.839866662025452
5 0.885899996757507
6 0.876900005340576
7 0.765333326657613
8 0.874233333269755
9 0.885866665840149
10 0.794099994500478
11 0.765233329931895
12 0.886333334445953
13 0.813366663455963
14 0.820233333110809
15 0.80789999961853
16 0.815499989191691
17 0.82433332602183
18 0.88896666765213
19 0.841799994309743
20 0.869766668478648
21 0.896999994913737
22 0.854566665490468
23 0.787966664632161
24 0.834399998188019
25 0.780200000603994
26 0.843666664759318
27 0.826933332284292
28 0.815366665522257
29 0.844133337338765
30 0.869633332888285
31 0.83806666135788
32 0.798933331171672
33 0.872233331203461
34 0.827833330631256
35 0.805966663360596
36 0.838566664854686
37 0.805966663360596
38 0.872966659069061
39 0.872966659069061
40 0.872966659069061
41 0.866699993610382
42 0.861866664886474
43 0.851199992497762
44 0.810466659069061
45 0.810433328151703
46 0.860266657670339
47 0.81146666208903
48 0.790466662247976
49 0.851266658306122
50 0.810433328151703
51 0.790466662247976
52 0.851199992497762
53 0.810433328151703
54 0.810433328151703
55 0.819299991925557
56 0.822200000286102
57 0.841799994309743
58 0.851199992497762
59 0.790466662247976
60 0.79933332602183
61 0.79933332602183
62 0.822200000286102
63 0.801233327388763
64 0.810433328151703
65 0.848233326276143
66 0.810433328151703
67 0.810433328151703
68 0.822200000286102
69 0.822200000286102
70 0.780799992879232
71 0.810433328151703
72 0.790466662247976
73 0.812266663710276
74 0.790466662247976
75 0.856033329168956
76 0.822200000286102
77 0.801599995295207
78 0.780799992879232
79 0.803066662947337
80 0.812999999523163
81 0.810433328151703
82 0.856033329168956
83 0.83506666024526
84 0.812266663710276
85 0.815099994341532
86 0.846499995390574
87 0.84609999259313
88 0.848933323224386
89 0.819299991925557
90 0.821133327484131
91 0.835833326975504
92 0.821899994214376
93 0.850833328564962
94 0.820066658655802
95 0.820066658655802
96 0.820066658655802
97 0.79953332344691
98 0.834266658624013
99 0.781566659609477
100 0.820066658655802
};
%\addlegendentry{DQN, n train envs=30}
\addplot [semithick, color2]
table {%
1 0.9521
100 0.9521
};
%\addlegendentry{Random}
\addplot [semithick, color3]
table {%
1 0.9548
100 0.9548
};
%\addlegendentry{ETS}
\addplot [semithick, color4]
table {%
1 0.9001
100 0.9001
};
%\addlegendentry{Heur-GD}
\addplot [semithick, color5, dash pattern=on 1pt off 3pt on 3pt off 3pt]
table {%
1 0.8544
100 0.8544
};
%\addlegendentry{Heur-LD}
\addplot [semithick, color6, dashed]
table {%
1 0.7602
100 0.7602
};
%\addlegendentry{Heur-AT}
