# Supplementary material for: Learn the Time to Learn: Replay Scheduling in Continual Learning
Source: arXiv:2209.08660 source file (2023-11-20)
Supplement: Supplementary file 36 [file rewards_env8.tex]

\nextgroupplot[title=Seed 7,
height=\figheight,
legend cell align={left},
legend style={
  fill opacity=0.8,
  draw opacity=1,
  text opacity=1,
  at={(0.5,0.91)},
  anchor=north,
  draw=white!80!black
},
minor xtick={25, 75},
minor ytick={},
tick align=outside,
tick pos=left,
width=\figwidth,
x grid style={white!69.0196078431373!black},
xlabel={Eval. Steps},
xminorgrids,
xmajorgrids,
xmin=-3.95, xmax=104.95,
xtick style={color=black},
xtick={-25,0,50,100,125},
xticklabels={-25,0,50,100,125},
y grid style={white!69.0196078431373!black},
ymajorgrids,
ymin=0.869310013518333, ymax=0.97248999935627,
ytick style={color=black},
ytick={0.86,0.88,0.9,0.92,0.94,0.96,0.98},
yticklabels={86,88,90,92,94,96,98}
]
\addplot [semithick, color0]
table {%
1 0.909533333778381
2 0.887866671880086
3 0.901666657129923
4 0.896099984645844
5 0.911366657416026
6 0.902299996217092
7 0.912266663710276
8 0.904799997806549
9 0.922599995136261
10 0.902833330631256
11 0.897599991162618
12 0.903599989414215
13 0.914599990844727
14 0.903599989414215
15 0.903599989414215
16 0.904199993610382
17 0.904199993610382
18 0.925599992275238
19 0.903599989414215
20 0.914599990844727
21 0.903599989414215
22 0.914599990844727
23 0.914599990844727
24 0.914599990844727
25 0.914599990844727
26 0.903599989414215
27 0.925599992275238
28 0.914599990844727
29 0.903599989414215
30 0.914599990844727
31 0.91636666059494
32 0.914833331108093
33 0.914366662502289
34 0.903599989414215
35 0.901099987824758
36 0.925599992275238
37 0.924599993228913
38 0.903366661071777
39 0.927633333206177
40 0.936933334668477
41 0.917666665712992
42 0.93633333047231
43 0.921199997266134
44 0.916133332252502
45 0.929499991734823
46 0.913899997870127
47 0.937899998823802
48 0.922433332602183
49 0.922433332602183
50 0.939066668351491
51 0.932266660531362
52 0.92940000295639
53 0.91453332901001
54 0.918766657511393
55 0.91329999367396
56 0.94056666692098
57 0.896099984645844
58 0.937466661135356
59 0.934933336575826
60 0.924833337465922
61 0.927033332983653
62 0.918233335018158
63 0.914266661802928
64 0.929300010204315
65 0.935366674264272
66 0.918366662661235
67 0.915566658973694
68 0.904533330599467
69 0.918233335018158
70 0.925699996948242
71 0.925200005372365
72 0.935533340771993
73 0.923566671212514
74 0.914100003242493
75 0.930166669686635
76 0.915700002511342
77 0.927900008360545
78 0.94140000740687
79 0.92916667064031
80 0.905900001525879
81 0.92756667137146
82 0.915700002511342
83 0.939466679096222
84 0.91023333867391
85 0.933700001239777
86 0.91023333867391
87 0.925500007470449
88 0.926233335336049
89 0.935433332125346
90 0.918200008074443
91 0.926166673501333
92 0.92370001077652
93 0.946266678969065
94 0.906400001049042
95 0.940300003687541
96 0.921400006612142
97 0.918366670608521
98 0.920500008265177
99 0.91506667137146
100 0.930266674359639
};
%\addlegendentry{a2c, gae, envs=10, lr=0.0003, act=tanh}
\addplot [semithick, color1]
table {%
1 0.902333335081736
2 0.898600002129873
3 0.9307000041008
4 0.912566673755646
5 0.904633339246114
6 0.923466662565867
7 0.932333330313365
8 0.920666666825612
9 0.894333338737488
10 0.934666665395101
11 0.912433342138926
12 0.926133326689402
13 0.930133334795634
14 0.938799997170766
15 0.919200007120768
16 0.941533335049947
17 0.925666670004527
18 0.942866663138072
19 0.896266667048136
20 0.928333330154419
21 0.922333335876465
22 0.929733331998189
23 0.916333333651225
24 0.931600006421407
25 0.927733341852824
26 0.929666670163472
27 0.937333329518636
28 0.935533332824707
29 0.926966675122579
30 0.91310000816981
31 0.941833337148031
32 0.938499999046326
33 0.904633343219757
34 0.934133330980937
35 0.890400004386902
36 0.899900007247925
37 0.894666675726573
38 0.922333335876465
39 0.894666675726573
40 0.905933340390523
41 0.905200004577637
42 0.912933337688446
43 0.884533341725667
44 0.934900001684825
45 0.88613334496816
46 0.905200004577637
47 0.899100001653035
48 0.874000012874603
49 0.884533341725667
50 0.898300007979075
51 0.895400011539459
52 0.905933340390523
53 0.895066670576731
54 0.900033338864644
55 0.932733333110809
56 0.874000012874603
57 0.901733342806498
58 0.892200009028117
59 0.894866673151652
60 0.884533341725667
61 0.893933339913686
62 0.883400011062622
63 0.905400002002716
64 0.894966677824656
65 0.894866673151652
66 0.884533341725667
67 0.883400011062622
68 0.901666673024495
69 0.891133344173431
70 0.896600011984507
71 0.907133340835571
72 0.896600011984507
73 0.904066673914592
74 0.901400005817413
75 0.874000012874603
76 0.874000012874603
77 0.893933339913686
78 0.874000012874603
79 0.889300008614858
80 0.900900002320607
81 0.874000012874603
82 0.893933339913686
83 0.874000012874603
84 0.893933339913686
85 0.917133343219757
86 0.896600011984507
87 0.915300007661184
88 0.897933340072632
89 0.895400011539459
90 0.896600011984507
91 0.896600011984507
92 0.885900004704793
93 0.895400011539459
94 0.911866672833761
95 0.884633338451385
96 0.874000012874603
97 0.900900002320607
98 0.920866672197978
99 0.896933341026306
100 0.878566674391429
};
%\addlegendentry{DQN, n train envs=30}
\addplot [semithick, color2]
table {%
1 0.939066666666667
100 0.939066666666667
};
%\addlegendentry{Random}
\addplot [semithick, color3]
table {%
1 0.9531
100 0.9531
};
%\addlegendentry{ETS}
\addplot [semithick, color4]
table {%
1 0.9176
100 0.9176
};
%\addlegendentry{Heur-GD}
\addplot [semithick, color5, dash pattern=on 1pt off 3pt on 3pt off 3pt]
table {%
1 0.9514
100 0.9514
};
%\addlegendentry{Heur-LD}
\addplot [semithick, color6, dashed]
table {%
1 0.9678
100 0.9678
};
%\addlegendentry{Heur-AT}
