# Supplementary material for: Learn the Time to Learn: Replay Scheduling in Continual Learning
Source: arXiv:2209.08660 source file (2023-11-20)
Supplement: Supplementary file 37 [file rewards_env9.tex]

\nextgroupplot[title=Seed 8,
height=\figheight,
legend cell align={left},
legend style={
  fill opacity=0.8,
  draw opacity=1,
  text opacity=1,
  at={(0.03,0.03)},
  anchor=south west,
  draw=white!80!black
},
minor xtick={25, 75},
minor ytick={},
tick align=outside,
tick pos=left,
width=\figwidth,
x grid style={white!69.0196078431373!black},
xlabel={Eval. Steps},
xminorgrids,
xmajorgrids,
xmin=-3.95, xmax=104.95,
xtick style={color=black},
xtick={-25,0,50,100,125},
xticklabels={-25,0,50,100,125},
y grid style={white!69.0196078431373!black},
ylabel={ACC (\%)},
ymajorgrids,
ymin=0.848394991755486, ymax=0.96,
ytick style={color=black},
ytick={0.84,0.86,0.88,0.9,0.92,0.94,0.96},
yticklabels={84,86,88,90,92,94,96}
]
\addplot [semithick, color0]
table {%
1 0.928900015354157
2 0.936133348941803
3 0.927733337879181
4 0.917700004577637
5 0.940233333905538
6 0.935833334922791
7 0.939233330885569
8 0.938633334636688
9 0.924000000953674
10 0.915666667620341
11 0.912533334891001
12 0.92610000371933
13 0.937566669782003
14 0.92610000371933
15 0.92610000371933
16 0.932366669178009
17 0.932366669178009
18 0.949033335844676
19 0.932366669178009
20 0.932366669178009
21 0.92610000371933
22 0.937566669782003
23 0.937566669782003
24 0.92610000371933
25 0.92610000371933
26 0.92610000371933
27 0.92610000371933
28 0.92610000371933
29 0.92610000371933
30 0.937566669782003
31 0.937566669782003
32 0.937566669782003
33 0.92610000371933
34 0.92610000371933
35 0.92610000371933
36 0.92610000371933
37 0.92610000371933
38 0.92610000371933
39 0.92610000371933
40 0.92610000371933
41 0.937566669782003
42 0.92610000371933
43 0.929300002257029
44 0.92610000371933
45 0.92610000371933
46 0.92610000371933
47 0.92610000371933
48 0.92610000371933
49 0.92610000371933
50 0.92610000371933
51 0.92610000371933
52 0.929300002257029
53 0.92610000371933
54 0.92610000371933
55 0.929300002257029
56 0.92610000371933
57 0.932500000794729
58 0.935699999332428
59 0.92610000371933
60 0.92610000371933
61 0.932500000794729
62 0.92610000371933
63 0.935699999332428
64 0.932500000794729
65 0.932500000794729
66 0.929300002257029
67 0.932500000794729
68 0.929300002257029
69 0.932500000794729
70 0.929300002257029
71 0.92610000371933
72 0.935699999332428
73 0.932500000794729
74 0.935699999332428
75 0.932500000794729
76 0.935699999332428
77 0.935699999332428
78 0.935699999332428
79 0.932500000794729
80 0.932500000794729
81 0.935699999332428
82 0.935699999332428
83 0.932500000794729
84 0.929300002257029
85 0.935699999332428
86 0.932500000794729
87 0.932500000794729
88 0.935699999332428
89 0.929300002257029
90 0.935699999332428
91 0.935699999332428
92 0.932500000794729
93 0.935699999332428
94 0.935699999332428
95 0.935699999332428
96 0.932500000794729
97 0.935699999332428
98 0.935699999332428
99 0.932500000794729
100 0.935699999332428
};
%\addlegendentry{a2c, gae, envs=10, lr=0.0003, act=tanh}
\addplot [semithick, color1]
table {%
1 0.904766670862834
2 0.937633331616719
3 0.905566664536794
4 0.900733343760172
5 0.915266664822896
6 0.906866673628489
7 0.920000004768372
8 0.91409999926885
9 0.934233339627584
10 0.931500005722046
11 0.929066669940949
12 0.880799992879232
13 0.907833325862884
14 0.913499995072683
15 0.915166668097178
16 0.948399992783864
17 0.927533328533173
18 0.945366668701172
19 0.889599998792013
20 0.915499997138977
21 0.899666666984558
22 0.937433338165283
23 0.921833324432373
24 0.937200001875559
25 0.937966664632161
26 0.940933342774709
27 0.925766666730245
28 0.915299999713898
29 0.934566668669383
30 0.927966666221619
31 0.94226667881012
32 0.925433345635732
33 0.920000012715658
34 0.918133342266083
35 0.928066678841909
36 0.928066670894623
37 0.943433340390523
38 0.924766671657562
39 0.94496666987737
40 0.92666666507721
41 0.900266671180725
42 0.915033336480458
43 0.940733333428701
44 0.885733326276143
45 0.907466665903727
46 0.909066665172577
47 0.933133335908254
48 0.907166663805644
49 0.942533338069916
50 0.921166666348775
51 0.904433325926463
52 0.921699996789296
53 0.927033336957296
54 0.919733333587647
55 0.914300004641215
56 0.882666671276093
57 0.882300003369649
58 0.886933330694834
59 0.926900001366933
60 0.893400001525879
61 0.876566668351491
62 0.911133333047231
63 0.853233325481415
64 0.895500008265178
65 0.921533338228862
66 0.929600004355113
67 0.929933337370555
68 0.902599998315175
69 0.86850000222524
70 0.903833333651225
71 0.87593332529068
72 0.900233332316081
73 0.903633332252502
74 0.889500006039937
75 0.908799997965495
76 0.862466661135356
77 0.903633332252502
78 0.891966660817464
79 0.884499990940094
80 0.878133328755697
81 0.885066664218903
82 0.89626665910085
83 0.916033331553141
84 0.888733327388763
85 0.915866661071777
86 0.898233330249786
87 0.886366673310598
88 0.903733328978221
89 0.907166663805644
90 0.903733328978221
91 0.894866665204366
92 0.885699999332428
93 0.916766663392385
94 0.944366669654846
95 0.892499991257985
96 0.916033331553141
97 0.894866665204366
98 0.908666662375132
99 0.924999996026357
100 0.925766666730245
};
%\addlegendentry{DQN, n train envs=30}
\addplot [semithick, color2]
table {%
1 0.9076
100 0.9076
};
%\addlegendentry{Random}
\addplot [semithick, color3]
table {%
1 0.948
100 0.948
};
%\addlegendentry{ETS}
\addplot [semithick, color4]
table {%
1 0.95
100 0.95
};
%\addlegendentry{Heur-GD}
\addplot [semithick, color5, dash pattern=on 1pt off 3pt on 3pt off 3pt]
table {%
1 0.8786
100 0.8786
};
%\addlegendentry{Heur-LD}
\addplot [semithick, color6, dashed]
table {%
1 0.9393
100 0.9393
};
%\addlegendentry{Heur-AT}
