# Supplementary material for: Learn the Time to Learn: Replay Scheduling in Continual Learning
Source: arXiv:2209.08660 source file (2023-11-20)
Supplement: Supplementary file 39 [file rewards_env1.tex]

\nextgroupplot[title=Seed 10,
height=\figheight,
legend cell align={left},
legend columns=-1,
legend style={
  fill opacity=0.8,
  draw opacity=1,
  text opacity=1,
  at={(0.10,1.29)},
  anchor=south west,
  draw=white!80!black
},
minor xtick={25, 75},
minor ytick={},
tick align=outside,
tick pos=left,
width=\figwidth,
x grid style={white!69.0196078431373!black},
xlabel={Eval. Steps},
xminorgrids,
xmajorgrids,
xmin=-3.95, xmax=104.95,
xtick style={color=black},
xtick={-25,0,50,100,125},
xticklabels={-25,0,50,100,125},
y grid style={white!69.0196078431373!black},
ylabel={ACC (\%)},
ymajorgrids,
ymin=0.895982454991159, ymax=0.960314079751296,
ytick style={color=black},
ytick={0.89,0.9,0.91,0.92,0.93,0.94,0.95,0.96,0.97},
yticklabels={89,90,91,92,93,94,95,96,97}
]
\addplot [semithick, color0]
table {%
1 0.928916958967845
2 0.951259243488312
3 0.951259243488312
4 0.957143481572469
5 0.957389914989471
6 0.950179465611776
7 0.935758566856384
8 0.935758566856384
9 0.935758566856384
10 0.947296047210693
11 0.953064787387848
12 0.953064787387848
13 0.953064787387848
14 0.953064787387848
15 0.953064787387848
16 0.953064787387848
17 0.953064787387848
18 0.953064787387848
19 0.953064787387848
20 0.953064787387848
21 0.953064787387848
22 0.953064787387848
23 0.953064787387848
24 0.953064787387848
25 0.953064787387848
26 0.953064787387848
27 0.953064787387848
28 0.953064787387848
29 0.953064787387848
30 0.953064787387848
31 0.953064787387848
32 0.953064787387848
33 0.953064787387848
34 0.953064787387848
35 0.953064787387848
36 0.953064787387848
37 0.953064787387848
38 0.953064787387848
39 0.953064787387848
40 0.953064787387848
41 0.953064787387848
42 0.953064787387848
43 0.953064787387848
44 0.953064787387848
45 0.953064787387848
46 0.953064787387848
47 0.947296047210693
48 0.947296047210693
49 0.953064787387848
50 0.953064787387848
51 0.953064787387848
52 0.953064787387848
53 0.953064787387848
54 0.953064787387848
55 0.953064787387848
56 0.953064787387848
57 0.953064787387848
58 0.953064787387848
59 0.953064787387848
60 0.947296047210693
61 0.953064787387848
62 0.953064787387848
63 0.953064787387848
64 0.953064787387848
65 0.953064787387848
66 0.947296047210693
67 0.953064787387848
68 0.947296047210693
69 0.953064787387848
70 0.953064787387848
71 0.953064787387848
72 0.941527307033539
73 0.953064787387848
74 0.947296047210693
75 0.953064787387848
76 0.953064787387848
77 0.953064787387848
78 0.947296047210693
79 0.953064787387848
80 0.953064787387848
81 0.953064787387848
82 0.953064787387848
83 0.953064787387848
84 0.953064787387848
85 0.953064787387848
86 0.953064787387848
87 0.953064787387848
88 0.947296047210693
89 0.947296047210693
90 0.947296047210693
91 0.953064787387848
92 0.953064787387848
93 0.953064787387848
94 0.953064787387848
95 0.953064787387848
96 0.953064787387848
97 0.947296047210693
98 0.953064787387848
99 0.947296047210693
100 0.953064787387848
};
\addlegendentry{A2C}
\addplot [semithick, color1]
table {%
1 0.946875449021657
2 0.943612333138784
3 0.939076503117879
4 0.943958342075348
5 0.951629606882731
6 0.949499154090881
7 0.938134737809499
8 0.947858540217082
9 0.93805935382843
10 0.947194731235504
11 0.938645708560944
12 0.944262035687764
13 0.930862271785736
14 0.941974437236786
15 0.938590168952942
16 0.943620713551839
17 0.937054864565531
18 0.93942437171936
19 0.940189401308695
20 0.938030183315277
21 0.936716564496358
22 0.932151925563812
23 0.934587570031484
24 0.936899375915527
25 0.936111251513163
26 0.945568529764811
27 0.931886915365855
28 0.944513730208079
29 0.937833281358083
30 0.941893573602041
31 0.939429183801015
32 0.927043116092682
33 0.933157527446747
34 0.935961580276489
35 0.934696674346924
36 0.945227158069611
37 0.946772507826487
38 0.936443185806274
39 0.944100288550059
40 0.939507095019023
41 0.939349623521169
42 0.935918192068736
43 0.943360650539398
44 0.940596298376719
45 0.942300256093343
46 0.941220355033874
47 0.943428015708923
48 0.945602977275848
49 0.949816147486369
50 0.940117915471395
51 0.947238286336263
52 0.934195733070374
53 0.935175971190135
54 0.944136706988017
55 0.939367651939392
56 0.948354355494181
57 0.948414611816406
58 0.94425938129425
59 0.938315244515737
60 0.943881408373515
61 0.938720309734345
62 0.940491338570913
63 0.937058353424072
64 0.946232680479685
65 0.950825242201487
66 0.947540696461995
67 0.946412448088328
68 0.938605499267578
69 0.950295746326447
70 0.944109499454498
71 0.947393588225047
72 0.952604659398397
73 0.949641068776449
74 0.94713325103124
75 0.95142068862915
76 0.94816845258077
77 0.943809986114502
78 0.941947905222575
79 0.945736765861511
80 0.943446473280589
81 0.94816845258077
82 0.951026980082194
83 0.948867444197337
84 0.947391430536906
85 0.940476810932159
86 0.949786361058553
87 0.947496966520945
88 0.945095586776733
89 0.936391858259837
90 0.944066290060679
91 0.945736765861511
92 0.942870044708252
93 0.945836798350016
94 0.943091146151225
95 0.938331906000773
96 0.943332389990489
97 0.928321810563405
98 0.945367765426636
99 0.9357603708903
100 0.947986404101054
};
\addlegendentry{DQN}
\addplot [semithick, color2]
table {%
1 0.943769861300433
100 0.943769861300433
};
\addlegendentry{Random}
\addplot [semithick, color3]
table {%
1 0.898906619752983
100 0.898906619752983
};
\addlegendentry{ETS}
\addplot [semithick, color4]
table {%
1 0.946386095853952
100 0.946386095853952
};
\addlegendentry{Heur-GD}
\addplot [semithick, color5, dash pattern=on 1pt off 3pt on 3pt off 3pt]
table {%
1 0.956332387217083
100 0.956332387217083
};
\addlegendentry{Heur-LD}
\addplot [semithick, color6, dashed]
table {%
1 0.946386095853952
100 0.946386095853952
};
\addlegendentry{Heur-AT}
