# Supplementary material for: Learn the Time to Learn: Replay Scheduling in Continual Learning
Source: arXiv:2209.08660 source file (2023-11-20)
Supplement: Supplementary file 40 [file rewards_env10.tex]

\nextgroupplot[title=Seed 19,
height=\figheight,
legend cell align={left},
legend style={
  fill opacity=0.8,
  draw opacity=1,
  text opacity=1,
  at={(0.5,0.91)},
  anchor=north,
  draw=white!80!black
},
minor xtick={25, 75},
minor ytick={},
tick align=outside,
tick pos=left,
width=\figwidth,
x grid style={white!69.0196078431373!black},
xlabel={Eval. Steps},
xminorgrids,
xmajorgrids,
xmin=-3.95, xmax=104.95,
xtick style={color=black},
xtick={-25,0,50,100,125},
xticklabels={-25,0,50,100,125},
y grid style={white!69.0196078431373!black},
ymajorgrids,
ymin=0.851598749903499, ymax=0.981,%0.979828229247698,
ytick style={color=black},
ytick={0.82,0.84,0.86,0.88,0.9,0.92,0.94,0.96,0.98},
yticklabels={82,84,86,88,90,92,94,96,98}
]
\addplot [semithick, color0]
table {%
1 0.889587275187174
2 0.919530880451202
3 0.919530880451202
4 0.905146797498067
5 0.89366180896759
6 0.882801576455434
7 0.861081111431122
8 0.861081111431122
9 0.861081111431122
10 0.869421029090881
11 0.877760946750641
12 0.877760946750641
13 0.8861008644104
14 0.8861008644104
15 0.8861008644104
16 0.8861008644104
17 0.877760946750641
18 0.869421029090881
19 0.877760946750641
20 0.8861008644104
21 0.869421029090881
22 0.869421029090881
23 0.877760946750641
24 0.877760946750641
25 0.8861008644104
26 0.877760946750641
27 0.877760946750641
28 0.877760946750641
29 0.869421029090881
30 0.861081111431122
31 0.8861008644104
32 0.869421029090881
33 0.869421029090881
34 0.869421029090881
35 0.869421029090881
36 0.869421029090881
37 0.861081111431122
38 0.861081111431122
39 0.861081111431122
40 0.861081111431122
41 0.861081111431122
42 0.861081111431122
43 0.861081111431122
44 0.861081111431122
45 0.861081111431122
46 0.861081111431122
47 0.861081111431122
48 0.861081111431122
49 0.861081111431122
50 0.861081111431122
51 0.861081111431122
52 0.861081111431122
53 0.861081111431122
54 0.861081111431122
55 0.861081111431122
56 0.861081111431122
57 0.861081111431122
58 0.861081111431122
59 0.861081111431122
60 0.861081111431122
61 0.861081111431122
62 0.861081111431122
63 0.861081111431122
64 0.861081111431122
65 0.861081111431122
66 0.861081111431122
67 0.861081111431122
68 0.861081111431122
69 0.861081111431122
70 0.861081111431122
71 0.861081111431122
72 0.861081111431122
73 0.861081111431122
74 0.861081111431122
75 0.861081111431122
76 0.861081111431122
77 0.861081111431122
78 0.861081111431122
79 0.861081111431122
80 0.861081111431122
81 0.861081111431122
82 0.861081111431122
83 0.873857895533244
84 0.861081111431122
85 0.861081111431122
86 0.861081111431122
87 0.861081111431122
88 0.861081111431122
89 0.861081111431122
90 0.861081111431122
91 0.861081111431122
92 0.861081111431122
93 0.861081111431122
94 0.861081111431122
95 0.861081111431122
96 0.861081111431122
97 0.873857895533244
98 0.873857895533244
99 0.873857895533244
100 0.873857895533244
};
%\addlegendentry{a2c, gae, envs=10, lr=0.0001, act=tanh}
\addplot [semithick, color1]
table {%
1 0.885726269086202
2 0.877382560571035
3 0.884418928623199
4 0.892041838169098
5 0.89137796163559
6 0.902422265211741
7 0.88383751710256
8 0.865990130106608
9 0.905353697141012
10 0.887937192122142
11 0.887296136220296
12 0.902266867955526
13 0.894675703843435
14 0.870205307006836
15 0.895979630947113
16 0.882224980990092
17 0.894167077541351
18 0.877688086032868
19 0.87767284711202
20 0.903855450948079
21 0.888350558280945
22 0.895839536190033
23 0.870886663595835
24 0.860171274344126
25 0.871138020356496
26 0.892439810434977
27 0.886742238203685
28 0.876995591322581
29 0.87334934870402
30 0.886608910560608
31 0.894884856541951
32 0.884392738342285
33 0.891410716374715
34 0.866475296020508
35 0.886420615514119
36 0.882389406363169
37 0.884482185045878
38 0.876778841018677
39 0.893021269639333
40 0.909104073047638
41 0.86597029765447
42 0.893543310960134
43 0.874693254629771
44 0.872570939858754
45 0.889108800888062
46 0.895020401477814
47 0.893546267350515
48 0.910843590895335
49 0.899906941254934
50 0.905060505867004
51 0.894493532180786
52 0.8802689909935
53 0.898676915963491
54 0.896909979979197
55 0.893667952219645
56 0.882753384113312
57 0.906167376041413
58 0.896711560090383
59 0.88842161099116
60 0.896711560090383
61 0.883209836483002
62 0.884720551967621
63 0.892328810691834
64 0.889599196116129
65 0.899138911565145
66 0.889835818608602
67 0.890894242127736
68 0.892000540097555
69 0.883720115820567
70 0.857427362600962
71 0.874030105272929
72 0.922141476472219
73 0.89893517891566
74 0.888890000184377
75 0.868843913078308
76 0.860843499501546
77 0.895374619960785
78 0.884557974338532
79 0.892795745531718
80 0.881325622399648
81 0.8981716076533
82 0.889866157372793
83 0.8955597559611
84 0.897647456328074
85 0.885942776997884
86 0.879752838611603
87 0.891802755991618
88 0.88284113407135
89 0.889164193471273
90 0.896600727240245
91 0.881477566560109
92 0.896385391553243
93 0.903439243634542
94 0.891802755991618
95 0.897349166870117
96 0.889706297715505
97 0.891802755991618
98 0.897779067357381
99 0.877799272537231
100 0.891543749968211
};
%\addlegendentry{DQN, n train envs=30, lr=0.0001}
\addplot [semithick, color2]
table {%
1 0.949259726637197
100 0.949259726637197
};
%\addlegendentry{Random}
\addplot [semithick, color3]
table {%
1 0.973999616550235
100 0.973999616550235
};
%\addlegendentry{ETS}
\addplot [semithick, color4]
table {%
1 0.883410454122764
100 0.883410454122764
};
%\addlegendentry{Heur-GD}
\addplot [semithick, color5, dash pattern=on 1pt off 3pt on 3pt off 3pt]
table {%
1 0.883410454122764
100 0.883410454122764
};
%\addlegendentry{Heur-LD}
\addplot [semithick, color6, dashed]
table {%
1 0.883410454122764
100 0.883410454122764
};
%\addlegendentry{Heur-AT}
