# Supplementary material for: Learn the Time to Learn: Replay Scheduling in Continual Learning
Source: arXiv:2209.08660 source file (2023-11-20)
Supplement: Supplementary file 41 [file rewards_env2.tex]

\nextgroupplot[title=Seed 11,
height=\figheight,
legend cell align={left},
legend style={
  fill opacity=0.8,
  draw opacity=1,
  text opacity=1,
  at={(0.03,0.03)},
  anchor=south west,
  draw=white!80!black
},
minor xtick={25, 75},
minor ytick={},
tick align=outside,
tick pos=left,
width=\figwidth,
x grid style={white!69.0196078431373!black},
xlabel={Eval. Steps},
xminorgrids,
xmajorgrids,
xmin=-3.95, xmax=104.95,
xtick style={color=black},
xtick={-25,0,50,100,125},
xticklabels={-25,0,50,100,125},
y grid style={white!69.0196078431373!black},
ymajorgrids,
ymin=0.908595944220984, ymax=0.972076868974256,
ytick style={color=black},
ytick={0.9,0.91,0.92,0.93,0.94,0.95,0.96,0.97,0.98},
yticklabels={90,91,92,93,94,95,96,97,98}
]
\addplot [semithick, color0]
table {%
1 0.93025412162145
2 0.966550159454346
3 0.966550159454346
4 0.966692364215851
5 0.969191372394562
6 0.962275453408559
7 0.948443615436554
8 0.948443615436554
9 0.948443615436554
10 0.948443615436554
11 0.959486003716787
12 0.959486003716787
13 0.965007197856903
14 0.965007197856903
15 0.959486003716787
16 0.965007197856903
17 0.959486003716787
18 0.95396480957667
19 0.959486003716787
20 0.965007197856903
21 0.95396480957667
22 0.95396480957667
23 0.95396480957667
24 0.959486003716787
25 0.965007197856903
26 0.959486003716787
27 0.959486003716787
28 0.959486003716787
29 0.959486003716787
30 0.948443615436554
31 0.965007197856903
32 0.959486003716787
33 0.959486003716787
34 0.95396480957667
35 0.959486003716787
36 0.959486003716787
37 0.95396480957667
38 0.948443615436554
39 0.948443615436554
40 0.95396480957667
41 0.948443615436554
42 0.95396480957667
43 0.948443615436554
44 0.95396480957667
45 0.948443615436554
46 0.948443615436554
47 0.948443615436554
48 0.948443615436554
49 0.959486003716787
50 0.95396480957667
51 0.95396480957667
52 0.95396480957667
53 0.948443615436554
54 0.95396480957667
55 0.95396480957667
56 0.95396480957667
57 0.959486003716787
58 0.959486003716787
59 0.959486003716787
60 0.95396480957667
61 0.959486003716787
62 0.959486003716787
63 0.95396480957667
64 0.959486003716787
65 0.95396480957667
66 0.959486003716787
67 0.959486003716787
68 0.948443615436554
69 0.95396480957667
70 0.959486003716787
71 0.959486003716787
72 0.95396480957667
73 0.959486003716787
74 0.959486003716787
75 0.957957514127096
76 0.959486003716787
77 0.959486003716787
78 0.95396480957667
79 0.959486003716787
80 0.959486003716787
81 0.959486003716787
82 0.959486003716787
83 0.965007197856903
84 0.965007197856903
85 0.965007197856903
86 0.959486003716787
87 0.963478708267212
88 0.963478708267212
89 0.963478708267212
90 0.965007197856903
91 0.959486003716787
92 0.965007197856903
93 0.963478708267212
94 0.965007197856903
95 0.961950218677521
96 0.963478708267212
97 0.963478708267212
98 0.965007197856903
99 0.957957514127096
100 0.965007197856903
};
%\addlegendentry{a2c, gae, envs=10, lr=0.0001, act=tanh}
\addplot [semithick, color1]
table {%
1 0.96431310971578
2 0.947577182451884
3 0.963807964324951
4 0.955493418375651
5 0.948687259356181
6 0.950334775447845
7 0.939556757609049
8 0.954793548583984
9 0.946726353963216
10 0.951599208513896
11 0.938393529256185
12 0.950230268637339
13 0.94481037457784
14 0.949019559224447
15 0.935358583927155
16 0.951525259017944
17 0.940329086780548
18 0.940207115809123
19 0.922030778725942
20 0.948713715871175
21 0.957756658395131
22 0.960303183396657
23 0.938515782356262
24 0.948169044653575
25 0.955965439478556
26 0.95956890185674
27 0.96104736328125
28 0.952626403172811
29 0.962253185113271
30 0.956047920385997
31 0.964518328507741
32 0.931204243501027
33 0.929132302602132
34 0.948770991961161
35 0.963231945037842
36 0.941038012504578
37 0.952184021472931
38 0.942987537384033
39 0.952572186787923
40 0.957016579310099
41 0.949736539522807
42 0.946119463443756
43 0.951970009009043
44 0.955394093195597
45 0.959692927201589
46 0.949527859687805
47 0.948845533529917
48 0.942819035053253
49 0.939798788229624
50 0.952979226907094
51 0.950085671742757
52 0.942322667439779
53 0.954101105531057
54 0.947761142253876
55 0.942485264937083
56 0.929199473063151
57 0.944249415397644
58 0.93682914574941
59 0.946581542491913
60 0.932097168763479
61 0.93991638024648
62 0.943958739439646
63 0.923537639776866
64 0.945287108421326
65 0.954377587636312
66 0.936274802684784
67 0.936135284105937
68 0.93285071849823
69 0.929466696580251
70 0.936135284105937
71 0.929581614335378
72 0.934962407747904
73 0.936412342389425
74 0.933721160888672
75 0.930947049458822
76 0.924756940205892
77 0.91840633948644
78 0.931870416800181
79 0.927693076928457
80 0.93285071849823
81 0.932711199919383
82 0.929779700438181
83 0.916820474465688
84 0.93285071849823
85 0.931086568037669
86 0.925060860315959
87 0.936135284105937
88 0.935468244552612
89 0.936063508192698
90 0.93014775911967
91 0.941006112098694
92 0.934696197509766
93 0.945628194014231
94 0.914729758103689
95 0.943353490034739
96 0.925372048219045
97 0.926104430357615
98 0.921393620967865
99 0.924325120449066
100 0.945107527573903
};
%\addlegendentry{DQN, n train envs=30, lr=0.0001}
\addplot [semithick, color2]
table {%
1 0.911481440800678
100 0.911481440800678
};
%\addlegendentry{Random}
\addplot [semithick, color3]
table {%
1 0.937675110453656
100 0.937675110453656
};
%\addlegendentry{ETS}
\addplot [semithick, color4]
table {%
1 0.913359966355126
100 0.913359966355126
};
%\addlegendentry{Heur-GD}
\addplot [semithick, color5, dash pattern=on 1pt off 3pt on 3pt off 3pt]
table {%
1 0.913359966355126
100 0.913359966355126
};
%\addlegendentry{Heur-LD}
\addplot [semithick, color6, dashed]
table {%
1 0.913359966355126
100 0.913359966355126
};
%\addlegendentry{Heur-AT}
