# Supplementary material for: Learn the Time to Learn: Replay Scheduling in Continual Learning
Source: arXiv:2209.08660 source file (2023-11-20)
Supplement: Supplementary file 42 [file rewards_env3.tex]

\nextgroupplot[title=Seed 12,
height=\figheight,
legend cell align={left},
legend style={
  fill opacity=0.8,
  draw opacity=1,
  text opacity=1,
  at={(0.97,0.03)},
  anchor=south east,
  draw=white!80!black
},
minor xtick={25, 75},
minor ytick={},
tick align=outside,
tick pos=left,
width=\figwidth,
x grid style={white!69.0196078431373!black},
xlabel={Eval. Steps},
xminorgrids,
xmajorgrids,
xmin=-3.95, xmax=104.95,
xtick style={color=black},
xtick={-25,0,50,100,125},
xticklabels={-25,0,50,100,125},
y grid style={white!69.0196078431373!black},
ymajorgrids,
ymin=0.91, ymax=0.95,
ytick style={color=black},
ytick={0.91,0.92,0.93,0.94,0.95},
yticklabels={91,92,93,94,95}
]
\addplot [semithick, color0]
table {%
1 0.936047828197479
2 0.93209730386734
3 0.93209730386734
4 0.93806779384613
5 0.942491888999939
6 0.94399356842041
7 0.946996927261353
8 0.946996927261353
9 0.946996927261353
10 0.939809068044027
11 0.936215138435364
12 0.936215138435364
13 0.936215138435364
14 0.936215138435364
15 0.936215138435364
16 0.936215138435364
17 0.936215138435364
18 0.936215138435364
19 0.936215138435364
20 0.936215138435364
21 0.936215138435364
22 0.936215138435364
23 0.936215138435364
24 0.936215138435364
25 0.936215138435364
26 0.936215138435364
27 0.936215138435364
28 0.936215138435364
29 0.936215138435364
30 0.936215138435364
31 0.936215138435364
32 0.936215138435364
33 0.936215138435364
34 0.936215138435364
35 0.936215138435364
36 0.936215138435364
37 0.936215138435364
38 0.936215138435364
39 0.936215138435364
40 0.936215138435364
41 0.936215138435364
42 0.936215138435364
43 0.936215138435364
44 0.936215138435364
45 0.936215138435364
46 0.936215138435364
47 0.936215138435364
48 0.936215138435364
49 0.936215138435364
50 0.936215138435364
51 0.936215138435364
52 0.936215138435364
53 0.936215138435364
54 0.936215138435364
55 0.936215138435364
56 0.936215138435364
57 0.936215138435364
58 0.936215138435364
59 0.936215138435364
60 0.936215138435364
61 0.936215138435364
62 0.936215138435364
63 0.936215138435364
64 0.936215138435364
65 0.936215138435364
66 0.936215138435364
67 0.936215138435364
68 0.936215138435364
69 0.936215138435364
70 0.936215138435364
71 0.936215138435364
72 0.936215138435364
73 0.936215138435364
74 0.936215138435364
75 0.936215138435364
76 0.936215138435364
77 0.936215138435364
78 0.936215138435364
79 0.936215138435364
80 0.936215138435364
81 0.936215138435364
82 0.936215138435364
83 0.936215138435364
84 0.936215138435364
85 0.936215138435364
86 0.936215138435364
87 0.936215138435364
88 0.936215138435364
89 0.936215138435364
90 0.936215138435364
91 0.936215138435364
92 0.936215138435364
93 0.936215138435364
94 0.936215138435364
95 0.936215138435364
96 0.936215138435364
97 0.936215138435364
98 0.936215138435364
99 0.936215138435364
100 0.936215138435364
};
%\addlegendentry{a2c, gae, envs=10, lr=0.0001, act=tanh}
\addplot [semithick, color1]
table {%
1 0.920871178309123
2 0.93013197183609
3 0.930246222019195
4 0.928390061855316
5 0.929438690344493
6 0.91416691939036
7 0.932036379973094
8 0.928942743937175
9 0.92954793771108
10 0.923440019289652
11 0.913473677635193
12 0.925967379411062
13 0.93908087015152
14 0.939187920093536
15 0.913824502627055
16 0.929045836130778
17 0.931464616457621
18 0.923940670490265
19 0.927227290471395
20 0.917160820960999
21 0.928424990177155
22 0.931177361806234
23 0.928094534079234
24 0.938453257083893
25 0.932049703598022
26 0.938203299045563
27 0.944667371114095
28 0.945513312021891
29 0.935003582636515
30 0.939077254136404
31 0.938024123509725
32 0.936308602492015
33 0.945330186684926
34 0.933321825663249
35 0.941365679105123
36 0.932294563452403
37 0.924232061704
38 0.937094108263651
39 0.938669276237488
40 0.944350608189901
41 0.937705190976461
42 0.938236482938131
43 0.94044912258784
44 0.936352789402008
45 0.941683622201284
46 0.913852365811666
47 0.936676335334778
48 0.940519738197327
49 0.934788564840953
50 0.928826606273651
51 0.926246579488118
52 0.932052326202393
53 0.937740294138591
54 0.939065873622894
55 0.937133018175761
56 0.944972364107768
57 0.931926691532135
58 0.940733019510905
59 0.937922326723735
60 0.937595236301422
61 0.936160135269165
62 0.931134720643361
63 0.928145317236582
64 0.919725787639618
65 0.938266094525655
66 0.937740294138591
67 0.94044912258784
68 0.936561489105225
69 0.921501894791921
70 0.938653739293416
71 0.937740294138591
72 0.942346831162771
73 0.932896912097931
74 0.932896912097931
75 0.936324870586395
76 0.937674160798391
77 0.939540159702301
78 0.938719872633616
79 0.936561489105225
80 0.938082257906596
81 0.935581910610199
82 0.935581910610199
83 0.937674160798391
84 0.935581910610199
85 0.938583123683929
86 0.939949536323547
87 0.93824823697408
88 0.930157132943471
89 0.929747756322225
90 0.938719872633616
91 0.934307591120402
92 0.93714470465978
93 0.936324870586395
94 0.938719872633616
95 0.943891366322835
96 0.941799116134644
97 0.943471467494965
98 0.945296986897787
99 0.945296986897787
100 0.938694218794505
};
%\addlegendentry{DQN, n train envs=30, lr=0.0001}
\addplot [semithick, color2]
table {%
1 0.91578345987902
100 0.91578345987902
};
%\addlegendentry{Random}
\addplot [semithick, color3]
table {%
1 0.916884203700455
100 0.916884203700455
};
%\addlegendentry{ETS}
\addplot [semithick, color4]
table {%
1 0.9481932676297
100 0.9481932676297
};
%\addlegendentry{Heur-GD}
\addplot [semithick, color5, dash pattern=on 1pt off 3pt on 3pt off 3pt]
table {%
1 0.919327072719136
100 0.919327072719136
};
%\addlegendentry{Heur-LD}
\addplot [semithick, color6, dashed]
table {%
1 0.9481932676297
100 0.9481932676297
};
%\addlegendentry{Heur-AT}
