# Supplementary material for: Learn the Time to Learn: Replay Scheduling in Continual Learning
Source: arXiv:2209.08660 source file (2023-11-20)
Supplement: Supplementary file 43 [file rewards_env4.tex]

\nextgroupplot[title=Seed 13,
height=\figheight,
legend cell align={left},
legend style={
  fill opacity=0.8,
  draw opacity=1,
  text opacity=1,
  at={(0.97,0.03)},
  anchor=south east,
  draw=white!80!black
},
minor xtick={25, 75},
minor ytick={},
tick align=outside,
tick pos=left,
width=\figwidth,
x grid style={white!69.0196078431373!black},
xlabel={Eval. Steps},
xminorgrids,
xmajorgrids,
xmin=-3.95, xmax=104.95,
xtick style={color=black},
xtick={-25,0,50,100,125},
xticklabels={-25,0,50,100,125},
y grid style={white!69.0196078431373!black},
ymajorgrids,
ymin=0.91, ymax=0.965336399277051,
ytick style={color=black},
ytick={0.91,0.92,0.93,0.94,0.95,0.96,0.97},
yticklabels={91,92,93,94,95,96,97}
]
\addplot [semithick, color0]
table {%
1 0.958892095088959
2 0.927731931209564
3 0.927731931209564
4 0.926020010312398
5 0.951843798160553
6 0.952404113610586
7 0.953524744510651
8 0.953524744510651
9 0.953524744510651
10 0.954908986886342
11 0.955601108074188
12 0.954908986886342
13 0.955601108074188
14 0.955601108074188
15 0.955601108074188
16 0.955601108074188
17 0.955601108074188
18 0.955601108074188
19 0.954908986886342
20 0.955601108074188
21 0.955601108074188
22 0.955601108074188
23 0.955601108074188
24 0.955601108074188
25 0.955601108074188
26 0.955601108074188
27 0.955601108074188
28 0.955601108074188
29 0.954908986886342
30 0.954908986886342
31 0.955601108074188
32 0.955601108074188
33 0.955601108074188
34 0.955601108074188
35 0.955601108074188
36 0.955601108074188
37 0.955601108074188
38 0.955601108074188
39 0.954908986886342
40 0.954908986886342
41 0.955601108074188
42 0.955601108074188
43 0.955601108074188
44 0.955601108074188
45 0.955601108074188
46 0.955601108074188
47 0.955601108074188
48 0.955601108074188
49 0.955601108074188
50 0.955601108074188
51 0.955601108074188
52 0.955601108074188
53 0.955601108074188
54 0.955601108074188
55 0.955601108074188
56 0.955601108074188
57 0.955601108074188
58 0.955601108074188
59 0.955601108074188
60 0.955601108074188
61 0.955601108074188
62 0.955601108074188
63 0.955601108074188
64 0.955601108074188
65 0.955601108074188
66 0.955601108074188
67 0.955601108074188
68 0.955601108074188
69 0.955601108074188
70 0.955601108074188
71 0.955601108074188
72 0.955601108074188
73 0.955601108074188
74 0.955601108074188
75 0.955601108074188
76 0.955601108074188
77 0.955601108074188
78 0.955601108074188
79 0.955601108074188
80 0.955601108074188
81 0.955601108074188
82 0.955601108074188
83 0.955601108074188
84 0.955601108074188
85 0.955601108074188
86 0.955601108074188
87 0.955601108074188
88 0.955601108074188
89 0.955601108074188
90 0.955601108074188
91 0.955601108074188
92 0.955601108074188
93 0.955601108074188
94 0.955601108074188
95 0.948935619990031
96 0.955601108074188
97 0.955601108074188
98 0.955601108074188
99 0.955601108074188
100 0.955601108074188
};
%\addlegendentry{a2c, gae, envs=10, lr=0.0001, act=tanh}
\addplot [semithick, color1]
table {%
1 0.933407004674276
2 0.937932419776916
3 0.954649058977763
4 0.961123502254486
5 0.95722488562266
6 0.942374416192373
7 0.950480616092682
8 0.961699668566386
9 0.943480225404103
10 0.955883808930715
11 0.956374084949493
12 0.959676849842071
13 0.948708780606588
14 0.944969435532888
15 0.913432319959005
16 0.931162516276042
17 0.943092469374339
18 0.940680503845215
19 0.942775996526082
20 0.956619517008463
21 0.942394459247589
22 0.946318423748016
23 0.944139118989309
24 0.957575619220734
25 0.938874761263529
26 0.95983213186264
27 0.953909071286519
28 0.955866559346517
29 0.926699916521708
30 0.94729376633962
31 0.954144303003947
32 0.962319982051849
33 0.960712897777557
34 0.953486160437266
35 0.960502135753632
36 0.962137055397034
37 0.952059765656789
38 0.96156572898229
39 0.943518360455831
40 0.962864776452382
41 0.962342516581217
42 0.9601815422376
43 0.962748356660207
44 0.951329282919566
45 0.951728876431783
46 0.952638248602549
47 0.949295699596405
48 0.949307278792063
49 0.951911683877309
50 0.949323916435242
51 0.949902363618215
52 0.96167825460434
53 0.961225545406342
54 0.962453595797221
55 0.95560804605484
56 0.948268922170003
57 0.95331920782725
58 0.949323916435242
59 0.948883207639058
60 0.948212786515554
61 0.939271815617879
62 0.948849050203959
63 0.952510746320089
64 0.953439458211263
65 0.95031711657842
66 0.95031711657842
67 0.95031711657842
68 0.949876407782237
69 0.943306096394857
70 0.93539426724116
71 0.943306096394857
72 0.93498842716217
73 0.935734041531881
74 0.943824823697408
75 0.948426755269368
76 0.961105362574259
77 0.946707650025686
78 0.960985124111176
79 0.959930129845937
80 0.962319982051849
81 0.961771635214488
82 0.948682828744253
83 0.95632746219635
84 0.959820218880971
85 0.936562903722127
86 0.953355753421783
87 0.950977277755737
88 0.952244818210602
89 0.96241968870163
90 0.947033035755157
91 0.95017230908076
92 0.953453322251638
93 0.959820218880971
94 0.94997851451238
95 0.950737579663595
96 0.951719212532043
97 0.948948093255361
98 0.943282183011373
99 0.958789797623952
100 0.953202569484711
};
%\addlegendentry{DQN, n train envs=30, lr=0.0001}
\addplot [semithick, color2]
table {%
1 0.925438288168189
100 0.925438288168189
};
%\addlegendentry{Random}
\addplot [semithick, color3]
table {%
1 0.949541405667153
100 0.949541405667153
};
%\addlegendentry{ETS}
\addplot [semithick, color4]
table {%
1 0.946626678641995
100 0.946626678641995
};
%\addlegendentry{Heur-GD}
\addplot [semithick, color5, dash pattern=on 1pt off 3pt on 3pt off 3pt]
table {%
1 0.931740421926683
100 0.931740421926683
};
%\addlegendentry{Heur-LD}
\addplot [semithick, color6, dashed]
table {%
1 0.946626678641995
100 0.946626678641995
};
%\addlegendentry{Heur-AT}
