# Supplementary material for: Learn the Time to Learn: Replay Scheduling in Continual Learning
Source: arXiv:2209.08660 source file (2023-11-20)
Supplement: Supplementary file 44 [file rewards_env5.tex]

\nextgroupplot[title=Seed 14,
height=\figheight,
legend cell align={left},
legend style={fill opacity=0.8, draw opacity=1, text opacity=1, draw=white!80!black},
minor xtick={25, 75},
minor ytick={},
tick align=outside,
tick pos=left,
width=\figwidth,
x grid style={white!69.0196078431373!black},
xlabel={Eval. Steps},
xminorgrids,
xmajorgrids,
xmin=-3.95, xmax=104.95,
xtick style={color=black},
xtick={-25,0,50,100,125},
xticklabels={-25,0,50,100,125},
y grid style={white!69.0196078431373!black},
ylabel={ACC (\%)},
ymajorgrids,
ymin=0.80, ymax=0.95714084326699,
ytick style={color=black},
ytick={0.8,0.82,0.84,0.86,0.88,0.9,0.92,0.94,0.96},
yticklabels={80,82,84,86,88,90,92,94,96}
]
\addplot [semithick, color0]
table {%
1 0.895180523395538
2 0.911138689517975
3 0.911138689517975
4 0.916412683327993
5 0.94194061756134
6 0.906023144721985
7 0.834188199043274
8 0.834188199043274
9 0.834188199043274
10 0.863489369551341
11 0.892790540059408
12 0.892790540059408
13 0.922091710567475
14 0.922091710567475
15 0.922091710567475
16 0.922091710567475
17 0.892790540059408
18 0.892790540059408
19 0.892790540059408
20 0.922091710567475
21 0.863489369551341
22 0.863489369551341
23 0.892790540059408
24 0.892790540059408
25 0.922091710567475
26 0.892790540059408
27 0.892790540059408
28 0.892790540059408
29 0.863489369551341
30 0.834188199043274
31 0.922091710567475
32 0.892790540059408
33 0.892790540059408
34 0.863489369551341
35 0.892790540059408
36 0.863489369551341
37 0.834188199043274
38 0.834188199043274
39 0.834188199043274
40 0.834188199043274
41 0.834188199043274
42 0.834188199043274
43 0.834188199043274
44 0.834188199043274
45 0.834188199043274
46 0.834188199043274
47 0.834188199043274
48 0.834188199043274
49 0.834188199043274
50 0.834188199043274
51 0.834188199043274
52 0.834188199043274
53 0.834188199043274
54 0.834188199043274
55 0.834188199043274
56 0.834188199043274
57 0.834188199043274
58 0.834188199043274
59 0.834188199043274
60 0.834188199043274
61 0.834188199043274
62 0.834188199043274
63 0.834188199043274
64 0.834188199043274
65 0.834188199043274
66 0.834188199043274
67 0.834188199043274
68 0.834188199043274
69 0.834188199043274
70 0.834188199043274
71 0.834188199043274
72 0.834188199043274
73 0.834188199043274
74 0.834188199043274
75 0.834188199043274
76 0.834188199043274
77 0.834188199043274
78 0.834188199043274
79 0.834188199043274
80 0.834188199043274
81 0.873697964350382
82 0.834188199043274
83 0.873697964350382
84 0.834188199043274
85 0.834188199043274
86 0.834188199043274
87 0.834188199043274
88 0.834188199043274
89 0.834188199043274
90 0.834188199043274
91 0.834188199043274
92 0.834188199043274
93 0.834188199043274
94 0.834188199043274
95 0.834188199043274
96 0.834188199043274
97 0.873697964350382
98 0.873697964350382
99 0.873697964350382
100 0.873697964350382
};
%\addlegendentry{a2c, gae, envs=10, lr=0.0001, act=tanh}
\addplot [semithick, color1]
table {%
1 0.918951265017192
2 0.914643760522207
3 0.890170832475026
4 0.888232890764872
5 0.936446531613668
6 0.931923019886017
7 0.878935094674428
8 0.845736042658488
9 0.909325619538625
10 0.880701665083567
11 0.858427302042643
12 0.926967962582906
13 0.892405494054159
14 0.876188401381175
15 0.910808066527049
16 0.941362178325653
17 0.890922005971273
18 0.847341040770213
19 0.900671565532684
20 0.899323832988739
21 0.926570749282837
22 0.884016382694244
23 0.889869260787964
24 0.88899735212326
25 0.91111958026886
26 0.88075882991155
27 0.887317089239756
28 0.885049939155579
29 0.921867724259694
30 0.893267647425334
31 0.923698063691457
32 0.8932408452034
33 0.950231230258942
34 0.912580700715383
35 0.925186983744303
36 0.924604952335358
37 0.926906414826711
38 0.940223197142283
39 0.929221510887146
40 0.898390038808187
41 0.884088778495788
42 0.881787316004435
43 0.915848509470622
44 0.927761924266815
45 0.896943831443787
46 0.867083517710368
47 0.907848850886027
48 0.933225011825562
49 0.906436268488566
50 0.917693932851156
51 0.920054097970327
52 0.881953227519989
53 0.933807043234507
54 0.90413631995519
55 0.913053957621257
56 0.914420433839162
57 0.907064394156138
58 0.920046651363373
59 0.930334810415904
60 0.907885869344076
61 0.939968597888947
62 0.874659331639608
63 0.908087277412415
64 0.9074529449145
65 0.875843743483225
66 0.906574738025665
67 0.934265609582265
68 0.906367846330007
69 0.930065075556437
70 0.920240493615468
71 0.934265609582265
72 0.928200288613637
73 0.897584708531698
74 0.912244832515717
75 0.905655531088511
76 0.907818524042765
77 0.912106362978617
78 0.909943370024363
79 0.932419820626577
80 0.907956993579864
81 0.906237562497457
82 0.896931223074595
83 0.892643384138743
84 0.910525401433309
85 0.892643384138743
86 0.892643384138743
87 0.907956993579864
88 0.91185184319814
89 0.907755585511525
90 0.893476204077403
91 0.907818524042765
92 0.909790639082591
93 0.907818524042765
94 0.892643384138743
95 0.906237562497457
96 0.892643384138743
97 0.892643384138743
98 0.892643384138743
99 0.911218718687693
100 0.892643384138743
};
%\addlegendentry{DQN, n train envs=30, lr=0.0001}
\addplot [semithick, color2]
table {%
1 0.838503634731188
100 0.838503634731188
};
%\addlegendentry{Random}
\addplot [semithick, color3]
table {%
1 0.872864057756591
100 0.872864057756591
};
%\addlegendentry{ETS}
\addplot [semithick, color4]
table {%
1 0.812038970097982
100 0.812038970097982
};
%\addlegendentry{Heur-GD}
\addplot [semithick, color5, dash pattern=on 1pt off 3pt on 3pt off 3pt]
table {%
1 0.812038970097982
100 0.812038970097982
};
%\addlegendentry{Heur-LD}
\addplot [semithick, color6, dashed]
table {%
1 0.823641171956639
100 0.823641171956639
};
%\addlegendentry{Heur-AT}
