# Supplementary material for: Learn the Time to Learn: Replay Scheduling in Continual Learning
Source: arXiv:2209.08660 source file (2023-11-20)
Supplement: Supplementary file 45 [file rewards_env6.tex]

\nextgroupplot[title=Seed 15,
height=\figheight,
legend cell align={left},
legend style={
  fill opacity=0.8,
  draw opacity=1,
  text opacity=1,
  at={(0.97,0.03)},
  anchor=south east,
  draw=white!80!black
},
minor xtick={25, 75},
minor ytick={},
tick align=outside,
tick pos=left,
width=\figwidth,
x grid style={white!69.0196078431373!black},
xlabel={Eval. Steps},
xminorgrids,
xmajorgrids,
xmin=-3.95, xmax=104.95,
xtick style={color=black},
xtick={-25,0,50,100,125},
xticklabels={-25,0,50,100,125},
y grid style={white!69.0196078431373!black},
ymajorgrids,
ymin=0.917591079316641, ymax=0.962546271995501,
ytick style={color=black},
ytick={0.89,0.90,0.91,0.92,0.93,0.94,0.95,0.96,0.97},
yticklabels={89,90,91,92,93,94,95,96,97}
]
\addplot [semithick, color0]
table {%
1 0.951650253931681
2 0.940867698192596
3 0.940867698192596
4 0.948078032334645
5 0.948131513595581
6 0.944906004269918
7 0.938454985618591
8 0.938454985618591
9 0.938454985618591
10 0.944964607556661
11 0.948219418525696
12 0.944964607556661
13 0.948219418525696
14 0.948219418525696
15 0.948219418525696
16 0.948219418525696
17 0.948219418525696
18 0.948219418525696
19 0.948219418525696
20 0.948219418525696
21 0.948219418525696
22 0.948219418525696
23 0.948219418525696
24 0.948219418525696
25 0.948219418525696
26 0.948219418525696
27 0.948219418525696
28 0.948219418525696
29 0.948219418525696
30 0.944964607556661
31 0.948219418525696
32 0.948219418525696
33 0.948219418525696
34 0.948219418525696
35 0.948219418525696
36 0.948219418525696
37 0.948219418525696
38 0.948219418525696
39 0.948219418525696
40 0.948219418525696
41 0.948219418525696
42 0.948219418525696
43 0.948219418525696
44 0.948219418525696
45 0.948219418525696
46 0.948219418525696
47 0.944964607556661
48 0.944964607556661
49 0.948219418525696
50 0.948219418525696
51 0.948219418525696
52 0.948219418525696
53 0.948219418525696
54 0.948219418525696
55 0.948219418525696
56 0.948219418525696
57 0.948219418525696
58 0.948219418525696
59 0.948219418525696
60 0.944964607556661
61 0.948219418525696
62 0.948219418525696
63 0.948219418525696
64 0.948219418525696
65 0.948219418525696
66 0.948219418525696
67 0.948219418525696
68 0.948219418525696
69 0.948219418525696
70 0.948219418525696
71 0.948219418525696
72 0.944964607556661
73 0.948219418525696
74 0.948219418525696
75 0.948219418525696
76 0.948219418525696
77 0.948219418525696
78 0.948219418525696
79 0.948219418525696
80 0.948219418525696
81 0.948219418525696
82 0.948219418525696
83 0.948219418525696
84 0.948219418525696
85 0.948219418525696
86 0.948219418525696
87 0.948219418525696
88 0.948219418525696
89 0.948219418525696
90 0.948219418525696
91 0.948219418525696
92 0.948219418525696
93 0.948219418525696
94 0.948219418525696
95 0.948219418525696
96 0.948219418525696
97 0.948219418525696
98 0.948219418525696
99 0.948219418525696
100 0.948219418525696
};
%\addlegendentry{a2c, gae, envs=10, lr=0.0001, act=tanh}
\addplot [semithick, color1]
table {%
1 0.955312685171763
2 0.954510879516601
3 0.950444503625234
4 0.950363171100617
5 0.953102123737335
6 0.952889839808146
7 0.947375639279683
8 0.942846246560415
9 0.953287172317505
10 0.946167325973511
11 0.929952383041382
12 0.95445925394694
13 0.94297255674998
14 0.947870596249898
15 0.942315165201823
16 0.952336267630259
17 0.946282267570496
18 0.94942049185435
19 0.944900278250376
20 0.941963708400726
21 0.944639849662781
22 0.946689927577972
23 0.943459892272949
24 0.940949189662933
25 0.942495286464691
26 0.937013586362203
27 0.944521121184031
28 0.945434542496999
29 0.944001150131226
30 0.946851003170013
31 0.948784677187602
32 0.944281967480977
33 0.94452440738678
34 0.933093698819478
35 0.935895168781281
36 0.91963449716568
37 0.948877461751302
38 0.941479408740997
39 0.953234493732452
40 0.942806319395701
41 0.94194803237915
42 0.940852161248525
43 0.94433708190918
44 0.944278434912364
45 0.937031189600627
46 0.947922241687775
47 0.942180744806925
48 0.947116935253143
49 0.944611314932505
50 0.934834929307302
51 0.937804273764292
52 0.948080412546794
53 0.944634008407593
54 0.945612168312073
55 0.948067510128021
56 0.94510854880015
57 0.946430079142253
58 0.935739835103353
59 0.94833820660909
60 0.950487144788106
61 0.939296062787374
62 0.946170834700267
63 0.95057110786438
64 0.94088382323583
65 0.944602783521016
66 0.941458721955617
67 0.944401093324025
68 0.946956646442413
69 0.942628570397695
70 0.944659399986267
71 0.943167996406555
72 0.946911919116974
73 0.944707687695821
74 0.952685157457987
75 0.942673154671987
76 0.936400751272837
77 0.944943662484487
78 0.943593974908193
79 0.948078417778015
80 0.949201222260793
81 0.94095420440038
82 0.952070224285126
83 0.941591954231262
84 0.951161714394887
85 0.948766322930654
86 0.945157579580943
87 0.945880568027496
88 0.943079562981923
89 0.952671849727631
90 0.945184195041657
91 0.94071048895518
92 0.943040283521016
93 0.945184195041657
94 0.95034921169281
95 0.947856406370799
96 0.950465142726898
97 0.942603389422099
98 0.942355012893677
99 0.953934605916341
100 0.946316822369893
};
%\addlegendentry{DQN, n train envs=30, lr=0.0001}
\addplot [semithick, color2]
table {%
1 0.937166291149101
100 0.937166291149101
};
%\addlegendentry{Random}
\addplot [semithick, color3]
table {%
1 0.953225047502535
100 0.953225047502535
};
%\addlegendentry{ETS}
\addplot [semithick, color4]
table {%
1 0.959211434368453
100 0.959211434368453
};
%\addlegendentry{Heur-GD}
\addplot [semithick, color5, dash pattern=on 1pt off 3pt on 3pt off 3pt]
table {%
1 0.960502854146462
100 0.960502854146462
};
%\addlegendentry{Heur-LD}
\addplot [semithick, color6, dashed]
table {%
1 0.959211434368453
100 0.959211434368453
};
%\addlegendentry{Heur-AT}
