# Supplementary material for: Learn the Time to Learn: Replay Scheduling in Continual Learning
Source: arXiv:2209.08660 source file (2023-11-20)
Supplement: Supplementary file 46 [file rewards_env7.tex]

\nextgroupplot[title=Seed 16,
height=\figheight,
legend cell align={left},
legend style={
  fill opacity=0.8,
  draw opacity=1,
  text opacity=1,
  at={(0.5,0.09)},
  anchor=south,
  draw=white!80!black
},
minor xtick={25, 75},
minor ytick={},
tick align=outside,
tick pos=left,
width=\figwidth,
x grid style={white!69.0196078431373!black},
xlabel={Eval. Steps},
xminorgrids,
xmajorgrids,
xmin=-3.95, xmax=104.95,
xtick style={color=black},
xtick={-25,0,50,100,125},
xticklabels={-25,0,50,100,125},
y grid style={white!69.0196078431373!black},
ymajorgrids,
ymin=0.786342887914087, ymax=0.950188479875955,
ytick style={color=black},
ytick={0.78,0.8,0.82,0.84,0.86,0.88,0.9,0.92,0.94,0.96},
yticklabels={78,80,82,84,86,88,90,92,94,96}
]
\addplot [semithick, color0]
table {%
1 0.89561520020167
2 0.842172574996948
3 0.842172574996948
4 0.870251055558522
5 0.886999356746674
6 0.892352298895518
7 0.903058183193207
8 0.903058183193207
9 0.903058183193207
10 0.912424429257711
11 0.921790675322215
12 0.921790675322215
13 0.931156921386719
14 0.931156921386719
15 0.931156921386719
16 0.931156921386719
17 0.921790675322215
18 0.912424429257711
19 0.921790675322215
20 0.931156921386719
21 0.912424429257711
22 0.912424429257711
23 0.921790675322215
24 0.921790675322215
25 0.931156921386719
26 0.921790675322215
27 0.921790675322215
28 0.921790675322215
29 0.912424429257711
30 0.903058183193207
31 0.931156921386719
32 0.912424429257711
33 0.912424429257711
34 0.912424429257711
35 0.912424429257711
36 0.912424429257711
37 0.903058183193207
38 0.903058183193207
39 0.903058183193207
40 0.903058183193207
41 0.903058183193207
42 0.903058183193207
43 0.903058183193207
44 0.903058183193207
45 0.903058183193207
46 0.903058183193207
47 0.903058183193207
48 0.903058183193207
49 0.903058183193207
50 0.903058183193207
51 0.903058183193207
52 0.903058183193207
53 0.903058183193207
54 0.903058183193207
55 0.903058183193207
56 0.903058183193207
57 0.903058183193207
58 0.903058183193207
59 0.903058183193207
60 0.903058183193207
61 0.903058183193207
62 0.903058183193207
63 0.903058183193207
64 0.903058183193207
65 0.903058183193207
66 0.903058183193207
67 0.903058183193207
68 0.903058183193207
69 0.903058183193207
70 0.903058183193207
71 0.903058183193207
72 0.903058183193207
73 0.903058183193207
74 0.903058183193207
75 0.903058183193207
76 0.903058183193207
77 0.903058183193207
78 0.903058183193207
79 0.903058183193207
80 0.903058183193207
81 0.909743805726369
82 0.903058183193207
83 0.909743805726369
84 0.903058183193207
85 0.903058183193207
86 0.903058183193207
87 0.903058183193207
88 0.903058183193207
89 0.903058183193207
90 0.903058183193207
91 0.903058183193207
92 0.903058183193207
93 0.903058183193207
94 0.903058183193207
95 0.903058183193207
96 0.903058183193207
97 0.909743805726369
98 0.909743805726369
99 0.909743805726369
100 0.909743805726369
};
%\addlegendentry{a2c, gae, envs=10, lr=0.0001, act=tanh}
\addplot [semithick, color1]
table {%
1 0.91650405327479
2 0.904043237368266
3 0.913246476650238
4 0.870602770646413
5 0.886044383049011
6 0.922824776172638
7 0.894750980536143
8 0.892096320788066
9 0.922540358702342
10 0.905100329717
11 0.933740385373433
12 0.899058349927266
13 0.889970529079437
14 0.892187794049581
15 0.895830094814301
16 0.90184234380722
17 0.902475380897522
18 0.892988248666128
19 0.915492935975393
20 0.878717788060506
21 0.904989989598592
22 0.914053905010224
23 0.887466553846995
24 0.917130720615387
25 0.922701911131541
26 0.89799503882726
27 0.924551383654276
28 0.921796270211538
29 0.896597564220428
30 0.917688274383545
31 0.931189711888631
32 0.912550703684489
33 0.926023821036021
34 0.921841239929199
35 0.933752107620239
36 0.913284889856974
37 0.930583624045054
38 0.919631548722585
39 0.934001803398132
40 0.923692639668783
41 0.915505905946096
42 0.913579150040944
43 0.923930390675863
44 0.93449072043101
45 0.941302156448364
46 0.925169106324514
47 0.922530794143677
48 0.942740952968597
49 0.929424242178599
50 0.897265724341075
51 0.92692547639211
52 0.919515085220337
53 0.904395190874736
54 0.919797885417938
55 0.903674515088399
56 0.918722422917684
57 0.882863481839498
58 0.90570692618688
59 0.883204686641693
60 0.911331284046173
61 0.89586668809255
62 0.900129838784536
63 0.880136934916178
64 0.885089035828908
65 0.875284890333811
66 0.885857550303141
67 0.894540385405223
68 0.883335530757904
69 0.905438296000163
70 0.903595383961995
71 0.890290224552155
72 0.902651099363963
73 0.916800002257029
74 0.913987970352173
75 0.892326617240906
76 0.903872009118398
77 0.912424445152283
78 0.893903156121572
79 0.896357595920563
80 0.901084935665131
81 0.89387929836909
82 0.909589604536692
83 0.91767992178599
84 0.910073781013489
85 0.899599913756053
86 0.897598250706991
87 0.915892783800761
88 0.898820344607035
89 0.918456892172495
90 0.93744740486145
91 0.923053538799286
92 0.931306978066762
93 0.930489540100098
94 0.898673872152964
95 0.888887651761373
96 0.920562887191772
97 0.911262706915537
98 0.910187097390493
99 0.899929853280385
100 0.93744740486145
};
%\addlegendentry{DQN, n train envs=30, lr=0.0001}
\addplot [semithick, color2]
table {%
1 0.8366389860345
100 0.8366389860345
};
%\addlegendentry{Random}
\addplot [semithick, color3]
table {%
1 0.793790414821445
100 0.793790414821445
};
%\addlegendentry{ETS}
\addplot [semithick, color4]
table {%
1 0.911572701428831
100 0.911572701428831
};
%\addlegendentry{Heur-GD}
\addplot [semithick, color5, dash pattern=on 1pt off 3pt on 3pt off 3pt]
table {%
1 0.911572701428831
100 0.911572701428831
};
%\addlegendentry{Heur-LD}
\addplot [semithick, color6, dashed]
table {%
1 0.911572701428831
100 0.911572701428831
};
%\addlegendentry{Heur-AT}
