# Supplementary material for: Learn the Time to Learn: Replay Scheduling in Continual Learning
Source: arXiv:2209.08660 source file (2023-11-20)
Supplement: Supplementary file 47 [file rewards_env8.tex]

\nextgroupplot[title=Seed 17,
height=\figheight,
legend cell align={left},
legend style={
  fill opacity=0.8,
  draw opacity=1,
  text opacity=1,
  at={(0.97,0.03)},
  anchor=south east,
  draw=white!80!black
},
minor xtick={25, 75},
minor ytick={},
tick align=outside,
tick pos=left,
width=\figwidth,
x grid style={white!69.0196078431373!black},
xlabel={Eval. Steps},
xminorgrids,
xmajorgrids,
xmin=-3.95, xmax=104.95,
xtick style={color=black},
xtick={-25,0,50,100,125},
xticklabels={-25,0,50,100,125},
y grid style={white!69.0196078431373!black},
ymajorgrids,
ymin=0.904683085481326, ymax=0.96807973364989,
ytick style={color=black},
ytick={0.9,0.91,0.92,0.93,0.94,0.95,0.96,0.97},
yticklabels={90,91,92,93,94,95,96,97}
]
\addplot [semithick, color0]
table {%
1 0.910669771830241
2 0.913990163803101
3 0.913990163803101
4 0.937742825349172
5 0.964568865299225
6 0.963402545452118
7 0.961069905757904
8 0.961069905757904
9 0.961069905757904
10 0.950339114665985
11 0.939608323574066
12 0.939608323574066
13 0.928877532482147
14 0.928877532482147
15 0.928877532482147
16 0.928877532482147
17 0.939608323574066
18 0.939608323574066
19 0.939608323574066
20 0.928877532482147
21 0.950339114665985
22 0.950339114665985
23 0.939608323574066
24 0.939608323574066
25 0.928877532482147
26 0.939608323574066
27 0.939608323574066
28 0.939608323574066
29 0.950339114665985
30 0.961069905757904
31 0.928877532482147
32 0.939608323574066
33 0.939608323574066
34 0.950339114665985
35 0.939608323574066
36 0.939608323574066
37 0.961069905757904
38 0.961069905757904
39 0.961069905757904
40 0.961069905757904
41 0.961069905757904
42 0.961069905757904
43 0.961069905757904
44 0.961069905757904
45 0.961069905757904
46 0.961069905757904
47 0.961069905757904
48 0.961069905757904
49 0.961069905757904
50 0.961069905757904
51 0.961069905757904
52 0.961069905757904
53 0.961069905757904
54 0.961069905757904
55 0.961069905757904
56 0.961069905757904
57 0.961069905757904
58 0.961069905757904
59 0.961069905757904
60 0.961069905757904
61 0.961069905757904
62 0.961069905757904
63 0.961069905757904
64 0.961069905757904
65 0.961069905757904
66 0.961069905757904
67 0.961069905757904
68 0.961069905757904
69 0.961069905757904
70 0.961069905757904
71 0.961069905757904
72 0.961069905757904
73 0.961069905757904
74 0.950339114665985
75 0.950339114665985
76 0.961069905757904
77 0.961069905757904
78 0.961069905757904
79 0.961069905757904
80 0.961069905757904
81 0.962532703081767
82 0.961069905757904
83 0.962532703081767
84 0.950339114665985
85 0.961069905757904
86 0.961069905757904
87 0.961069905757904
88 0.961069905757904
89 0.961069905757904
90 0.961069905757904
91 0.961069905757904
92 0.961069905757904
93 0.961069905757904
94 0.961069905757904
95 0.961069905757904
96 0.961069905757904
97 0.962532703081767
98 0.950339114665985
99 0.96399550040563
100 0.962532703081767
};
%\addlegendentry{a2c, gae, envs=10, lr=0.0001, act=tanh}
\addplot [semithick, color1]
table {%
1 0.933694044748942
2 0.926308786869049
3 0.921757038434346
4 0.965198067824046
5 0.944572329521179
6 0.931518427530925
7 0.922107565402985
8 0.959665381908417
9 0.949670712153117
10 0.953983028729757
11 0.942034848531087
12 0.933266806602478
13 0.913771156469981
14 0.962546249230703
15 0.908211366335551
16 0.947611308097839
17 0.940364253520966
18 0.931723054250081
19 0.929577310880025
20 0.94657678604126
21 0.964511871337891
22 0.946507374445597
23 0.940001010894775
24 0.951151200135549
25 0.949984566370646
26 0.946573030948639
27 0.932349212964376
28 0.931950350602468
29 0.959392273426056
30 0.95118575890859
31 0.958781282107035
32 0.957411229610443
33 0.957411229610443
34 0.964111963907878
35 0.9510697722435
36 0.944499532381693
37 0.95381905635198
38 0.958084833621979
39 0.948182725906372
40 0.936690219243368
41 0.9348282178243
42 0.937214688460032
43 0.93867126305898
44 0.937214688460032
45 0.94951612552007
46 0.944769303003947
47 0.948514668146769
48 0.950325326124827
49 0.930569752057393
50 0.941978732744853
51 0.931885993480682
52 0.929910405476888
53 0.947342518965403
54 0.962368563810984
55 0.949444548288981
56 0.90756475130717
57 0.932972856362661
58 0.951336709658305
59 0.934249567985535
60 0.945160853862762
61 0.937905418872833
62 0.925836074352264
63 0.937074704964956
64 0.929561177889506
65 0.94193129936854
66 0.926242605845133
67 0.949566117922465
68 0.909849981466929
69 0.912361987431844
70 0.913712362448374
71 0.944270098209381
72 0.93283261458079
73 0.944833838939667
74 0.919162484010061
75 0.919967412948608
76 0.942409745852152
77 0.962638862927755
78 0.949912059307099
79 0.959818820158641
80 0.922741361459096
81 0.94126779238383
82 0.95930495262146
83 0.953799839814504
84 0.948515470822652
85 0.940180532137553
86 0.949009684721629
87 0.936057690779368
88 0.943376962343852
89 0.93882653315862
90 0.939832083384196
91 0.919162484010061
92 0.919162484010061
93 0.937798810005188
94 0.950980007648468
95 0.93679758310318
96 0.949615931510925
97 0.961728151639302
98 0.931899086634318
99 0.909086700280507
100 0.958308335145314
};
%\addlegendentry{DQN, n train envs=30, lr=0.0001}
\addplot [semithick, color2]
table {%
1 0.962258720618549
100 0.962258720618549
};
%\addlegendentry{Random}
\addplot [semithick, color3]
table {%
1 0.956852431378258
100 0.956852431378258
};
%\addlegendentry{ETS}
\addplot [semithick, color4]
table {%
1 0.93479620382951
100 0.93479620382951
};
%\addlegendentry{Heur-GD}
\addplot [semithick, color5, dash pattern=on 1pt off 3pt on 3pt off 3pt]
table {%
1 0.93479620382951
100 0.93479620382951
};
%\addlegendentry{Heur-LD}
\addplot [semithick, color6, dashed]
table {%
1 0.93479620382951
100 0.93479620382951
};
%\addlegendentry{Heur-AT}
