# Supplementary material for: Learn the Time to Learn: Replay Scheduling in Continual Learning
Source: arXiv:2209.08660 source file (2023-11-20)
Supplement: Supplementary file 48 [file rewards_env9.tex]

\nextgroupplot[title=Seed 18,
height=\figheight,
legend cell align={left},
legend style={
  fill opacity=0.8,
  draw opacity=1,
  text opacity=1,
  at={(0.97,0.03)},
  anchor=south east,
  draw=white!80!black
},
minor xtick={25, 75},
minor ytick={},
tick align=outside,
tick pos=left,
width=\figwidth,
x grid style={white!69.0196078431373!black},
xlabel={Eval. Steps},
xminorgrids,
xmajorgrids,
xmin=-3.95, xmax=104.95,
xtick style={color=black},
xtick={-25,0,50,100,125},
xticklabels={-25,0,50,100,125},
y grid style={white!69.0196078431373!black},
ylabel={ACC (\%)},
ymajorgrids,
ymin=0.830549303416718, ymax=0.938523592342451,
ytick style={color=black},
ytick={0.82,0.84,0.86,0.88,0.9,0.92,0.94},
yticklabels={82,84,86,88,90,92,94}
]
\addplot [semithick, color0]
table {%
1 0.87737991809845
2 0.913773119449615
3 0.913773119449615
4 0.886410609881083
5 0.896446752548218
6 0.892599534988403
7 0.884905099868774
8 0.884905099868774
9 0.884905099868774
10 0.884905099868774
11 0.905919059117635
12 0.905919059117635
13 0.916426038742065
14 0.916426038742065
15 0.916426038742065
16 0.916426038742065
17 0.905919059117635
18 0.895412079493205
19 0.905919059117635
20 0.916426038742065
21 0.895412079493205
22 0.895412079493205
23 0.905919059117635
24 0.905919059117635
25 0.916426038742065
26 0.905919059117635
27 0.905919059117635
28 0.905919059117635
29 0.905919059117635
30 0.884905099868774
31 0.916426038742065
32 0.905919059117635
33 0.905919059117635
34 0.895412079493205
35 0.916426038742065
36 0.905919059117635
37 0.895412079493205
38 0.884905099868774
39 0.884905099868774
40 0.895412079493205
41 0.884905099868774
42 0.905919059117635
43 0.884905099868774
44 0.895412079493205
45 0.884905099868774
46 0.884905099868774
47 0.884905099868774
48 0.884905099868774
49 0.905919059117635
50 0.895412079493205
51 0.895412079493205
52 0.905919059117635
53 0.884905099868774
54 0.895412079493205
55 0.895412079493205
56 0.895412079493205
57 0.905919059117635
58 0.905919059117635
59 0.905919059117635
60 0.895412079493205
61 0.905919059117635
62 0.895412079493205
63 0.895412079493205
64 0.905919059117635
65 0.895412079493205
66 0.905919059117635
67 0.905919059117635
68 0.884905099868774
69 0.895412079493205
70 0.895412079493205
71 0.905919059117635
72 0.895412079493205
73 0.895412079493205
74 0.895412079493205
75 0.890624399979909
76 0.905919059117635
77 0.905919059117635
78 0.884905099868774
79 0.905919059117635
80 0.905919059117635
81 0.895412079493205
82 0.895412079493205
83 0.916426038742065
84 0.916426038742065
85 0.905919059117635
86 0.905919059117635
87 0.890624399979909
88 0.890624399979909
89 0.90113137960434
90 0.916426038742065
91 0.905919059117635
92 0.916426038742065
93 0.90113137960434
94 0.916426038742065
95 0.90113137960434
96 0.90113137960434
97 0.878151484330495
98 0.905919059117635
99 0.890624399979909
100 0.916426038742065
};
%\addlegendentry{a2c, gae, envs=10, lr=0.0001, act=tanh}
\addplot [semithick, color1]
table {%
1 0.835457225640615
2 0.866590360800425
3 0.883082008361816
4 0.84378301302592
5 0.836289616425832
6 0.894843550523122
7 0.866071108977
8 0.901073793570201
9 0.871098466714223
10 0.870586188634237
11 0.905485240618388
12 0.899811192353567
13 0.886938579877218
14 0.892894279956818
15 0.895080868403117
16 0.884705098470052
17 0.889181693394979
18 0.898494637012482
19 0.882737370332082
20 0.893611327807109
21 0.897111248970032
22 0.877803178628286
23 0.891212360064189
24 0.885723785559336
25 0.882922617594401
26 0.885075986385345
27 0.891451811790466
28 0.891869429747264
29 0.896333336830139
30 0.893889530499776
31 0.890659173329671
32 0.89218213558197
33 0.893445599079132
34 0.876827534039815
35 0.89242324034373
36 0.879579774538676
37 0.889278848965963
38 0.878133809566498
39 0.885611867904663
40 0.89532059431076
41 0.891281219323476
42 0.901695509751638
43 0.892548310756683
44 0.891281219323476
45 0.891281219323476
46 0.891281219323476
47 0.898888544241587
48 0.892741445700328
49 0.891502372423808
50 0.898740887641907
51 0.905765648682912
52 0.900015036265055
53 0.895757122834524
54 0.894678008556366
55 0.893160049120585
56 0.896606580416361
57 0.902120486895243
58 0.896369874477386
59 0.898652072747548
60 0.891733455657959
61 0.895412643750509
62 0.89339675505956
63 0.883882466952006
64 0.896986917654673
65 0.87491637468338
66 0.896986917654673
67 0.883818463484446
68 0.89825400908788
69 0.896606580416361
70 0.891910247008006
71 0.893777092297872
72 0.893777092297872
73 0.896986917654673
74 0.894666830698649
75 0.894666830698649
76 0.894666830698649
77 0.895412643750509
78 0.896679735183716
79 0.897694949309031
80 0.905765648682912
81 0.896679735183716
82 0.897694949309031
83 0.893621385097504
84 0.902581822872162
85 0.893621385097504
86 0.897694949309031
87 0.897694949309031
88 0.88617521127065
89 0.893621385097504
90 0.89086480140686
91 0.897694949309031
92 0.897694949309031
93 0.894666830698649
94 0.894666830698649
95 0.895933922131856
96 0.894286493460337
97 0.894666830698649
98 0.893621385097504
99 0.899679871400197
100 0.897694949309031
};
%\addlegendentry{DQN, n train envs=30, lr=0.0001}
\addplot [semithick, color2]
table {%
1 0.933615670118554
100 0.933615670118554
};
%\addlegendentry{Random}
\addplot [semithick, color3]
table {%
1 0.928894772109996
100 0.928894772109996
};
%\addlegendentry{ETS}
\addplot [semithick, color4]
table {%
1 0.878206432691232
100 0.878206432691232
};
%\addlegendentry{Heur-GD}
\addplot [semithick, color5, dash pattern=on 1pt off 3pt on 3pt off 3pt]
table {%
1 0.878206432691232
100 0.878206432691232
};
%\addlegendentry{Heur-LD}
\addplot [semithick, color6, dashed]
table {%
1 0.878206432691232
100 0.878206432691232
};
%\addlegendentry{Heur-AT}
