# Supplementary material for: Learn the Time to Learn: Replay Scheduling in Continual Learning
Source: arXiv:2209.08660 source file (2023-11-20)
Supplement: Supplementary file 50 [file rewards_env1.tex]

\nextgroupplot[title=Seed 0,
height=\figheight,
legend cell align={left},
legend columns=-1,
legend style={
  fill opacity=0.8,
  draw opacity=1,
  text opacity=1,
  at={(0.10,1.29)},
  anchor=south west,
  draw=white!80!black
},
minor xtick={25, 75},
minor ytick={},
tick align=outside,
tick pos=left,
width=\figwidth,
x grid style={white!69.0196078431373!black},
xlabel={Eval. Steps},
xminorgrids,
xmajorgrids,
xmin=-3.95, xmax=104.95,
xtick style={color=black},
xtick={-25,0,50,100,125},
xticklabels={-25,0,50,100,125},
y grid style={white!69.0196078431373!black},
ylabel={ACC (\%)},
ymajorgrids,
ymin=0.874000021219254, ymax=0.944911737839381,
ytick style={color=black},
ytick={0.87,0.88,0.89,0.9,0.91,0.92,0.93,0.94,0.95},
yticklabels={87,88,89,90,91,92,93,94,95}
]
\addplot [semithick, color0]
table {%
1 0.920442871252696
2 0.941688477993011
3 0.941688477993011
4 0.941688477993011
5 0.92857813835144
6 0.90269779364268
7 0.899552301565806
8 0.89826672077179
9 0.901317000389099
10 0.90269779364268
11 0.899552301565806
12 0.893451742331187
13 0.899552301565806
14 0.911943844954173
15 0.90712886651357
16 0.896502021948497
17 0.897882815202077
18 0.902313888072968
19 0.90712886651357
20 0.89826672077179
21 0.892070949077606
22 0.896502021948497
23 0.897882815202077
24 0.90712886651357
25 0.900933094819387
26 0.897882815202077
27 0.911943844954173
28 0.90574807325999
29 0.89826672077179
30 0.903991615772247
31 0.897794369856517
32 0.902313888072968
33 0.90712886651357
34 0.911943844954173
35 0.911943844954173
36 0.911943844954173
37 0.902313888072968
38 0.896561602751414
39 0.902313888072968
40 0.909403892358144
41 0.909403892358144
42 0.914218870798747
43 0.916493896643321
44 0.910741611321767
45 0.914218870798747
46 0.909403892358144
47 0.923292430241903
48 0.923583900928497
49 0.916493896643321
50 0.923583900928497
51 0.925210293134053
52 0.924621899922689
53 0.926582682132721
54 0.923292430241903
55 0.923583900928497
56 0.923292430241903
57 0.925210293134053
58 0.923583900928497
59 0.925210293134053
60 0.923292430241903
61 0.92683668533961
62 0.923583900928497
63 0.924627351760864
64 0.923000959555308
65 0.923000959555308
66 0.923583900928497
67 0.923000959555308
68 0.923292430241903
69 0.923583900928497
70 0.923583900928497
71 0.924621733029683
72 0.923583900928497
73 0.923583900928497
74 0.924918822447459
75 0.924330429236094
76 0.911563050746918
77 0.926291211446126
78 0.913772384325663
79 0.923583900928497
80 0.919341317812602
81 0.925210293134053
82 0.924918822447459
83 0.924918822447459
84 0.913480913639069
85 0.92595682144165
86 0.92595682144165
87 0.925999740759532
88 0.912892520427704
89 0.915398776531219
90 0.913480913639069
91 0.926218418280284
92 0.900708083311717
93 0.915398776531219
94 0.913480913639069
95 0.922340099016825
96 0.921751705805461
97 0.917131984233856
98 0.915398776531219
99 0.915398776531219
100 0.921751705805461
};
\addlegendentry{A2C}
\addplot [semithick, color1]
table {%
1 0.917391939957937
2 0.893735134601593
3 0.928369176387787
4 0.913403868675232
5 0.881280032793681
6 0.904842758178711
7 0.922092696030935
8 0.913173941771189
9 0.911552508672078
10 0.882053593794505
11 0.919121166070302
12 0.877223281065623
13 0.903644506136576
14 0.895649520556132
15 0.924893915653229
16 0.926588149865468
17 0.926732567946116
18 0.92084907690684
19 0.928024895985921
20 0.90300509929657
21 0.915032398700714
22 0.900353260835012
23 0.902990074952443
24 0.91404904127121
25 0.899091947078705
26 0.925257849693298
27 0.922489154338837
28 0.895459878444672
29 0.902996039390564
30 0.894334733486176
31 0.915931260585785
32 0.911435166994731
33 0.921298980712891
34 0.909860912958781
35 0.916818722089132
36 0.919512649377187
37 0.918125911553701
38 0.926833562056224
39 0.922511267662048
40 0.912653028964996
41 0.917856554190318
42 0.904125285148621
43 0.928729323546092
44 0.923400549093882
45 0.906525619824727
46 0.910272725423177
47 0.907428586483002
48 0.910797242323558
49 0.918778196970622
50 0.900753668944041
51 0.917465869585673
52 0.922927192846934
53 0.913506857554118
54 0.918377463022868
55 0.918654251098633
56 0.924610034624735
57 0.930768668651581
58 0.926225193341573
59 0.910062948862712
60 0.930805810292562
61 0.918196562925975
62 0.902306791146596
63 0.908601939678192
64 0.908501255512237
65 0.931351455052694
66 0.910565503438314
67 0.897773396968842
68 0.910506268342336
69 0.919329957167308
70 0.904659565289815
71 0.924862730503082
72 0.901529077688853
73 0.903433068593343
74 0.91377325852712
75 0.914650988578796
76 0.892892404397329
77 0.91377325852712
78 0.898701965808868
79 0.895259539286296
80 0.926143173376719
81 0.922568714618683
82 0.925139685471853
83 0.925793282190959
84 0.91958281993866
85 0.922568714618683
86 0.923876885573069
87 0.908007089296977
88 0.912167000770569
89 0.93069638411204
90 0.926091678937276
91 0.908002463976542
92 0.904659565289815
93 0.926143173376719
94 0.91958281993866
95 0.919823940594991
96 0.901666402816772
97 0.909426828225454
98 0.923898514111837
99 0.904934374491374
100 0.901666402816772
};
\addlegendentry{DQN}
\addplot [semithick, color2]
table {%
1 0.939648303765951
100 0.939648303765951
};
\addlegendentry{Random}
\addplot [semithick, color3]
table {%
1 0.910772966283802
100 0.910772966283802
};
\addlegendentry{ETS}
\addplot [semithick, color4]
table {%
1 0.924058274027314
100 0.924058274027314
};
\addlegendentry{Heur-GD}
\addplot [semithick, color5, dash pattern=on 1pt off 3pt on 3pt off 3pt]
table {%
1 0.924058274027314
100 0.924058274027314
};
\addlegendentry{Heur-LD}
\addplot [semithick, color6, dashed]
table {%
1 0.924058274027314
100 0.924058274027314
};
\addlegendentry{Heur-AT}
