# Supplementary material for: Learn the Time to Learn: Replay Scheduling in Continual Learning
Source: arXiv:2209.08660 source file (2023-11-20)
Supplement: Supplementary file 51 [file rewards_env10.tex]

\nextgroupplot[title=Seed 9,
height=\figheight,
legend cell align={left},
legend style={
  fill opacity=0.8,
  draw opacity=1,
  text opacity=1,
  at={(0.03,0.97)},
  anchor=north west,
  draw=white!80!black
},
minor xtick={25, 75},
minor ytick={},
tick align=outside,
tick pos=left,
width=\figwidth,
x grid style={white!69.0196078431373!black},
xlabel={Eval. Steps},
xminorgrids,
xmajorgrids,
xmin=-3.95, xmax=104.95,
xtick style={color=black},
xtick={-25,0,50,100,125},
xticklabels={-25,0,50,100,125},
y grid style={white!69.0196078431373!black},
ymajorgrids,
ymin=0.737830088791097, ymax=0.952696562415609,
ytick style={color=black},
ytick={0.7,0.75,0.8,0.85,0.9,0.95},
yticklabels={70,75,80,85,90,95}
]
\addplot [semithick, color0]
table {%
1 0.864580869674683
2 0.890737676620483
3 0.890737676620483
4 0.890737676620483
5 0.875396760304769
6 0.854225154717763
7 0.868369205792745
8 0.847537930806478
9 0.852605259418488
10 0.854225154717763
11 0.868369205792745
12 0.858234548568726
13 0.868369205792745
14 0.850215760866801
15 0.860912378629049
16 0.826918341716131
17 0.823584355910619
18 0.788934163252513
19 0.830271579821904
20 0.754264718294144
21 0.757598704099655
22 0.754264718294144
23 0.750930732488632
24 0.747596746683121
25 0.750930732488632
26 0.754264718294144
27 0.747596746683121
28 0.787314267953237
29 0.754264718294144
30 0.792268149058024
31 0.754264718294144
32 0.747596746683121
33 0.747596746683121
34 0.795471624533335
35 0.778237545490265
36 0.747596746683121
37 0.795471624533335
38 0.817509053150813
39 0.795471624533335
40 0.836809041102727
41 0.891221380233765
42 0.84334650238355
43 0.84334650238355
44 0.847002758582433
45 0.891221380233765
46 0.891221380233765
47 0.903750479221344
48 0.902299348513285
49 0.902299348513285
50 0.902299348513285
51 0.902299348513285
52 0.902299348513285
53 0.902299348513285
54 0.903779264291127
55 0.907838332653046
56 0.907838332653046
57 0.907838332653046
58 0.907838332653046
59 0.907838332653046
60 0.907838332653046
61 0.907838332653046
62 0.907838332653046
63 0.909289463361104
64 0.910740594069163
65 0.909289463361104
66 0.905085090796153
67 0.910740594069163
68 0.909289463361104
69 0.907838332653046
70 0.905085090796153
71 0.907838332653046
72 0.907838332653046
73 0.907838332653046
74 0.909289463361104
75 0.905085090796153
76 0.906536221504211
77 0.90233184893926
78 0.909289463361104
79 0.905085090796153
80 0.907838332653046
81 0.905085090796153
82 0.909289463361104
83 0.907838332653046
84 0.906536221504211
85 0.907838332653046
86 0.909289463361104
87 0.906536221504211
88 0.910740594069163
89 0.909289463361104
90 0.906536221504211
91 0.909289463361104
92 0.910740594069163
93 0.907838332653046
94 0.909289463361104
95 0.909289463361104
96 0.907838332653046
97 0.912191724777222
98 0.909289463361104
99 0.906536221504211
100 0.907838332653046
};
%\addlegendentry{a2c, gae, envs=10, lr=0.0001, act=tanh}
\addplot [semithick, color1]
table {%
1 0.82398406068484
2 0.819590324163437
3 0.805619784196218
4 0.842099557320277
5 0.847449709971746
6 0.862992805242539
7 0.862818151712418
8 0.815620054801305
9 0.838435190916062
10 0.828719919919968
11 0.837833952903748
12 0.83437171181043
13 0.809042167663574
14 0.811566481987635
15 0.802314128478368
16 0.768619201580683
17 0.76221762696902
18 0.775513849655787
19 0.821620704730352
20 0.788659310340881
21 0.755245093504588
22 0.80042626063029
23 0.796455224355062
24 0.784978888432185
25 0.830409242709478
26 0.766947452227275
27 0.794648689031601
28 0.819959839185079
29 0.821937431891759
30 0.774133729934692
31 0.78890484770139
32 0.820355375607808
33 0.78890484770139
34 0.824500423669815
35 0.754527072111766
36 0.763281941413879
37 0.754268834988276
38 0.772821555534999
39 0.763281941413879
40 0.783529005448024
41 0.784274286031723
42 0.797616587082545
43 0.799387564261754
44 0.808817382653554
45 0.822072672843933
46 0.780172135432561
47 0.798758753140767
48 0.767593346039454
49 0.810347509384155
50 0.82993229230245
51 0.814422140518824
52 0.817668300867081
53 0.815709577004115
54 0.830520842472712
55 0.818913745880127
56 0.76557908654213
57 0.833521642287572
58 0.832544392347336
59 0.863667800029119
60 0.826702016592026
61 0.792052586873372
62 0.78453009724617
63 0.859827069441478
64 0.797461128234863
65 0.803748973210653
66 0.814349021514257
67 0.833525441090266
68 0.822327238321304
69 0.836811979611715
70 0.765421374638875
71 0.785058705012004
72 0.801098960638046
73 0.83154648343722
74 0.805435031652451
75 0.83154648343722
76 0.787536863485972
77 0.849995064735413
78 0.786743950843811
79 0.784296961625417
80 0.799439497788747
81 0.787542967001597
82 0.794803486267726
83 0.787542967001597
84 0.808187987407048
85 0.799438212315242
86 0.810539462169012
87 0.748970190684001
88 0.801836121082306
89 0.846956340471903
90 0.841425973176956
91 0.829928729931514
92 0.833457630872727
93 0.815532783667246
94 0.828041472037633
95 0.815532783667246
96 0.819186894098918
97 0.828615017731984
98 0.794450050592422
99 0.810692767302195
100 0.815824488798777
};
%\addlegendentry{DQN, n train envs=30}
\addplot [semithick, color2]
table {%
1 0.917741544938917
100 0.917741544938917
};
%\addlegendentry{Random}
\addplot [semithick, color3]
table {%
1 0.942929904523586
100 0.942929904523586
};
%\addlegendentry{ETS}
\addplot [semithick, color4]
table {%
1 0.790914223232021
100 0.790914223232021
};
%\addlegendentry{Heur-GD}
\addplot [semithick, color5, dash pattern=on 1pt off 3pt on 3pt off 3pt]
table {%
1 0.790914223232021
100 0.790914223232021
};
%\addlegendentry{Heur-LD}
\addplot [semithick, color6, dashed]
table {%
1 0.790914223232021
100 0.790914223232021
};
%\addlegendentry{Heur-AT}
