# Supplementary material for: Learn the Time to Learn: Replay Scheduling in Continual Learning
Source: arXiv:2209.08660 source file (2023-11-20)
Supplement: Supplementary file 52 [file rewards_env2.tex]

\nextgroupplot[title=Seed 1,
height=\figheight,
legend cell align={left},
legend style={
  fill opacity=0.8,
  draw opacity=1,
  text opacity=1,
  at={(0.5,0.09)},
  anchor=south,
  draw=white!80!black
},
minor xtick={25, 75},
minor ytick={},
tick align=outside,
tick pos=left,
width=\figwidth,
x grid style={white!69.0196078431373!black},
xlabel={Eval. Steps},
xminorgrids,
xmajorgrids,
xmin=-3.95, xmax=104.95,
xtick style={color=black},
xtick={-25,0,50,100,125},
xticklabels={-25,0,50,100,125},
y grid style={white!69.0196078431373!black},
ymajorgrids,
ymin=0.899988176226616, ymax=0.949457623759906,
ytick style={color=black},
ytick={0.89,0.9,0.91,0.92,0.93,0.94,0.95},
yticklabels={89,90,91,92,93,94,95}
]
\addplot [semithick, color0]
table {%
1 0.928993729750315
2 0.921653783321381
3 0.921653783321381
4 0.921653783321381
5 0.902236787478129
6 0.921563911437988
7 0.939947307109833
8 0.926932243506114
9 0.933179255326589
10 0.925797196229299
11 0.939947307109833
12 0.927453283468882
13 0.939947307109833
14 0.924141108989716
15 0.924662148952484
16 0.933640118439992
17 0.929370228449504
18 0.931287173430125
19 0.928235181172689
20 0.939305913448334
21 0.947209012508392
22 0.939887130260468
23 0.93860905567805
24 0.934339165687561
25 0.938669232527415
26 0.942878945668538
27 0.930766133467356
28 0.93509620030721
29 0.939305913448334
30 0.942172876993815
31 0.942939122517904
32 0.934339165687561
33 0.930766133467356
34 0.939366090297699
35 0.930766133467356
36 0.939305913448334
37 0.942878945668538
38 0.930766133467356
39 0.935750730832418
40 0.937000735600789
41 0.931074758370717
42 0.928604666392009
43 0.940329245726268
44 0.933692375818888
45 0.937187381585439
46 0.938573861122131
47 0.934218136469523
48 0.935265040397644
49 0.941492362817129
50 0.937470920880636
51 0.93636798063914
52 0.938573861122131
53 0.937512346108754
54 0.936424016952515
55 0.937470920880636
56 0.938213805357615
57 0.936236683527629
58 0.938573861122131
59 0.936236683527629
60 0.936236683527628
61 0.936105386416117
62 0.938573861122131
63 0.933039935429891
64 0.934274172782898
65 0.936424016952515
66 0.937470920880636
67 0.933452359835307
68 0.936424016952515
69 0.938573861122131
70 0.935150078932444
71 0.937470920880636
72 0.938573861122131
73 0.938573861122131
74 0.935189779599508
75 0.936465442180634
76 0.929849628607432
77 0.935321076711019
78 0.928615391254425
79 0.93625301917394
80 0.936105386416117
81 0.935018781820933
82 0.928615391254425
83 0.937339623769124
84 0.928388833999634
85 0.937339623769124
86 0.929849628607432
87 0.934144600232442
88 0.928388833999634
89 0.933133729298909
90 0.932047124703725
91 0.928656816482544
92 0.926877971490224
93 0.936146811644236
94 0.930126253763835
95 0.92993247906367
96 0.937381048997243
97 0.918975551923116
98 0.928656816482544
99 0.923876829942067
100 0.937381048997243
};
%\addlegendentry{a2c, gae, envs=10, lr=0.0001, act=tanh}
\addplot [semithick, color1]
table {%
1 0.917090237140656
2 0.941090885798136
3 0.935193920135498
4 0.92663596868515
5 0.933226803938548
6 0.940216020743052
7 0.938880399862925
8 0.93150053024292
9 0.927185396353404
10 0.927726697921753
11 0.939616942405701
12 0.934015727043152
13 0.933697092533112
14 0.938335784276326
15 0.922370894749959
16 0.941266016165415
17 0.926876668135325
18 0.936521116892497
19 0.939547340075175
20 0.937949856122335
21 0.936437372366587
22 0.935050892829895
23 0.938372600078583
24 0.932349522908529
25 0.941066837310791
26 0.934335390726725
27 0.936019655068715
28 0.936847595373789
29 0.930208420753479
30 0.938615389664968
31 0.933179974555969
32 0.935184590021769
33 0.937681245803833
34 0.934714301427205
35 0.935290797551473
36 0.936282928784688
37 0.934310408433278
38 0.943678450584412
39 0.933089526494344
40 0.935127401351929
41 0.933108162879944
42 0.937339150905609
43 0.937936814626058
44 0.940008421738943
45 0.935417489210765
46 0.932427871227264
47 0.932951994736989
48 0.933705945809682
49 0.928139122327169
50 0.939642028013865
51 0.936670482158661
52 0.940031087398529
53 0.940705267588298
54 0.939265529314677
55 0.939835011959076
56 0.938107804457347
57 0.935274358590444
58 0.93172158797582
59 0.934811182816823
60 0.935215079784393
61 0.935780636469523
62 0.938767846425374
63 0.942241807778676
64 0.933221395810445
65 0.933172957102458
66 0.938112421830495
67 0.935823575655619
68 0.937325700124105
69 0.932510618368785
70 0.943464310963949
71 0.942089347044627
72 0.941985551516215
73 0.943289176623026
74 0.944119735558828
75 0.93965988556544
76 0.93918027083079
77 0.940389426549276
78 0.940416924158732
79 0.938562353452047
80 0.935225911935171
81 0.939959983030955
82 0.937595415115356
83 0.941985551516215
84 0.940416924158732
85 0.93918027083079
86 0.938146829605103
87 0.940416924158732
88 0.938398373126984
89 0.937329840660095
90 0.938716312249502
91 0.942265164852142
92 0.943464310963949
93 0.941005158424378
94 0.94091770251592
95 0.943162020047506
96 0.943162020047506
97 0.94087317387263
98 0.94271680911382
99 0.944096378485362
100 0.944096378485362
};
%\addlegendentry{DQN, n train envs=30}
\addplot [semithick, color2]
table {%
1 0.921745991773276
100 0.921745991773276
};
%\addlegendentry{Random}
\addplot [semithick, color3]
table {%
1 0.924611906166864
100 0.924611906166864
};
%\addlegendentry{ETS}
\addplot [semithick, color4]
table {%
1 0.911768768911962
100 0.911768768911962
};
%\addlegendentry{Heur-GD}
\addplot [semithick, color5, dash pattern=on 1pt off 3pt on 3pt off 3pt]
table {%
1 0.911768768911962
100 0.911768768911962
};
%\addlegendentry{Heur-LD}
\addplot [semithick, color6, dashed]
table {%
1 0.911768768911962
100 0.911768768911962
};
%\addlegendentry{Heur-AT}
