# Supplementary material for: Learn the Time to Learn: Replay Scheduling in Continual Learning
Source: arXiv:2209.08660 source file (2023-11-20)
Supplement: Supplementary file 53 [file rewards_env3.tex]

\nextgroupplot[title=Seed 2,
height=\figheight,
legend cell align={left},
legend style={
  fill opacity=0.8,
  draw opacity=1,
  text opacity=1,
  at={(0.5,0.09)},
  anchor=south,
  draw=white!80!black
},
minor xtick={25, 75},
minor ytick={},
tick align=outside,
tick pos=left,
width=\figwidth,
x grid style={white!69.0196078431373!black},
xlabel={Eval. Steps},
xminorgrids,
xmajorgrids,
xmin=-3.95, xmax=104.95,
xtick style={color=black},
xtick={-25,0,50,100,125},
xticklabels={-25,0,50,100,125},
y grid style={white!69.0196078431373!black},
ymajorgrids,
ymin=0.819999375325716, ymax=0.9482612031612,
ytick style={color=black},
ytick={0.8,0.82,0.84,0.86,0.88,0.9,0.92,0.94,0.96},
yticklabels={80,82,84,86,88,90,92,94,96}
]
\addplot [semithick, color0]
table {%
1 0.901102566719055
2 0.902243876457214
3 0.902243876457214
4 0.902243876457214
5 0.876675689220428
6 0.914959967136383
7 0.870579195022583
8 0.923964730898539
9 0.896327006816864
10 0.914959967136383
11 0.870579195022583
12 0.925854643185933
13 0.870579195022583
14 0.904065291086833
15 0.905955203374227
16 0.923574550946554
17 0.915542340278625
18 0.905230037371318
19 0.906537576516469
20 0.919404546419779
21 0.902661498387655
22 0.896006862322489
23 0.911954708894094
24 0.903922498226166
25 0.911954708894094
26 0.919986919562022
27 0.903340125083923
28 0.886014703909556
29 0.915544891357422
30 0.904208771387736
31 0.915544891357422
32 0.899892326196035
33 0.899309953053792
34 0.911787990729014
35 0.885553630193075
36 0.912199846903483
37 0.912473118305206
38 0.900137464205424
39 0.904167636235555
40 0.909707697232564
41 0.916748428344727
42 0.916748428344727
43 0.916748428344727
44 0.908442946275075
45 0.916748428344727
46 0.916748428344727
47 0.916748428344727
48 0.910016592343648
49 0.916748428344727
50 0.916748428344727
51 0.913687610626221
52 0.916748428344727
53 0.913687610626221
54 0.899766270319621
55 0.916748428344727
56 0.916748428344727
57 0.916748428344727
58 0.913687610626221
59 0.910016592343648
60 0.910016592343648
61 0.903725504875183
62 0.906955774625142
63 0.910016592343648
64 0.906955774625142
65 0.906955774625142
66 0.906955774625142
67 0.90328475634257
68 0.903894956906636
69 0.910016592343648
70 0.90328475634257
71 0.916748428344727
72 0.910016592343648
73 0.896552920341492
74 0.90328475634257
75 0.890905725955963
76 0.896095252037048
77 0.90328475634257
78 0.90328475634257
79 0.90328475634257
80 0.90328475634257
81 0.90328475634257
82 0.90328475634257
83 0.90328475634257
84 0.896552920341492
85 0.910016592343648
86 0.902827088038127
87 0.90328475634257
88 0.896552920341492
89 0.90328475634257
90 0.902827088038127
91 0.896552920341492
92 0.902827088038127
93 0.90328475634257
94 0.906955774625142
95 0.869561115900675
96 0.90328475634257
97 0.889804164568583
98 0.896552920341492
99 0.875208310286204
100 0.910016592343648
};
%\addlegendentry{a2c, gae, envs=10, lr=0.0001, act=tanh}
\addplot [semithick, color1]
table {%
1 0.895822556813558
2 0.883807682991028
3 0.871220616499583
4 0.92232936223348
5 0.894194694360097
6 0.910101052125295
7 0.92542005777359
8 0.909507513046265
9 0.917677895228068
10 0.90328106880188
11 0.905240313212077
12 0.901160271962484
13 0.922922551631927
14 0.912497993310292
15 0.904860631624858
16 0.91266002257665
17 0.895391122500102
18 0.896006306012472
19 0.890017557144165
20 0.931374529997508
21 0.917277419567108
22 0.907385925451914
23 0.919625488917033
24 0.936748441060384
25 0.926673523585002
26 0.918082030614217
27 0.941581237316132
28 0.934482284386953
29 0.925168752670288
30 0.912477318445842
31 0.941581237316132
32 0.933137504259745
33 0.934125113487244
34 0.926815799872081
35 0.941889190673828
36 0.935494307676951
37 0.934125113487244
38 0.932624876499176
39 0.941273283958435
40 0.941273283958435
41 0.941581237316132
42 0.924422204494476
43 0.941581237316132
44 0.932457848389943
45 0.94090158144633
46 0.923742548624674
47 0.940593628088633
48 0.91470011472702
49 0.915687723954519
50 0.924869028727214
51 0.931198672453562
52 0.915474073092143
53 0.924095070362091
54 0.935943547884623
55 0.919444990158081
56 0.908764052391052
57 0.925287600358327
58 0.934762060642242
59 0.940593628088633
60 0.925791398684184
61 0.902621408303579
62 0.934950228532155
63 0.917983150482178
64 0.940593628088633
65 0.930694874127706
66 0.931682483355204
67 0.94090158144633
68 0.932970317204793
69 0.931274282932281
70 0.94090158144633
71 0.94090158144633
72 0.94090158144633
73 0.942431120077769
74 0.94090158144633
75 0.94090158144633
76 0.94090158144633
77 0.939913972218831
78 0.94090158144633
79 0.939913972218831
80 0.939238556226095
81 0.94090158144633
82 0.94090158144633
83 0.938166677951813
84 0.918970759709676
85 0.918970759709676
86 0.938166677951813
87 0.938166677951813
88 0.932970317204793
89 0.938166677951813
90 0.938166677951813
91 0.937179068724314
92 0.916235856215159
93 0.930795391400655
94 0.919958368937174
95 0.939913972218831
96 0.938926362991333
97 0.909594384829203
98 0.916053553422292
99 0.938166677951813
100 0.933530294895172
};
%\addlegendentry{DQN, n train envs=30}
\addplot [semithick, color2]
table {%
1 0.870293399244796
100 0.870293399244796
};
%\addlegendentry{Random}
\addplot [semithick, color3]
table {%
1 0.912342344433749
100 0.912342344433749
};
%\addlegendentry{ETS}
\addplot [semithick, color4]
table {%
1 0.825829458409147
100 0.825829458409147
};
%\addlegendentry{Heur-GD}
\addplot [semithick, color5, dash pattern=on 1pt off 3pt on 3pt off 3pt]
table {%
1 0.825829458409147
100 0.825829458409147
};
%\addlegendentry{Heur-LD}
\addplot [semithick, color6, dashed]
table {%
1 0.825829458409147
100 0.825829458409147
};
%\addlegendentry{Heur-AT}
