# Supplementary material for: Learn the Time to Learn: Replay Scheduling in Continual Learning
Source: arXiv:2209.08660 source file (2023-11-20)
Supplement: Supplementary file 54 [file rewards_env4.tex]

\nextgroupplot[title=Seed 3,
height=\figheight,
legend cell align={left},
legend style={
  fill opacity=0.8,
  draw opacity=1,
  text opacity=1,
  at={(0.5,0.09)},
  anchor=south,
  draw=white!80!black
},
minor xtick={25, 75},
minor ytick={},
tick align=outside,
tick pos=left,
width=\figwidth,
x grid style={white!69.0196078431373!black},
xlabel={Eval. Steps},
xminorgrids,
xmajorgrids,
xmin=-3.95, xmax=104.95,
xtick style={color=black},
xtick={-25,0,50,100,125},
xticklabels={-25,0,50,100,125},
y grid style={white!69.0196078431373!black},
ymajorgrids,
ymin=0.889578813913873, ymax=0.955645133384438,
ytick style={color=black},
ytick={0.88,0.89,0.9,0.91,0.92,0.93,0.94,0.95,0.96},
yticklabels={88,89,90,91,92,93,94,95,96}
]
\addplot [semithick, color0]
table {%
1 0.917372953891754
2 0.901369512081146
3 0.901369512081146
4 0.901369512081146
5 0.905200250943502
6 0.93375430504481
7 0.9278972864151
8 0.931276913483937
9 0.924610249201457
10 0.93375430504481
11 0.9278972864151
12 0.941230614980062
13 0.9278972864151
14 0.926277995109558
15 0.936231696605682
16 0.940860247612
17 0.942041341463725
18 0.942852067947388
19 0.944518733024597
20 0.930536178747813
21 0.931345824400584
22 0.937249135971069
23 0.940004309018453
24 0.941185402870178
25 0.940004309018453
26 0.938823215166728
27 0.932898366451263
28 0.92542097568512
29 0.93558247089386
30 0.93919358253479
31 0.93558247089386
32 0.941185402870178
33 0.932898366451263
34 0.924958010514577
35 0.932898366451263
36 0.924356162548065
37 0.933245046933492
38 0.932898366451263
39 0.932898366451263
40 0.936254306634267
41 0.932898366451263
42 0.940490961074829
43 0.940490961074829
44 0.940490961074829
45 0.932898366451263
46 0.943515288829804
47 0.944209730625153
48 0.941185402870178
49 0.942372949918111
50 0.944209730625153
51 0.941185402870178
52 0.940328375498454
53 0.939348622163137
54 0.937874674797058
55 0.947234058380127
56 0.944209730625153
57 0.947234058380127
58 0.941185402870178
59 0.942372949918111
60 0.947234058380127
61 0.944563945134481
62 0.943398996194204
63 0.943398996194204
64 0.943398996194204
65 0.950258386135101
66 0.947234058380127
67 0.950258386135101
68 0.936539606253306
69 0.945397277673086
70 0.936539606253306
71 0.943398996194204
72 0.943398996194204
73 0.950258386135101
74 0.943398996194204
75 0.943398996194204
76 0.950258386135101
77 0.943398996194204
78 0.950258386135101
79 0.943398996194204
80 0.943398996194204
81 0.943398996194204
82 0.950258386135101
83 0.943398996194204
84 0.950258386135101
85 0.950258386135101
86 0.943398996194204
87 0.943398996194204
88 0.950258386135101
89 0.943398996194204
90 0.943398996194204
91 0.943398996194204
92 0.950258386135101
93 0.943398996194204
94 0.950258386135101
95 0.950258386135101
96 0.943398996194204
97 0.950258386135101
98 0.950258386135101
99 0.936539606253306
100 0.950258386135101
};
%\addlegendentry{a2c, gae, envs=10, lr=0.0001, act=tanh}
\addplot [semithick, color1]
table {%
1 0.901369512081146
2 0.926092799504598
3 0.924642546971639
4 0.916640830039978
5 0.93488910595576
6 0.929757754007975
7 0.925698745250702
8 0.916848619778951
9 0.923376397291819
10 0.932411714394887
11 0.926569759845734
12 0.915544792016347
13 0.930582463741302
14 0.932511838277181
15 0.918268740177155
16 0.922350339094798
17 0.923022182782491
18 0.915127038955688
19 0.926208011309306
20 0.923353787263234
21 0.93111541668574
22 0.92620800336202
23 0.927998491128286
24 0.916978887716929
25 0.938754300276438
26 0.933576651414235
27 0.925243314107259
28 0.925937755902608
29 0.91777454217275
30 0.922195299466451
31 0.914872952302297
32 0.928915802637736
33 0.928352709611257
34 0.923291341463725
35 0.916046504179637
36 0.903646632035573
37 0.919919244448344
38 0.930967903137207
39 0.922295431296031
40 0.919941858450572
41 0.931378126144409
42 0.915768730640412
43 0.923754306634267
44 0.921686041355133
45 0.921061583360036
46 0.918122311433156
47 0.917474162578583
48 0.918415160973867
49 0.915852705637614
50 0.929587642351786
51 0.920830102761586
52 0.92366171280543
53 0.929163432121277
54 0.913831822077433
55 0.929865415891011
56 0.940713818868001
57 0.937797156969706
58 0.929526269435883
59 0.907256674766541
60 0.920089364051819
61 0.933715542157491
62 0.928808132807414
63 0.915521097183228
64 0.932342807451884
65 0.925127037366231
66 0.929865415891011
67 0.933854432900747
68 0.926223079363505
69 0.934826652208964
70 0.933159987131755
71 0.90748815536499
72 0.915945299466451
73 0.930628760655721
74 0.905250859260559
75 0.926585912704468
76 0.937889738877614
77 0.929764207204183
78 0.927326651414235
79 0.924032084147135
80 0.897922046979268
81 0.930628760655721
82 0.924387379487356
83 0.917919890085856
84 0.913584188620249
85 0.931161709626516
86 0.906555771827698
87 0.938630485534668
88 0.892581828435262
89 0.932133932908376
90 0.909170977274577
91 0.922010111808777
92 0.936400727430979
93 0.905220715204875
94 0.926192935307821
95 0.89775839249293
96 0.933676783243815
97 0.909341084957123
98 0.924000859260559
99 0.918213824431101
100 0.92792850335439
};
%\addlegendentry{DQN, n train envs=30}
\addplot [semithick, color2]
table {%
1 0.896216623600344
100 0.896216623600344
};
%\addlegendentry{Random}
\addplot [semithick, color3]
table {%
1 0.893317183462532
100 0.893317183462532
};
%\addlegendentry{ETS}
\addplot [semithick, color4]
table {%
1 0.952642118863049
100 0.952642118863049
};
%\addlegendentry{Heur-GD}
\addplot [semithick, color5, dash pattern=on 1pt off 3pt on 3pt off 3pt]
table {%
1 0.952642118863049
100 0.952642118863049
};
%\addlegendentry{Heur-LD}
\addplot [semithick, color6, dashed]
table {%
1 0.952642118863049
100 0.952642118863049
};
%\addlegendentry{Heur-AT}
