# Supplementary material for: Learn the Time to Learn: Replay Scheduling in Continual Learning
Source: arXiv:2209.08660 source file (2023-11-20)
Supplement: Supplementary file 55 [file rewards_env5.tex]

\nextgroupplot[title=Seed 4,
height=\figheight,
legend cell align={left},
legend style={
  fill opacity=0.8,
  draw opacity=1,
  text opacity=1,
  at={(0.03,0.03)},
  anchor=south west,
  draw=white!80!black
},
minor xtick={25, 75},
minor ytick={},
tick align=outside,
tick pos=left,
width=\figwidth,
x grid style={white!69.0196078431373!black},
xlabel={Eval. Steps},
xminorgrids,
xmajorgrids,
xmin=-3.95, xmax=104.95,
xtick style={color=black},
xtick={-25,0,50,100,125},
xticklabels={-25,0,50,100,125},
y grid style={white!69.0196078431373!black},
ylabel={ACC (\%)},
ymajorgrids,
ymin=0.90, ymax=0.95,
ytick style={color=black},
ytick={0.9,0.91,0.92,0.93,0.94,0.95},
yticklabels={90,91,92,93,94,95}
]
\addplot [semithick, color0]
table {%
1 0.914315195878347
2 0.902619230747223
3 0.902619230747223
4 0.902619230747223
5 0.923831009864807
6 0.934635249773661
7 0.937834147612254
8 0.936086698373159
9 0.937076163291931
10 0.934635249773661
11 0.937834147612254
12 0.935855217774709
13 0.937834147612254
14 0.933415281772613
15 0.933183801174164
16 0.938786156972249
17 0.936525396505992
18 0.937195575237274
19 0.933183801174164
20 0.941948576768239
21 0.94415800968806
22 0.939775621891022
23 0.941577963034312
24 0.937427055835724
25 0.937746342023214
26 0.941948576768239
27 0.935536909103393
28 0.937746342023214
29 0.941948576768239
30 0.931035117308299
31 0.938536890347799
32 0.939317202568054
33 0.935536909103393
34 0.937746342023214
35 0.935536909103393
36 0.937797669569651
37 0.937427055835724
38 0.937427055835724
39 0.932605977853139
40 0.939456335703532
41 0.937427055835724
42 0.935536909103393
43 0.939317202568054
44 0.939317202568054
45 0.937427055835724
46 0.936776546637217
47 0.939317202568054
48 0.937427055835724
49 0.941577963034312
50 0.939317202568054
51 0.937427055835724
52 0.938898173967997
53 0.934651017189026
54 0.938527401288351
55 0.938898173967997
56 0.930484350522359
57 0.937008027235667
58 0.934651017189026
59 0.935073947906494
60 0.934886399904887
61 0.931328463554382
62 0.939317202568054
63 0.937427055835724
64 0.932367936770121
65 0.936244320869446
66 0.937427055835724
67 0.936244320869446
68 0.934122693538666
69 0.924999642372131
70 0.924999642372131
71 0.915107309818268
72 0.924999642372131
73 0.925418670972188
74 0.939845359325409
75 0.931529879570007
76 0.933315122127533
77 0.924999642372131
78 0.931097741921743
79 0.924999642372131
80 0.924999642372131
81 0.915107309818268
82 0.931529879570007
83 0.935280172030131
84 0.939845359325409
85 0.922489472230275
86 0.935825292269389
87 0.922489472230275
88 0.94414077202479
89 0.921869027614593
90 0.924567504723867
91 0.924381776650747
92 0.930665604273478
93 0.923481102784475
94 0.929019709428151
95 0.912730785210927
96 0.934091031551361
97 0.934636151790619
98 0.927969706058502
99 0.928317797183991
100 0.930259831746419
};
%\addlegendentry{a2c, gae, envs=10, lr=0.0001, act=tanh}
\addplot [semithick, color1]
table {%
1 0.913430353005727
2 0.926380228996277
3 0.927857907613118
4 0.926647575696309
5 0.92497315009435
6 0.93016722202301
7 0.931838766733805
8 0.92684633731842
9 0.930871152877808
10 0.925254627068838
11 0.925844669342041
12 0.931430149078369
13 0.930891652901967
14 0.930147123336792
15 0.928239472707113
16 0.928872545560201
17 0.923749049504598
18 0.932359552383423
19 0.933897356192271
20 0.925131603082021
21 0.917210336526235
22 0.922892391681671
23 0.936214824517568
24 0.925836368401845
25 0.927980319658915
26 0.923626108964284
27 0.927355738480886
28 0.924304509162903
29 0.915823407967885
30 0.929792054494222
31 0.922065444787343
32 0.925773390134176
33 0.924978446960449
34 0.928726021448771
35 0.927858885129293
36 0.92255740960439
37 0.926624898115794
38 0.909767353534699
39 0.923485147953033
40 0.930620896816254
41 0.920959365367889
42 0.917286554972331
43 0.92255740960439
44 0.922251160939534
45 0.923791396617889
46 0.920166993141174
47 0.923791396617889
48 0.933115112781525
49 0.915377644697825
50 0.918933006127675
51 0.920910958449046
52 0.925953125953674
53 0.927187112967173
54 0.92635946671168
55 0.928120358784993
56 0.928752601146698
57 0.926623515288035
58 0.925591993331909
59 0.918549704551697
60 0.92028751373291
61 0.92481183608373
62 0.911718797683716
63 0.923216716448466
64 0.931974649429321
65 0.921557223796844
66 0.929473125934601
67 0.924181763331095
68 0.922413961092631
69 0.91725873152415
70 0.918061486879985
71 0.923480765024821
72 0.921557223796844
73 0.916487709681193
74 0.915231549739838
75 0.915819346904755
76 0.914003137747447
77 0.922106726964315
78 0.918711996078491
79 0.923043048381805
80 0.922750600179036
81 0.92224029302597
82 0.919655283292135
83 0.92447935740153
84 0.917734738190969
85 0.924181763331095
86 0.927064780394236
87 0.922522270679474
88 0.928778680165609
89 0.923043048381805
90 0.926598409811656
91 0.918966909249624
92 0.922522270679474
93 0.920035529136658
94 0.930163657665253
95 0.911529584725698
96 0.912463740507762
97 0.919979381561279
98 0.925044151147207
99 0.912325855096181
100 0.914703710873922
};
%\addlegendentry{DQN, n train envs=30}
\addplot [semithick, color2]
table {%
1 0.911614472409506
100 0.911614472409506
};
%\addlegendentry{Random}
\addplot [semithick, color3]
table {%
1 0.905164085947425
100 0.905164085947425
};
%\addlegendentry{ETS}
\addplot [semithick, color4]
table {%
1 0.916400743643145
100 0.916400743643145
};
%\addlegendentry{Heur-GD}
\addplot [semithick, color5, dash pattern=on 1pt off 3pt on 3pt off 3pt]
table {%
1 0.92662679292127
100 0.92662679292127
};
%\addlegendentry{Heur-LD}
\addplot [semithick, color6, dashed]
table {%
1 0.916400743643145
100 0.916400743643145
};
%\addlegendentry{Heur-AT}
