# Supplementary material for: Learn the Time to Learn: Replay Scheduling in Continual Learning
Source: arXiv:2209.08660 source file (2023-11-20)
Supplement: Supplementary file 56 [file rewards_env6.tex]

\nextgroupplot[title=Seed 5,
height=\figheight,
legend cell align={left},
legend style={
  fill opacity=0.8,
  draw opacity=1,
  text opacity=1,
  at={(0.97,0.03)},
  anchor=south east,
  draw=white!80!black
},
minor xtick={25, 75},
minor ytick={},
tick align=outside,
tick pos=left,
width=\figwidth,
x grid style={white!69.0196078431373!black},
xlabel={Eval. Steps},
xminorgrids,
xmajorgrids,
xmin=-3.95, xmax=104.95,
xtick style={color=black},
xtick={-25,0,50,100,125},
xticklabels={-25,0,50,100,125},
y grid style={white!69.0196078431373!black},
ymajorgrids,
ymin=0.90, ymax=0.95,
ytick style={color=black},
ytick={0.9,0.91,0.92,0.93,0.94,0.95},
yticklabels={90,91,92,93,94,95}
]
\addplot [semithick, color0]
table {%
1 0.931729527314504
2 0.937117218971252
3 0.937117218971252
4 0.937117218971252
5 0.942877070109049
6 0.934570733706157
7 0.929683101177216
8 0.942782874902089
9 0.937807408968608
10 0.934570733706157
11 0.929683101177216
12 0.939634033044179
13 0.929683101177216
14 0.929507434368134
15 0.926358592510223
16 0.938103334108988
17 0.93698548078537
18 0.93433692852656
19 0.928773339589437
20 0.939721477031708
21 0.939809310436249
22 0.93869145711263
23 0.941018370787303
24 0.939900517463684
25 0.941018370787303
26 0.942136224110921
27 0.937485770384471
28 0.935158856709798
29 0.942136224110921
30 0.937474048137665
31 0.939809310436249
32 0.942136224110921
33 0.937573603789012
34 0.936276710033417
35 0.937485770384471
36 0.939809310436249
37 0.94325407743454
38 0.939721477031708
39 0.938206644852956
40 0.940855197111766
41 0.934674044450124
42 0.939324498176575
43 0.93539491891861
44 0.935028020540873
45 0.931465339660644
46 0.931465339660644
47 0.9312779545784
48 0.931465339660644
49 0.934177509943644
50 0.931465339660644
51 0.931465339660644
52 0.931465339660644
53 0.931465339660644
54 0.9312779545784
55 0.931465339660644
56 0.931465339660644
57 0.931465339660644
58 0.931465339660644
59 0.931465339660644
60 0.931465339660644
61 0.933546725908915
62 0.931465339660644
63 0.931090569496155
64 0.931090569496155
65 0.9312779545784
66 0.931465339660644
67 0.931090569496155
68 0.9312779545784
69 0.931465339660644
70 0.931465339660644
71 0.931465339660644
72 0.931465339660644
73 0.931465339660644
74 0.9312779545784
75 0.9312779545784
76 0.929871662457784
77 0.9312779545784
78 0.9312779545784
79 0.931465339660644
80 0.931465339660644
81 0.925737639268239
82 0.9312779545784
83 0.931465339660644
84 0.933171955744426
85 0.93335934082667
86 0.9312779545784
87 0.931090569496155
88 0.931090569496155
89 0.935440727074941
90 0.9312779545784
91 0.9312779545784
92 0.931090569496155
93 0.933546725908915
94 0.9312779545784
95 0.930262192090352
96 0.929502296447754
97 0.929127526283264
98 0.933665068944295
99 0.931583682696025
100 0.928180805842082
};
%\addlegendentry{a2c, gae, envs=10, lr=0.0001, act=tanh}
\addplot [semithick, color1]
table {%
1 0.938462579250336
2 0.929322858651479
3 0.93185932636261
4 0.919784116744995
5 0.923728128274282
6 0.919772783915202
7 0.940860076745351
8 0.926340981324514
9 0.935865338643392
10 0.943523891766866
11 0.928873646259308
12 0.932237732410431
13 0.946447324752808
14 0.938856673240662
15 0.935454722245534
16 0.926658300558726
17 0.931981674830119
18 0.935190240542094
19 0.916622002919515
20 0.919737533728282
21 0.913096984227498
22 0.922481528917948
23 0.908880762259165
24 0.911864976088206
25 0.908803669611613
26 0.9075230717659
27 0.914152542750041
28 0.916906170050303
29 0.938629158337911
30 0.921688520908356
31 0.931728839874268
32 0.942857221762339
33 0.93785594701767
34 0.930912121136983
35 0.932871409257253
36 0.927952154477437
37 0.927952154477437
38 0.932871409257253
39 0.938629158337911
40 0.934254634380341
41 0.934254634380341
42 0.924203590552012
43 0.91836435397466
44 0.937225651741028
45 0.93217324813207
46 0.933058794339498
47 0.93217324813207
48 0.940622886021932
49 0.91836435397466
50 0.934254634380341
51 0.928101881345113
52 0.928415397802989
53 0.937099472681681
54 0.933337430159251
55 0.935110624631246
56 0.932451883951823
57 0.914488629500071
58 0.926863654454549
59 0.925524310270945
60 0.92686740954717
61 0.936768265565236
62 0.925134134292603
63 0.928985778490702
64 0.932591048876445
65 0.932025988896688
66 0.917664090792338
67 0.939527535438538
68 0.933797895908356
69 0.918236402670542
70 0.93553394873937
71 0.937721188863118
72 0.944841833909353
73 0.928742865721385
74 0.944841833909353
75 0.934656186898549
76 0.921211969852448
77 0.929280662536621
78 0.937721188863118
79 0.942302890618642
80 0.937181663513183
81 0.92693882783254
82 0.943035491307577
83 0.934801348050435
84 0.943035491307577
85 0.925608591238658
86 0.935625203450521
87 0.935903628667196
88 0.923314925034841
89 0.934097286065419
90 0.917586783568064
91 0.931163505713145
92 0.923850417137146
93 0.925524310270945
94 0.930219646294912
95 0.923604933420817
96 0.934097286065419
97 0.925742328166962
98 0.927723395824433
99 0.927723395824433
100 0.927723395824433
};
%\addlegendentry{DQN, n train envs=30}
\addplot [semithick, color2]
table {%
1 0.919256607570398
100 0.919256607570398
};
%\addlegendentry{Random}
\addplot [semithick, color3]
table {%
1 0.907289510340143
100 0.907289510340143
};
%\addlegendentry{ETS}
\addplot [semithick, color4]
table {%
1 0.917972439382205
100 0.917972439382205
};
%\addlegendentry{Heur-GD}
\addplot [semithick, color5, dash pattern=on 1pt off 3pt on 3pt off 3pt]
table {%
1 0.917972439382205
100 0.917972439382205
};
%\addlegendentry{Heur-LD}
\addplot [semithick, color6, dashed]
table {%
1 0.917972439382205
100 0.917972439382205
};
%\addlegendentry{Heur-AT}
