# Supplementary material for: Learn the Time to Learn: Replay Scheduling in Continual Learning
Source: arXiv:2209.08660 source file (2023-11-20)
Supplement: Supplementary file 57 [file rewards_env7.tex]

\nextgroupplot[title=Seed 6,
height=\figheight,
legend cell align={left},
legend style={fill opacity=0.8, draw opacity=1, text opacity=1, draw=white!80!black},
minor xtick={25, 75},
minor ytick={},
tick align=outside,
tick pos=left,
width=\figwidth,
x grid style={white!69.0196078431373!black},
xlabel={Eval. Steps},
xminorgrids,
xmajorgrids,
xmin=-3.95, xmax=104.95,
xtick style={color=black},
xtick={-25,0,50,100,125},
xticklabels={-25,0,50,100,125},
y grid style={white!69.0196078431373!black},
ymajorgrids,
ymin=0.86, ymax=0.96,
ytick style={color=black},
ytick={0.86,0.88,0.9,0.92,0.94,0.96},
yticklabels={86,88,90,92,94,96}
]
\addplot [semithick, color0]
table {%
1 0.896765355269114
2 0.894921326637268
3 0.894921326637268
4 0.894921326637268
5 0.903399686018626
6 0.906071809927622
7 0.912411081790924
8 0.917821955680847
9 0.925969870885213
10 0.906071809927622
11 0.917367764314016
12 0.904689220587413
13 0.917367764314016
14 0.893567522366842
15 0.892513020833333
16 0.91672381957372
17 0.898092579841614
18 0.890482870737712
19 0.898092579841614
20 0.913631820678711
21 0.929171061515808
22 0.913631820678711
23 0.898092579841614
24 0.898092579841614
25 0.913631820678711
26 0.913631820678711
27 0.898092579841614
28 0.898092579841614
29 0.898092579841614
30 0.898092579841614
31 0.898584715525309
32 0.898092579841614
33 0.898092579841614
34 0.898092579841614
35 0.898584715525309
36 0.898584715525309
37 0.898584715525309
38 0.899076851209005
39 0.899076851209005
40 0.899076851209005
41 0.899076851209005
42 0.898584715525309
43 0.899076851209005
44 0.8995689868927
45 0.899076851209005
46 0.899076851209005
47 0.898584715525309
48 0.881827569007874
49 0.889714006582896
50 0.881335433324178
51 0.881335433324178
52 0.881335433324178
53 0.890698277950287
54 0.881827569007874
55 0.87295686006546
56 0.890721388657888
57 0.87295686006546
58 0.876064987977346
59 0.88495880762736
60 0.881850679715474
61 0.88495880762736
62 0.87295686006546
63 0.881850679715474
64 0.881850679715474
65 0.881850679715474
66 0.87295686006546
67 0.87295686006546
68 0.87295686006546
69 0.87295686006546
70 0.87295686006546
71 0.881850679715474
72 0.881850679715474
73 0.87295686006546
74 0.881850679715474
75 0.881850679715474
76 0.881850679715474
77 0.881850679715474
78 0.881850679715474
79 0.881850679715474
80 0.881850679715474
81 0.87295686006546
82 0.890744499365489
83 0.881850679715474
84 0.897418832778931
85 0.888525013128917
86 0.881850679715474
87 0.881850679715474
88 0.890744499365489
89 0.881850679715474
90 0.881850679715474
91 0.881850679715474
92 0.910753818353017
93 0.881850679715474
94 0.890744499365489
95 0.910753818353017
96 0.910753818353017
97 0.897418832778931
98 0.908534332116445
99 0.917428151766459
100 0.910753818353017
};
%\addlegendentry{a2c, gae, envs=10, lr=0.0001, act=tanh}
\addplot [semithick, color1]
table {%
1 0.921480818589528
2 0.935147138436635
3 0.920640448729197
4 0.93584371805191
5 0.938798908392588
6 0.950426689783732
7 0.93047868013382
8 0.938684165477753
9 0.93298856417338
10 0.942491340637207
11 0.938083600997925
12 0.949347658952077
13 0.937293823560079
14 0.932733265558879
15 0.923964134852092
16 0.946110077699025
17 0.931890956560771
18 0.934519072373708
19 0.932322569688161
20 0.933503027757009
21 0.929636486371358
22 0.939193348089854
23 0.934011054039001
24 0.932698806126912
25 0.94049733877182
26 0.925894375642141
27 0.921403002738953
28 0.932791344324748
29 0.933933361371358
30 0.927562729517619
31 0.937888709704081
32 0.920600946744283
33 0.938136263688405
34 0.899996622403463
35 0.912926848729451
36 0.928985595703125
37 0.940373949209849
38 0.937859932581584
39 0.942313873767853
40 0.937640762329102
41 0.930248153209686
42 0.913606786727905
43 0.935721615950266
44 0.935050336519877
45 0.930439297358195
46 0.937542017300924
47 0.918103329340617
48 0.897861814498901
49 0.926783275604248
50 0.907383171717326
51 0.909225769837697
52 0.942691270510356
53 0.933572089672089
54 0.939028263092041
55 0.940800519784291
56 0.939861921469371
57 0.913835887114207
58 0.906464064121246
59 0.935820357004801
60 0.908855724334717
61 0.933304270108541
62 0.936751465002696
63 0.934923716386159
64 0.931359966595968
65 0.911879702409109
66 0.915474430720011
67 0.915474430720011
68 0.908855724334717
69 0.911879702409109
70 0.933412305514018
71 0.93657025496165
72 0.92080721060435
73 0.925509091218312
74 0.925509091218312
75 0.932577860355377
76 0.931575111548106
77 0.934081399440765
78 0.914847405751546
79 0.895011293888092
80 0.937535949548086
81 0.933331366380056
82 0.920738403002421
83 0.917576460043589
84 0.915250742435455
85 0.922635873158773
86 0.940002608299255
87 0.937019153436025
88 0.937215872605642
89 0.941721439361572
90 0.902065221468608
91 0.929928580919901
92 0.941261808077494
93 0.919952885309855
94 0.938575609525045
95 0.938800060749054
96 0.936749017238617
97 0.929316782951355
98 0.939537576834361
99 0.938596649964651
100 0.940555159250895
};
%\addlegendentry{DQN, n train envs=30}
\addplot [semithick, color2]
table {%
1 0.902341936589183
100 0.902341936589183
};
%\addlegendentry{Random}
\addplot [semithick, color3]
table {%
1 0.919890937296078
100 0.919890937296078
};
%\addlegendentry{ETS}
\addplot [semithick, color4]
table {%
1 0.915537550984307
100 0.915537550984307
};
%\addlegendentry{Heur-GD}
\addplot [semithick, color5, dash pattern=on 1pt off 3pt on 3pt off 3pt]
table {%
1 0.870281256890804
100 0.870281256890804
};
%\addlegendentry{Heur-LD}
\addplot [semithick, color6, dashed]
table {%
1 0.915537550984307
100 0.915537550984307
};
%\addlegendentry{Heur-AT}
