# Supplementary material for: Learn the Time to Learn: Replay Scheduling in Continual Learning
Source: arXiv:2209.08660 source file (2023-11-20)
Supplement: Supplementary file 58 [file rewards_env8.tex]

\nextgroupplot[title=Seed 7,
height=\figheight,
legend cell align={left},
legend style={
  fill opacity=0.8,
  draw opacity=1,
  text opacity=1,
  at={(0.5,0.09)},
  anchor=south,
  draw=white!80!black
},
minor xtick={25, 75},
minor ytick={},
tick align=outside,
tick pos=left,
width=\figwidth,
x grid style={white!69.0196078431373!black},
xlabel={Eval. Steps},
xminorgrids,
xmajorgrids,
xmin=-3.95, xmax=104.95,
xtick style={color=black},
xtick={-25,0,50,100,125},
xticklabels={-25,0,50,100,125},
y grid style={white!69.0196078431373!black},
ymajorgrids,
ymin=0.885420464722211, ymax=0.944487913067026,
ytick style={color=black},
ytick={0.88,0.89,0.9,0.91,0.92,0.93,0.94,0.95},
yticklabels={88,89,90,91,92,93,94,95}
]
\addplot [semithick, color0]
table {%
1 0.92578417857488
2 0.913716804981232
3 0.913716804981232
4 0.913716804981232
5 0.925796155134837
6 0.923675127824148
7 0.92083371480306
8 0.926712167263031
9 0.923458111286163
10 0.922236128648122
11 0.92083371480306
12 0.927341826756795
13 0.92083371480306
14 0.917130430539449
15 0.917760090033213
16 0.924087770779928
17 0.925669650236766
18 0.923997473716736
19 0.921193611621857
20 0.924703268210093
21 0.926554910341899
22 0.923083321253459
23 0.927469062805176
24 0.926801335811615
25 0.925219456354777
26 0.928136789798737
27 0.923367814222972
28 0.921785934766134
29 0.928136789798737
30 0.924563503265381
31 0.925887183348338
32 0.926801335811615
33 0.923367814222972
34 0.923225140571594
35 0.923367814222972
36 0.923367814222972
37 0.926658662160238
38 0.924833687146505
39 0.927341282367706
40 0.929592482248942
41 0.926373314857483
42 0.926373314857483
43 0.92651598850886
44 0.927198608716329
45 0.926373314857483
46 0.926373314857483
47 0.930824327468872
48 0.926373314857483
49 0.926373314857483
50 0.926373314857483
51 0.935686127344767
52 0.930862390995026
53 0.930862390995026
54 0.935313403606415
55 0.926373314857483
56 0.931197051207225
57 0.930862390995026
58 0.930862390995026
59 0.926373314857483
60 0.926373314857483
61 0.926373314857483
62 0.930862390995026
63 0.927865016460419
64 0.929356718063355
65 0.938786840438843
66 0.934335827827454
67 0.9342977643013
68 0.939802479743958
69 0.929846751689911
70 0.934335827827454
71 0.926373314857483
72 0.930862390995026
73 0.929846751689911
74 0.932354092597961
75 0.929846751689911
76 0.937771201133728
77 0.933320188522339
78 0.934335827827454
79 0.929846751689911
80 0.938824903964996
81 0.929846751689911
82 0.935313403606415
83 0.929846751689911
84 0.9342977643013
85 0.926373314857483
86 0.9342977643013
87 0.938786840438843
88 0.9342977643013
89 0.933320188522339
90 0.9342977643013
91 0.9342977643013
92 0.930824327468872
93 0.929846751689911
94 0.934335827827454
95 0.9342977643013
96 0.929846751689911
97 0.938748776912689
98 0.936793625354767
99 0.936845274766286
100 0.929846751689911
};
%\addlegendentry{a2c, gae, envs=10, lr=0.0001, act=tanh}
\addplot [semithick, color1]
table {%
1 0.922018905480703
2 0.93385188182195
3 0.933049762248993
4 0.937681969006856
5 0.923364698886871
6 0.932277429103851
7 0.926413504282633
8 0.929269806543986
9 0.919175859292348
10 0.926569151878357
11 0.909814258416494
12 0.928396105766296
13 0.92667064666748
14 0.927418152491252
15 0.927338369687398
16 0.924459314346313
17 0.914904852708181
18 0.930903911590576
19 0.934333777427673
20 0.929718132813771
21 0.932110798358917
22 0.926157573858897
23 0.921757793426514
24 0.928022789955139
25 0.920009370644887
26 0.92337947289149
27 0.933102718989054
28 0.930000944932302
29 0.934517109394074
30 0.92908806403478
31 0.931301661332448
32 0.930003949006398
33 0.929051729043325
34 0.931829039255778
35 0.924023560682933
36 0.927264149983724
37 0.933500679334005
38 0.930545163154602
39 0.93114980061849
40 0.912345822652181
41 0.926198760668437
42 0.933579409122467
43 0.928345727920532
44 0.931149593989054
45 0.93114980061849
46 0.931033209959666
47 0.924755167961121
48 0.934453276793162
49 0.929902791976929
50 0.931149593989054
51 0.93549599647522
52 0.930313583215078
53 0.931882210572561
54 0.93435199658076
55 0.928255434830983
56 0.934866336981455
57 0.93549599647522
58 0.930133573214213
59 0.935314667224884
60 0.92856494585673
61 0.935752340157827
62 0.934866336981455
63 0.937139431635539
64 0.934260173638662
65 0.930262144406637
66 0.934158484141032
67 0.931149593989054
68 0.928989958763123
69 0.935687983036041
70 0.934633282820384
71 0.93312980333964
72 0.933797272046407
73 0.930285231272379
74 0.93616425593694
75 0.932268770535787
76 0.928563805421193
77 0.930042135715485
78 0.925259788831075
79 0.932910207907359
80 0.932909417152405
81 0.931792497634888
82 0.929374611377716
83 0.929373343785604
84 0.935108109315236
85 0.935006419817607
86 0.932923253377279
87 0.933126425743103
88 0.927960435549418
89 0.932073990503947
90 0.933425815900167
91 0.932073990503947
92 0.93155779838562
93 0.93155779838562
94 0.93155779838562
95 0.932909417152405
96 0.933772456645966
97 0.933425815900167
98 0.929964407285054
99 0.929989171028137
100 0.93405255873998
};
%\addlegendentry{DQN, n train envs=30}
\addplot [semithick, color2]
table {%
1 0.941803029051352
100 0.941803029051352
};
%\addlegendentry{Random}
\addplot [semithick, color3]
table {%
1 0.94031006304327
100 0.94031006304327
};
%\addlegendentry{ETS}
\addplot [semithick, color4]
table {%
1 0.888105348737885
100 0.888105348737885
};
%\addlegendentry{Heur-GD}
\addplot [semithick, color5, dash pattern=on 1pt off 3pt on 3pt off 3pt]
table {%
1 0.906470737356177
100 0.906470737356177
};
%\addlegendentry{Heur-LD}
\addplot [semithick, color6, dashed]
table {%
1 0.93077412279482
100 0.93077412279482
};
%\addlegendentry{Heur-AT}
