# Supplementary material for: Learn the Time to Learn: Replay Scheduling in Continual Learning
Source: arXiv:2209.08660 source file (2023-11-20)
Supplement: Supplementary file 59 [file rewards_env9.tex]

\nextgroupplot[title=Seed 8,
height=\figheight,
legend cell align={left},
legend style={
  fill opacity=0.8,
  draw opacity=1,
  text opacity=1,
  at={(0.5,0.09)},
  anchor=south,
  draw=white!80!black
},
minor xtick={25, 75},
minor ytick={},
tick align=outside,
tick pos=left,
width=\figwidth,
x grid style={white!69.0196078431373!black},
xlabel={Eval. Steps},
xminorgrids,
xmajorgrids,
xmin=-3.95, xmax=104.95,
xtick style={color=black},
xtick={-25,0,50,100,125},
xticklabels={-25,0,50,100,125},
y grid style={white!69.0196078431373!black},
ylabel={ACC (\%)},
ymajorgrids,
ymin=0.87912724410805, ymax=0.945090560499017,
ytick style={color=black},
ytick={0.87,0.88,0.89,0.9,0.91,0.92,0.93,0.94,0.95},
yticklabels={87,88,89,90,91,92,93,94,95}
]
\addplot [semithick, color0]
table {%
1 0.932959767182668
2 0.9315957903862
3 0.9315957903862
4 0.9315957903862
5 0.929590439796448
6 0.922864870230357
7 0.920010852813721
8 0.926947601636251
9 0.921921781698863
10 0.922864870230357
11 0.920010852813721
12 0.928529818852743
13 0.920010852813721
14 0.917199921607971
15 0.91954847574234
16 0.92719247341156
17 0.925871590773265
18 0.923213362693787
19 0.923213362693787
20 0.926513294378916
21 0.927834177017212
22 0.930987938245138
23 0.925192411740621
24 0.925748900572459
25 0.927069783210754
26 0.926513294378916
27 0.925748900572459
28 0.924147645632426
29 0.932865309715271
30 0.927069783210754
31 0.931189453601837
32 0.927626272042592
33 0.927626272042592
34 0.933421798547109
35 0.927292303244273
36 0.927851009368897
37 0.926682889461517
38 0.926761345068614
39 0.925616447130839
40 0.922710601488749
41 0.928392314910889
42 0.925537991523743
43 0.932428169250488
44 0.928470770517985
45 0.932959127426147
46 0.928392314910889
47 0.933311065038045
48 0.937698856989543
49 0.931516695022583
50 0.937698856989543
51 0.934844533602397
52 0.931516695022583
53 0.936165388425191
54 0.937698856989543
55 0.933035643895467
56 0.937698856989543
57 0.93590448697408
58 0.939232325553894
59 0.939232325553894
60 0.93590448697408
61 0.93590448697408
62 0.939232325553894
63 0.939232325553894
64 0.939232325553894
65 0.93590448697408
66 0.939232325553894
67 0.93590448697408
68 0.939232325553894
69 0.93590448697408
70 0.939232325553894
71 0.939232325553894
72 0.939232325553894
73 0.939232325553894
74 0.93590448697408
75 0.93590448697408
76 0.939232325553894
77 0.93590448697408
78 0.93590448697408
79 0.939232325553894
80 0.93590448697408
81 0.939232325553894
82 0.932576648394267
83 0.932576648394267
84 0.93590448697408
85 0.939232325553894
86 0.932576648394267
87 0.939232325553894
88 0.932576648394267
89 0.93590448697408
90 0.93590448697408
91 0.939232325553894
92 0.932576648394267
93 0.93590448697408
94 0.93590448697408
95 0.929248809814453
96 0.932576648394267
97 0.93590448697408
98 0.939232325553894
99 0.9348570783933
100 0.939232325553894
};
%\addlegendentry{a2c, gae, envs=10, lr=0.0001, act=tanh}
\addplot [semithick, color1]
table {%
1 0.932049596309662
2 0.941636677583059
3 0.934989941120148
4 0.921661857763926
5 0.930970370769501
6 0.930268514156341
7 0.935579820473989
8 0.931672505537669
9 0.922811106840769
10 0.923790995279948
11 0.927957705656687
12 0.933957719802856
13 0.926543176174164
14 0.936040687561035
15 0.932267272472382
16 0.926834412415822
17 0.93060261408488
18 0.929786193370819
19 0.939294250806173
20 0.936575829982758
21 0.936856269836426
22 0.938313861687978
23 0.93715136051178
24 0.942092227935791
25 0.938181002934774
26 0.931000852584839
27 0.929074800014496
28 0.920625591278076
29 0.926675526301066
30 0.928688132762909
31 0.927901291847229
32 0.927641900380452
33 0.938032786051432
34 0.925219917297363
35 0.938511923948924
36 0.927879174550374
37 0.935892975330353
38 0.938010668754578
39 0.927901291847229
40 0.930322178204854
41 0.927901291847229
42 0.929819822311401
43 0.942092227935791
44 0.923540131251017
45 0.927879174550374
46 0.93443036476771
47 0.927879174550374
48 0.933671625455221
49 0.933671625455221
50 0.936981530984243
51 0.941434061527252
52 0.936981530984243
53 0.931788198153178
54 0.934452482064565
55 0.932146255175273
56 0.937352502346039
57 0.933951226870219
58 0.931788198153178
59 0.931960733731588
60 0.938010668754578
61 0.931302567323049
62 0.935870858033498
63 0.931302567323049
64 0.933401230971019
65 0.931459482510885
66 0.939952417214712
67 0.936575829982758
68 0.93447459936142
69 0.925738263130188
70 0.931960733731588
71 0.931960733731588
72 0.933902482191722
73 0.921810984611511
74 0.929820923010508
75 0.925910798708598
76 0.931960733731588
77 0.935870858033498
78 0.938010668754578
79 0.935870858033498
80 0.937316373984019
81 0.931960733731588
82 0.927621690432231
83 0.930005343755086
84 0.940824639797211
85 0.933244315783183
86 0.921071171760559
87 0.924524704615275
88 0.927571841080983
89 0.927621690432231
90 0.91920108795166
91 0.922336483001709
92 0.929489497343699
93 0.923298939069112
94 0.921399219830831
95 0.928038068612417
96 0.933508288860321
97 0.926905278364817
98 0.935325880845388
99 0.925916190942128
100 0.927621690432231
};
%\addlegendentry{DQN, n train envs=30}
\addplot [semithick, color2]
table {%
1 0.924340868446401
100 0.924340868446401
};
%\addlegendentry{Random}
\addplot [semithick, color3]
table {%
1 0.890415249936047
100 0.890415249936047
};
%\addlegendentry{ETS}
\addplot [semithick, color4]
table {%
1 0.935567569236973
100 0.935567569236973
};
%\addlegendentry{Heur-GD}
\addplot [semithick, color5, dash pattern=on 1pt off 3pt on 3pt off 3pt]
table {%
1 0.882125576671276
100 0.882125576671276
};
%\addlegendentry{Heur-LD}
\addplot [semithick, color6, dashed]
table {%
1 0.935567569236973
100 0.935567569236973
};
%\addlegendentry{Heur-AT}
