# Supplementary material for: Learn the Time to Learn: Replay Scheduling in Continual Learning
Source: arXiv:2209.08660 source file (2023-11-20)
Supplement: Supplementary file 60 [file fashionmnist_new_dataset.tex]

\begin{tabular}{lcccccccccc}
\toprule
                 & \multicolumn{2}{c}{\textbf{Test Env. Seed 0}} & \multicolumn{2}{c}{\textbf{Test Env. Seed 1}} & \multicolumn{2}{c}{\textbf{Test Env. Seed 2}} & \multicolumn{2}{c}{\textbf{Test Env. Seed 3}} & \multicolumn{2}{c}{\textbf{Test Env. Seed 4}} \\
\cmidrule(lr){2-3} \cmidrule(lr){4-5} \cmidrule(lr){6-7} \cmidrule(lr){8-9} \cmidrule(lr){10-11}
\textbf{Methods} & $t$                   & $p$                     & $t$                   & $p$                     & $t$                   & $p$                     & $t$                   & $p$                     & $t$                   & $p$                     \\
\midrule
DQN vs Random   & 1.47      & 0.193             & 0.69      & 0.515             & 1.53      & 0.187             & 0.17      & 0.872             & 1.46      & 0.184             \\
DQN vs ETS      & -0.38     & 0.725             & -0.38     & 0.720             & 19.36     & \textbf{0.000}    & 2.09      & 0.105             & 0.72      & 0.513             \\
DQN vs Heur-GD  & -1.45     & 0.222             & -1.36     & 0.245             & -2.63     & 0.058             & -0.81     & 0.463             & -1.07     & 0.345             \\
DQN vs Heur-LD: & -1.03     & 0.360             & 3.98      & 0.016             & -2.40     & 0.074             & 1.62      & 0.181             & 0.85      & 0.442             \\
DQN vs Heur-AT  & -0.79     & 0.473             & -0.37     & 0.728             & -3.12     & \textbf{0.035}    & -1.90     & 0.131             & 2.32      & 0.081             \\
DQN vs A2C      & 0.59      & 0.579             & 0.77      & 0.462             & -2.11     & 0.076             & 0.81      & 0.442             & -1.36     & 0.245             \\
\midrule
A2C vs Random   & 0.63      & 0.547             & 0.26      & 0.804             & 2.37      & 0.073             & -0.72     & 0.495             & 3.19      & \textbf{0.033}    \\
A2C vs ETS      & -0.82     & 0.461             & -1.67     & 0.171             & 38.38     & \textbf{0.000}    & 1.43      & 0.226             & 57.27     & \textbf{0.000}    \\
A2C vs Heur-GD  & -1.30     & 0.265             & -2.84     & \textbf{0.047}    & -0.35     & 0.746             & -2.44     & 0.072             & 8.05      & \textbf{0.001}    \\
A2C vs Heur-LD  & -1.11     & 0.329             & 3.56      & \textbf{0.024}    & 0.05      & 0.962             & 0.81      & 0.465             & 61.00     & \textbf{0.000}    \\
A2C vs Heur-AT  & -1.00     & 0.373             & -1.65     & 0.173             & -1.22     & 0.290             & -3.88     & 0.018             & 101.48    & \textbf{0.000}    \\
A2C vs DQN      & -0.59     & 0.579             & -0.77     & 0.462             & 2.11      & 0.076             & -0.81     & 0.442             & 1.36      & 0.245             \\
\midrule
                & \multicolumn{2}{c}{Test Env. Seed 5} & \multicolumn{2}{c}{Test Env. Seed 6} & \multicolumn{2}{c}{Test Env. Seed 7} & \multicolumn{2}{c}{Test Env. Seed 8} & \multicolumn{2}{c}{Test Env. Seed 9} \\
\cmidrule(lr){2-3} \cmidrule(lr){4-5} \cmidrule(lr){6-7} \cmidrule(lr){8-9} \cmidrule(lr){10-11}
Methods         & $t$          & $p$                     & $t$          & $p$                     & $t$          & $p$                     & $t$          & $p$                     & $t$          & $p$                     \\
\midrule
DQN vs Random   & -1.82     & 0.122             & -2.93     & \textbf{0.041}    & -4.21     & \textbf{0.009}    & -0.59     & 0.570             & 0.25      & 0.812             \\
DQN vs ETS      & -7.73     & \textbf{0.002}    & -3.00     & \textbf{0.040}    & -5.20     & \textbf{0.007}    & -2.20     & 0.093             & -1.58     & 0.189             \\
DQN vs Heur-GD  & -5.53     & \textbf{0.005}    & -1.15     & 0.313             & -2.17     & 0.096             & -2.34     & 0.079             & 0.05      & 0.961             \\
DQN vs Heur-LD: & -1.28     & 0.269             & 0.39      & 0.714             & -5.06     & \textbf{0.007}    & 2.67      & 0.056             & 6.00      & \textbf{0.004}    \\
DQN vs Heur-AT  & -5.90     & \textbf{0.004}    & 3.58      & \textbf{0.023}    & -6.46     & \textbf{0.003}    & -1.59     & 0.187             & 5.70      & \textbf{0.005}    \\
DQN vs A2C      & -1.14     & 0.320             & -0.73     & 0.490             & -2.45     & \textbf{0.040}    & -1.34     & 0.253             & 3.87      & \textbf{0.007}    \\
\midrule
A2C vs Random   & -1.49     & 0.210             & -3.32     & \textbf{0.026}    & -0.68     & 0.529             & 0.21      & 0.846             & -1.84     & 0.129             \\
A2C vs ETS      & -inf      & \textbf{0.000}    & -3.47     & \textbf{0.026}    & -1.41     & 0.231             & -inf      & \textbf{0.000}    & -10.02    & \textbf{0.001}    \\
A2C vs Heur-GD  & -inf      & \textbf{0.000}    & -0.47     & 0.660             & 1.34      & 0.252             & -inf      & \textbf{0.000}    & -7.35     & \textbf{0.002}    \\
A2C vs Heur-LD  & -inf      & \textbf{0.000}    & 2.03      & 0.113             & -1.28     & 0.270             & inf       & \textbf{0.000}    & 2.39      & 0.075             \\
A2C vs Heur-AT  & -inf      & \textbf{0.000}    & 7.18      & \textbf{0.002}    & -2.55     & 0.063             & -inf      & \textbf{0.000}    & 1.89      & 0.131             \\
A2C vs DQN      & 1.14      & 0.320             & 0.73      & 0.490             & 2.45      & \textbf{0.040}    & 1.34      & 0.253             & -3.87     & \textbf{0.007}   \\
\bottomrule
\end{tabular}
